# Supplementary material for: Sharper Bounds for the Chebyshev function $\theta(x)$
Source: arXiv:2002.11068 ancillary file (2021-01-27)
Supplement: Supplementary file 1 [file Full-Tables-Sharper-Bounds-June-2020.pdf]

# TABLES OF VALUES OF THE CHEBYSHEV FUNCTIONS $\theta(x)$ AND $\psi(x)$

SAMUEL BROADBENT, ANDREW FIORI, HABIBA KADIRI, ALLYSA LUMLEY, NATHAN NG, JOSHUA SWIDINSKY, KIRSTEN WILK

**ABSTRACT.** In these tables, we provide explicit bounds for the prime counting functions (Chebyshev functions)  $\theta(x)$  and  $\psi(x)$  in all ranges of  $x$ . The bounds for the error terms  $\psi(x) - x$  and  $\theta(x) - x$  are of the shape  $\varepsilon x$  and  $\frac{c_k x}{(\log x)^k}$ , for  $k = 0, \dots, 5$ . Tables of values for  $\varepsilon$  and  $c_k$  are provided.

## 1. INTRODUCTION

These tables provide explicit values for the prime counting functions (Chebyshev functions)

$$\theta(x) = \sum_{p \leq x} \log p, \text{ and } \psi(x) = \sum_{p^k \leq x, k \geq 1} \log p$$

where  $p$  ranges through prime numbers. This file complements the article [1]. In [1] the following theorem for  $\theta(x)$  is established:

**Theorem 1.** *Let  $k$  be an integer with  $0 \leq k \leq 5$ . For any fixed  $X_0 \geq 1$ , there exists  $m_k > 0$  such that, for all  $x \geq X_0$*

$$(1.1) \quad x \left( 1 - \frac{m_k}{(\log x)^k} \right) \leq \theta(x).$$

*For any fixed  $X_1 \geq 1$ , there exists  $M_k > 0$  such that, for all  $x \geq X_1$*

$$(1.2) \quad \theta(x) \leq x \left( 1 + \frac{M_k}{(\log x)^k} \right).$$

In addition, we established bounds for  $\psi(x) - x$  based on the work of Büthe [2], [3] and Platt-Trudgian [7].

**Theorem 2.** *Let  $b > 0$ . Then there exists a positive constant  $\varepsilon(b)$  such that*

$$(1.3) \quad \left| \frac{\psi(x) - x}{x} \right| \leq \varepsilon(b), \text{ for all } x \geq e^b.$$

Tables 8-15 which follow give a variety of bounds for  $\theta(x)$  and  $\psi(x)$ , in various ranges of  $x$ . In particular, Tables 14 and 15 give values for  $m_k$  and  $M_k$  in Theorem 1 and Table 8 gives values for  $\varepsilon(b)$  in Theorem 2. The values for some of these constants improve on and also extend previous values given in a number of articles including [9], [10], [4], [6], [2], [5], and [7]. Further details and a comprehensive history of such bounds may be found in [1]. The numbering of these tables is so that they match up with the companion article [1]. In [1], Appendix B contains abbreviated versions of Tables 8-15 that appear in this file. The various bounds for  $\theta(x)$  and  $\psi(x)$  are based on the arguments from [1] and the reader should consult it for further details.

The bounds for  $\theta(x)$  were first done by Broadbent and Wilk (under the supervision of Kadiri and Ng). The calculations for  $|\psi(x) - x|$  were first computed using programs of Kadiri and Lumley. Using different programs, both calculations for  $\theta$  and  $\psi$  were then independently verified by Fiori

---

2000 *Mathematics Subject Classification.* 11N05, 11M06, 11M26.

*Key words and phrases.* prime number theorem,  $\psi(x)$ ,  $\theta(x)$ , explicit formula, zeros of Riemann zeta function.

and then by Swidinsky (under the supervision of Fiori and Kadiri). These calculations were done on the University of Lethbridge Number Theory Group Eudoxus machine, supported by an NSERC RTI grant.

2. TABLE 8: SHARPER BOUNDS FOR  $\psi(x) - |\psi(x) - x| < \varepsilon(b)x$  WHERE  $\varepsilon(b)$  IS COMPUTABLE FOR  $x \geq e^b$  FIXED

TABLE 8. Combined table of sharpest bounds for  $|\psi(x) - x| < \varepsilon x$ . Computed using Wedeniwski's partial verification of the Riemann Hypothesis ( $H_0 = 2\,445\,999\,556\,030$  [11]). For all  $x \geq x_0 = e^b$  we have  $|\psi(x) - x| < \varepsilon(b)x$ .

| $b$                           | $\varepsilon(b)$        |
|-------------------------------|-------------------------|
| Computed as in [2, Theorem 1] |                         |
| 20                            | $4.2677 \cdot 10^{-5}$  |
| 21                            | $2.5885 \cdot 10^{-5}$  |
| 22                            | $1.5701 \cdot 10^{-5}$  |
| 23                            | $9.5224 \cdot 10^{-6}$  |
| 24                            | $5.7757 \cdot 10^{-6}$  |
| 25                            | $3.5032 \cdot 10^{-6}$  |
| 26                            | $2.1248 \cdot 10^{-6}$  |
| 27                            | $1.2888 \cdot 10^{-6}$  |
| 28                            | $7.8165 \cdot 10^{-7}$  |
| 29                            | $4.7410 \cdot 10^{-7}$  |
| 30                            | $2.8756 \cdot 10^{-7}$  |
| 31                            | $1.7442 \cdot 10^{-7}$  |
| 32                            | $1.0579 \cdot 10^{-7}$  |
| 33                            | $6.4162 \cdot 10^{-8}$  |
| 34                            | $3.8917 \cdot 10^{-8}$  |
| 35                            | $2.3604 \cdot 10^{-8}$  |
| 36                            | $1.9339 \cdot 10^{-8}$  |
| 37                            | $1.9339 \cdot 10^{-8}$  |
| 38                            | $1.9339 \cdot 10^{-8}$  |
| 39                            | $1.9339 \cdot 10^{-8}$  |
| 40                            | $1.9339 \cdot 10^{-8}$  |
| 41                            | $1.9339 \cdot 10^{-8}$  |
| 42                            | $1.9338 \cdot 10^{-8}$  |
| 43                            | $1.9339 \cdot 10^{-8}$  |
| 44                            | $1.7201 \cdot 10^{-8}$  |
| 45                            | $1.0908 \cdot 10^{-8}$  |
| 46                            | $6.9452 \cdot 10^{-9}$  |
| 47                            | $4.4013 \cdot 10^{-9}$  |
| 48                            | $2.7915 \cdot 10^{-9}$  |
| 49                            | $1.7690 \cdot 10^{-9}$  |
| 50                            | $1.1200 \cdot 10^{-9}$  |
| 51                            | $7.0925 \cdot 10^{-10}$ |
| 52                            | $4.4782 \cdot 10^{-10}$ |
| 53                            | $2.8281 \cdot 10^{-10}$ |
| 54                            | $1.7847 \cdot 10^{-10}$ |
| 55                            | $1.1256 \cdot 10^{-10}$ |
| 56                            | $7.0929 \cdot 10^{-11}$ |
| 57                            | $4.4656 \cdot 10^{-11}$ |
| 58                            | $2.8329 \cdot 10^{-11}$ |
| 59                            | $1.8441 \cdot 10^{-11}$ |
| 60                            | $1.2216 \cdot 10^{-11}$ |
| Continued on next page        |                         |

Table 8 – continued from previous page

| $b$                             | $\varepsilon(b)$        |
|---------------------------------|-------------------------|
| 65                              | $3.5713 \cdot 10^{-12}$ |
| 70                              | $2.7924 \cdot 10^{-12}$ |
| 75                              | $2.7037 \cdot 10^{-12}$ |
| 80                              | $2.6109 \cdot 10^{-12}$ |
| 85                              | $2.5693 \cdot 10^{-12}$ |
| 90                              | $2.5214 \cdot 10^{-12}$ |
| 95                              | $2.4920 \cdot 10^{-12}$ |
| 100                             | $2.4531 \cdot 10^{-12}$ |
| 200                             | $2.1816 \cdot 10^{-12}$ |
| 300                             | $2.0903 \cdot 10^{-12}$ |
| 400                             | $2.0399 \cdot 10^{-12}$ |
| 500                             | $2.0000 \cdot 10^{-12}$ |
| 600                             | $1.9890 \cdot 10^{-12}$ |
| 700                             | $1.9765 \cdot 10^{-12}$ |
| 800                             | $1.9672 \cdot 10^{-12}$ |
| 900                             | $1.9600 \cdot 10^{-12}$ |
| 1000                            | $1.9476 \cdot 10^{-12}$ |
| 1500                            | $1.9369 \cdot 10^{-12}$ |
| 1600                            | $1.9293 \cdot 10^{-12}$ |
| 1700                            | $1.9274 \cdot 10^{-12}$ |
| 1725                            | $1.9270 \cdot 10^{-12}$ |
| 1750                            | $1.9266 \cdot 10^{-12}$ |
| 1775                            | $1.9261 \cdot 10^{-12}$ |
| 1800                            | $1.9257 \cdot 10^{-12}$ |
| 1825                            | $1.9254 \cdot 10^{-12}$ |
| 1850                            | $1.9250 \cdot 10^{-12}$ |
| 1875                            | $1.9246 \cdot 10^{-12}$ |
| 1900                            | $1.9242 \cdot 10^{-12}$ |
| 1925                            | $1.9239 \cdot 10^{-12}$ |
| 1950                            | $1.9235 \cdot 10^{-12}$ |
| 1975                            | $1.9232 \cdot 10^{-12}$ |
| 2000                            | $1.9229 \cdot 10^{-12}$ |
| 2025                            | $1.9225 \cdot 10^{-12}$ |
| 2050                            | $1.9222 \cdot 10^{-12}$ |
| 2075                            | $1.9219 \cdot 10^{-12}$ |
| 2100                            | $1.9217 \cdot 10^{-12}$ |
| 2125                            | $1.9214 \cdot 10^{-12}$ |
| 2150                            | $1.9211 \cdot 10^{-12}$ |
| 2175                            | $1.9208 \cdot 10^{-12}$ |
| 2200                            | $1.9206 \cdot 10^{-12}$ |
| 2225                            | $1.9203 \cdot 10^{-12}$ |
| 2250                            | $1.9200 \cdot 10^{-12}$ |
| 2275                            | $1.9198 \cdot 10^{-12}$ |
| 2300                            | $1.9195 \cdot 10^{-12}$ |
| 2325                            | $1.8751 \cdot 10^{-12}$ |
| 2350                            | $1.7788 \cdot 10^{-12}$ |
| 2375                            | $1.6875 \cdot 10^{-12}$ |
| 2400                            | $1.6009 \cdot 10^{-12}$ |
| Computed using [1, Theorem 13 ] |                         |
| 2425                            | $1.4218 \cdot 10^{-12}$ |
| 2450                            | $1.2214 \cdot 10^{-12}$ |
| 2475                            | $1.0512 \cdot 10^{-12}$ |
| 2500                            | $9.0631 \cdot 10^{-13}$ |
| 2525                            | $7.7933 \cdot 10^{-13}$ |
| Continued on next page          |                         |

Table 8 – continued from previous page

| $b$                    | $\varepsilon(b)$        |
|------------------------|-------------------------|
| 2550                   | $6.7069 \cdot 10^{-13}$ |
| 2575                   | $5.7662 \cdot 10^{-13}$ |
| 2600                   | $4.9610 \cdot 10^{-13}$ |
| 2625                   | $4.2694 \cdot 10^{-13}$ |
| 2650                   | $3.6747 \cdot 10^{-13}$ |
| 2675                   | $3.1642 \cdot 10^{-13}$ |
| 2700                   | $2.7243 \cdot 10^{-13}$ |
| 2725                   | $2.3455 \cdot 10^{-13}$ |
| 2750                   | $2.0207 \cdot 10^{-13}$ |
| 2775                   | $1.7404 \cdot 10^{-13}$ |
| 2800                   | $1.5006 \cdot 10^{-13}$ |
| 2825                   | $1.2952 \cdot 10^{-13}$ |
| 2850                   | $1.1190 \cdot 10^{-13}$ |
| 2875                   | $9.6389 \cdot 10^{-14}$ |
| 2900                   | $8.3167 \cdot 10^{-14}$ |
| 2925                   | $7.1662 \cdot 10^{-14}$ |
| 2950                   | $6.1818 \cdot 10^{-14}$ |
| 2975                   | $5.3383 \cdot 10^{-14}$ |
| 3000                   | $4.5998 \cdot 10^{-14}$ |
| 3025                   | $3.9721 \cdot 10^{-14}$ |
| 3050                   | $3.4247 \cdot 10^{-14}$ |
| 3075                   | $2.9576 \cdot 10^{-14}$ |
| 3100                   | $2.5535 \cdot 10^{-14}$ |
| 3125                   | $2.2031 \cdot 10^{-14}$ |
| 3150                   | $1.9028 \cdot 10^{-14}$ |
| 3175                   | $1.6430 \cdot 10^{-14}$ |
| 3200                   | $1.4197 \cdot 10^{-14}$ |
| 3225                   | $1.2278 \cdot 10^{-14}$ |
| 3250                   | $1.0627 \cdot 10^{-14}$ |
| 3275                   | $9.1915 \cdot 10^{-15}$ |
| 3300                   | $7.9435 \cdot 10^{-15}$ |
| 3325                   | $6.8702 \cdot 10^{-15}$ |
| 3350                   | $5.9387 \cdot 10^{-15}$ |
| 3375                   | $5.1333 \cdot 10^{-15}$ |
| 3400                   | $4.4414 \cdot 10^{-15}$ |
| 3425                   | $3.8454 \cdot 10^{-15}$ |
| 3450                   | $3.3251 \cdot 10^{-15}$ |
| 3475                   | $2.8741 \cdot 10^{-15}$ |
| 3500                   | $2.4865 \cdot 10^{-15}$ |
| 3525                   | $2.1523 \cdot 10^{-15}$ |
| 3550                   | $1.8633 \cdot 10^{-15}$ |
| 3575                   | $1.6124 \cdot 10^{-15}$ |
| 3600                   | $1.3966 \cdot 10^{-15}$ |
| 3625                   | $1.2101 \cdot 10^{-15}$ |
| 3650                   | $1.0470 \cdot 10^{-15}$ |
| 3675                   | $9.0704 \cdot 10^{-16}$ |
| 3700                   | $7.8647 \cdot 10^{-16}$ |
| 3725                   | $6.8213 \cdot 10^{-16}$ |
| 3750                   | $5.9196 \cdot 10^{-16}$ |
| 3775                   | $5.1352 \cdot 10^{-16}$ |
| 3800                   | $4.4496 \cdot 10^{-16}$ |
| 3825                   | $3.8583 \cdot 10^{-16}$ |
| 3850                   | $3.3477 \cdot 10^{-16}$ |
| 3875                   | $2.9011 \cdot 10^{-16}$ |
| Continued on next page |                         |

Table 8 – continued from previous page

| $b$                    | $\varepsilon(b)$        |
|------------------------|-------------------------|
| 3900                   | $2.5173 \cdot 10^{-16}$ |
| 3925                   | $2.1855 \cdot 10^{-16}$ |
| 3950                   | $1.8982 \cdot 10^{-16}$ |
| 3975                   | $1.6448 \cdot 10^{-16}$ |
| 4000                   | $1.4264 \cdot 10^{-16}$ |
| 4025                   | $1.2412 \cdot 10^{-16}$ |
| 4050                   | $1.0750 \cdot 10^{-16}$ |
| 4075                   | $9.3378 \cdot 10^{-17}$ |
| 4100                   | $8.1038 \cdot 10^{-17}$ |
| 4125                   | $7.0376 \cdot 10^{-17}$ |
| 4150                   | $6.1237 \cdot 10^{-17}$ |
| 4175                   | $5.3118 \cdot 10^{-17}$ |
| 4200                   | $4.6145 \cdot 10^{-17}$ |
| 4225                   | $4.0111 \cdot 10^{-17}$ |
| 4250                   | $3.4884 \cdot 10^{-17}$ |
| 4275                   | $3.0318 \cdot 10^{-17}$ |
| 4300                   | $2.6350 \cdot 10^{-17}$ |
| 4325                   | $2.2914 \cdot 10^{-17}$ |
| 4350                   | $1.9935 \cdot 10^{-17}$ |
| 4375                   | $1.7336 \cdot 10^{-17}$ |
| 4400                   | $1.5084 \cdot 10^{-17}$ |
| 4425                   | $1.3133 \cdot 10^{-17}$ |
| 4450                   | $1.1437 \cdot 10^{-17}$ |
| 4475                   | $9.9627 \cdot 10^{-18}$ |
| 4500                   | $8.6830 \cdot 10^{-18}$ |
| 4525                   | $7.5706 \cdot 10^{-18}$ |
| 4550                   | $6.5914 \cdot 10^{-18}$ |
| 4575                   | $5.7400 \cdot 10^{-18}$ |
| 4600                   | $5.0071 \cdot 10^{-18}$ |
| 4625                   | $4.3570 \cdot 10^{-18}$ |
| 4650                   | $3.7976 \cdot 10^{-18}$ |
| 4675                   | $3.3113 \cdot 10^{-18}$ |
| 4700                   | $2.8885 \cdot 10^{-18}$ |
| 4725                   | $2.5214 \cdot 10^{-18}$ |
| 4750                   | $2.1972 \cdot 10^{-18}$ |
| 4775                   | $1.9146 \cdot 10^{-18}$ |
| 4800                   | $1.6693 \cdot 10^{-18}$ |
| 4825                   | $1.4561 \cdot 10^{-18}$ |
| 4850                   | $1.2709 \cdot 10^{-18}$ |
| 4875                   | $1.1095 \cdot 10^{-18}$ |
| 4900                   | $9.6895 \cdot 10^{-19}$ |
| 4925                   | $8.4602 \cdot 10^{-19}$ |
| 4950                   | $7.3831 \cdot 10^{-19}$ |
| 4975                   | $6.4458 \cdot 10^{-19}$ |
| 5000                   | $5.6304 \cdot 10^{-19}$ |
| 5100                   | $3.2860 \cdot 10^{-19}$ |
| 5200                   | $1.9218 \cdot 10^{-19}$ |
| 5300                   | $1.1293 \cdot 10^{-19}$ |
| 5400                   | $6.6313 \cdot 10^{-20}$ |
| 5500                   | $3.9136 \cdot 10^{-20}$ |
| 5600                   | $2.3189 \cdot 10^{-20}$ |
| 5700                   | $1.3808 \cdot 10^{-20}$ |
| 5800                   | $8.2235 \cdot 10^{-21}$ |
| 5900                   | $4.9138 \cdot 10^{-21}$ |
| Continued on next page |                         |

Table 8 – continued from previous page

| $b$   | $\varepsilon(b)$        |
|-------|-------------------------|
| 6000  | $2.9430 \cdot 10^{-21}$ |
| 6100  | $1.7722 \cdot 10^{-21}$ |
| 6200  | $1.0664 \cdot 10^{-21}$ |
| 6300  | $6.4481 \cdot 10^{-22}$ |
| 6400  | $3.9202 \cdot 10^{-22}$ |
| 6500  | $2.3850 \cdot 10^{-22}$ |
| 6600  | $1.4521 \cdot 10^{-22}$ |
| 6700  | $8.8894 \cdot 10^{-23}$ |
| 6800  | $5.4568 \cdot 10^{-23}$ |
| 6900  | $3.3650 \cdot 10^{-23}$ |
| 7000  | $2.0766 \cdot 10^{-23}$ |
| 7100  | $1.2893 \cdot 10^{-23}$ |
| 7200  | $8.0276 \cdot 10^{-24}$ |
| 7300  | $5.0020 \cdot 10^{-24}$ |
| 7400  | $3.1319 \cdot 10^{-24}$ |
| 7500  | $1.9616 \cdot 10^{-24}$ |
| 7600  | $1.2315 \cdot 10^{-24}$ |
| 7700  | $7.7654 \cdot 10^{-25}$ |
| 7800  | $4.9129 \cdot 10^{-25}$ |
| 7900  | $3.1161 \cdot 10^{-25}$ |
| 8000  | $1.9762 \cdot 10^{-25}$ |
| 8100  | $1.2594 \cdot 10^{-25}$ |
| 8200  | $8.0517 \cdot 10^{-26}$ |
| 8300  | $5.1497 \cdot 10^{-26}$ |
| 8400  | $3.3065 \cdot 10^{-26}$ |
| 8500  | $2.1298 \cdot 10^{-26}$ |
| 8600  | $1.3772 \cdot 10^{-26}$ |
| 8700  | $8.8888 \cdot 10^{-27}$ |
| 8800  | $5.7961 \cdot 10^{-27}$ |
| 8900  | $3.7648 \cdot 10^{-27}$ |
| 9000  | $2.4454 \cdot 10^{-27}$ |
| 9100  | $1.5915 \cdot 10^{-27}$ |
| 9200  | $1.0407 \cdot 10^{-27}$ |
| 9300  | $6.8293 \cdot 10^{-28}$ |
| 9400  | $4.5234 \cdot 10^{-28}$ |
| 9500  | $2.9701 \cdot 10^{-28}$ |
| 9600  | $1.9649 \cdot 10^{-28}$ |
| 9700  | $1.2949 \cdot 10^{-28}$ |
| 9800  | $8.5698 \cdot 10^{-29}$ |
| 9900  | $5.7396 \cdot 10^{-29}$ |
| 10000 | $3.7850 \cdot 10^{-29}$ |
| 10100 | $2.5241 \cdot 10^{-29}$ |
| 10200 | $1.6883 \cdot 10^{-29}$ |
| 10300 | $1.1283 \cdot 10^{-29}$ |
| 10400 | $7.5768 \cdot 10^{-30}$ |
| 10500 | $5.1016 \cdot 10^{-30}$ |
| 10600 | $3.4435 \cdot 10^{-30}$ |
| 10700 | $2.3288 \cdot 10^{-30}$ |
| 10800 | $1.5782 \cdot 10^{-30}$ |
| 10900 | $1.0582 \cdot 10^{-30}$ |
| 11000 | $7.1427 \cdot 10^{-31}$ |
| 11100 | $4.8354 \cdot 10^{-31}$ |
| 11200 | $3.2850 \cdot 10^{-31}$ |
| 11300 | $2.2377 \cdot 10^{-31}$ |

Continued on next page

Table 8 – continued from previous page

| $b$   | $\varepsilon(b)$        |
|-------|-------------------------|
| 11400 | $1.5279 \cdot 10^{-31}$ |
| 11500 | $1.0434 \cdot 10^{-31}$ |
| 11600 | $7.1321 \cdot 10^{-32}$ |
| 11700 | $4.8892 \cdot 10^{-32}$ |
| 11800 | $3.3603 \cdot 10^{-32}$ |
| 11900 | $2.3147 \cdot 10^{-32}$ |
| 12000 | $1.5976 \cdot 10^{-32}$ |
| 12100 | $1.1048 \cdot 10^{-32}$ |
| 12200 | $7.5730 \cdot 10^{-33}$ |
| 12300 | $5.2476 \cdot 10^{-33}$ |
| 12400 | $3.6432 \cdot 10^{-33}$ |
| 12500 | $2.5337 \cdot 10^{-33}$ |
| 12600 | $1.7565 \cdot 10^{-33}$ |
| 12700 | $1.2188 \cdot 10^{-33}$ |
| 12800 | $8.4803 \cdot 10^{-34}$ |
| 12900 | $5.9154 \cdot 10^{-34}$ |
| 13000 | $4.1356 \cdot 10^{-34}$ |
| 14000 | $1.2266 \cdot 10^{-35}$ |
| 15000 | $4.1071 \cdot 10^{-37}$ |
| 16000 | $1.5141 \cdot 10^{-38}$ |
| 17000 | $6.2041 \cdot 10^{-40}$ |
| 18000 | $2.8284 \cdot 10^{-41}$ |
| 19000 | $1.3679 \cdot 10^{-42}$ |
| 20000 | $7.1622 \cdot 10^{-44}$ |
| 21000 | $4.1185 \cdot 10^{-45}$ |
| 22000 | $2.4393 \cdot 10^{-46}$ |
| 23000 | $1.5648 \cdot 10^{-47}$ |
| 24000 | $1.0703 \cdot 10^{-48}$ |
| 25000 | $7.5725 \cdot 10^{-50}$ |

Note that for the last line of this table it was produced using [1, Theorem 13] which gives  $|\psi(x) - x|/x < 7.5725 \cdot 10^{-50}$  is valid for  $e^{25000} \leq x \leq e^{26000}$ . We can say it holds for  $x \geq e^{25000}$  by making use of [7, Theorem 1] with  $A = 535.4$ ,  $B = 1.51$ ,  $C = 1.94$ , which gives for all  $x \geq e^{26000}$  that  $|\psi(x) - x|/x \leq 5.28498 \cdot 10^{-50}$ .

3. TABLE 9: SHARPER BOUNDS FOR  $\theta(x)$ :  $x$  IN A LARGE RANGE ( $x \geq e^{1000}$ )

TABLE 9. Values of  $\mathcal{A}_k(b)$  as defined in Corollary 7.1:  $|\theta(x) - x| < \frac{\mathcal{A}_k(b)x}{(\log x)^k}$  for  $x \geq e^b$ .

| $b_j$ | $\mathcal{A}_1$        | $\mathcal{A}_2$        | $\mathcal{A}_3$        | $\mathcal{A}_4$     | $\mathcal{A}_5$        |
|-------|------------------------|------------------------|------------------------|---------------------|------------------------|
| 1000  | $1.1919 \cdot 10^{-2}$ | $1.1919 \cdot 10^1$    | $1.1919 \cdot 10^4$    | $1.1919 \cdot 10^7$ | $1.1919 \cdot 10^{10}$ |
| 1500  | $1.0346 \cdot 10^{-4}$ | $1.5519 \cdot 10^{-1}$ | $2.3278 \cdot 10^2$    | $3.4917 \cdot 10^5$ | $5.2376 \cdot 10^8$    |
| 1600  | $4.3525 \cdot 10^{-5}$ | $6.9640 \cdot 10^{-2}$ | $1.1143 \cdot 10^2$    | $1.7828 \cdot 10^5$ | $2.8525 \cdot 10^8$    |
| 1700  | $1.8714 \cdot 10^{-5}$ | $3.1813 \cdot 10^{-2}$ | $5.4081 \cdot 10^1$    | $9.1938 \cdot 10^4$ | $1.5630 \cdot 10^8$    |
| 1725  | $1.5202 \cdot 10^{-5}$ | $2.6223 \cdot 10^{-2}$ | $4.5234 \cdot 10^1$    | $7.8029 \cdot 10^4$ | $1.3460 \cdot 10^8$    |
| 1750  | $1.2365 \cdot 10^{-5}$ | $2.1638 \cdot 10^{-2}$ | $3.7865 \cdot 10^1$    | $6.6264 \cdot 10^4$ | $1.1597 \cdot 10^8$    |
| 1775  | $1.0069 \cdot 10^{-5}$ | $1.7872 \cdot 10^{-2}$ | $3.1722 \cdot 10^1$    | $5.6306 \cdot 10^4$ | $9.9944 \cdot 10^7$    |
| 1800  | $8.2088 \cdot 10^{-6}$ | $1.4776 \cdot 10^{-2}$ | $2.6597 \cdot 10^1$    | $4.7874 \cdot 10^4$ | $8.6172 \cdot 10^7$    |
| 1825  | $6.7004 \cdot 10^{-6}$ | $1.2229 \cdot 10^{-2}$ | $2.2317 \cdot 10^1$    | $4.0728 \cdot 10^4$ | $7.4328 \cdot 10^7$    |
| 1850  | $5.4754 \cdot 10^{-6}$ | $1.0130 \cdot 10^{-2}$ | $1.8740 \cdot 10^1$    | $3.4669 \cdot 10^4$ | $6.4137 \cdot 10^7$    |
| 1875  | $4.4795 \cdot 10^{-6}$ | $8.3990 \cdot 10^{-3}$ | $1.5749 \cdot 10^1$    | $2.9528 \cdot 10^4$ | $5.5365 \cdot 10^7$    |
| 1900  | $3.6687 \cdot 10^{-6}$ | $6.9706 \cdot 10^{-3}$ | $1.3244 \cdot 10^1$    | $2.5164 \cdot 10^4$ | $4.7811 \cdot 10^7$    |
| 1925  | $3.0080 \cdot 10^{-6}$ | $5.7904 \cdot 10^{-3}$ | $1.1147 \cdot 10^1$    | $2.1457 \cdot 10^4$ | $4.1305 \cdot 10^7$    |
| 1950  | $2.4689 \cdot 10^{-6}$ | $4.8143 \cdot 10^{-3}$ | $9.3879 \cdot 10^0$    | $1.8307 \cdot 10^4$ | $3.5698 \cdot 10^7$    |
| 1975  | $2.0286 \cdot 10^{-6}$ | $4.0064 \cdot 10^{-3}$ | $7.9126 \cdot 10^0$    | $1.5628 \cdot 10^4$ | $3.0864 \cdot 10^7$    |
| 2000  | $1.6685 \cdot 10^{-6}$ | $3.3369 \cdot 10^{-3}$ | $6.6738 \cdot 10^0$    | $1.3348 \cdot 10^4$ | $2.6696 \cdot 10^7$    |
| 2025  | $1.3737 \cdot 10^{-6}$ | $2.7818 \cdot 10^{-3}$ | $5.6330 \cdot 10^0$    | $1.1407 \cdot 10^4$ | $2.3099 \cdot 10^7$    |
| 2050  | $1.1322 \cdot 10^{-6}$ | $2.3209 \cdot 10^{-3}$ | $4.7578 \cdot 10^0$    | $9.7535 \cdot 10^3$ | $1.9995 \cdot 10^7$    |
| 2075  | $9.3398 \cdot 10^{-7}$ | $1.9381 \cdot 10^{-3}$ | $4.0214 \cdot 10^0$    | $8.3444 \cdot 10^3$ | $1.7315 \cdot 10^7$    |
| 2100  | $7.7126 \cdot 10^{-7}$ | $1.6197 \cdot 10^{-3}$ | $3.4013 \cdot 10^0$    | $7.1426 \cdot 10^3$ | $1.5000 \cdot 10^7$    |
| 2125  | $6.3749 \cdot 10^{-7}$ | $1.3547 \cdot 10^{-3}$ | $2.8787 \cdot 10^0$    | $6.1172 \cdot 10^3$ | $1.2999 \cdot 10^7$    |
| 2150  | $5.2743 \cdot 10^{-7}$ | $1.1340 \cdot 10^{-3}$ | $2.4381 \cdot 10^0$    | $5.2418 \cdot 10^3$ | $1.1270 \cdot 10^7$    |
| 2175  | $4.3677 \cdot 10^{-7}$ | $9.4996 \cdot 10^{-4}$ | $2.0662 \cdot 10^0$    | $4.4940 \cdot 10^3$ | $9.7743 \cdot 10^6$    |
| 2200  | $3.6202 \cdot 10^{-7}$ | $7.9645 \cdot 10^{-4}$ | $1.7522 \cdot 10^0$    | $3.8548 \cdot 10^3$ | $8.4806 \cdot 10^6$    |
| 2225  | $3.0034 \cdot 10^{-7}$ | $6.6825 \cdot 10^{-4}$ | $1.4869 \cdot 10^0$    | $3.3083 \cdot 10^3$ | $7.3609 \cdot 10^6$    |
| 2250  | $2.4939 \cdot 10^{-7}$ | $5.6112 \cdot 10^{-4}$ | $1.2626 \cdot 10^0$    | $2.8407 \cdot 10^3$ | $6.3915 \cdot 10^6$    |
| 2275  | $2.0726 \cdot 10^{-7}$ | $4.7152 \cdot 10^{-4}$ | $1.0727 \cdot 10^0$    | $2.4404 \cdot 10^3$ | $5.5519 \cdot 10^6$    |
| 2300  | $1.7240 \cdot 10^{-7}$ | $3.9652 \cdot 10^{-4}$ | $9.1198 \cdot 10^{-1}$ | $2.0976 \cdot 10^3$ | $4.8244 \cdot 10^6$    |
| 2325  | $1.4352 \cdot 10^{-7}$ | $3.3369 \cdot 10^{-4}$ | $7.7582 \cdot 10^{-1}$ | $1.8038 \cdot 10^3$ | $4.1938 \cdot 10^6$    |
| 2350  | $1.1959 \cdot 10^{-7}$ | $2.8102 \cdot 10^{-4}$ | $6.6039 \cdot 10^{-1}$ | $1.5520 \cdot 10^3$ | $3.6470 \cdot 10^6$    |
| 2375  | $9.9718 \cdot 10^{-8}$ | $2.3683 \cdot 10^{-4}$ | $5.6247 \cdot 10^{-1}$ | $1.3359 \cdot 10^3$ | $3.1727 \cdot 10^6$    |
| 2400  | $8.3221 \cdot 10^{-8}$ | $1.9974 \cdot 10^{-4}$ | $4.7936 \cdot 10^{-1}$ | $1.1505 \cdot 10^3$ | $2.7611 \cdot 10^6$    |
| 2425  | $6.9510 \cdot 10^{-8}$ | $1.6857 \cdot 10^{-4}$ | $4.0876 \cdot 10^{-1}$ | $9.9125 \cdot 10^2$ | $2.4038 \cdot 10^6$    |
| 2450  | $5.8104 \cdot 10^{-8}$ | $1.4236 \cdot 10^{-4}$ | $3.4877 \cdot 10^{-1}$ | $8.5448 \cdot 10^2$ | $2.0935 \cdot 10^6$    |
| 2475  | $4.8607 \cdot 10^{-8}$ | $1.2031 \cdot 10^{-4}$ | $2.9775 \cdot 10^{-1}$ | $7.3693 \cdot 10^2$ | $1.8239 \cdot 10^6$    |
| 2500  | $4.0694 \cdot 10^{-8}$ | $1.0174 \cdot 10^{-4}$ | $2.5434 \cdot 10^{-1}$ | $6.3585 \cdot 10^2$ | $1.5897 \cdot 10^6$    |
| 2525  | $3.4095 \cdot 10^{-8}$ | $8.6090 \cdot 10^{-5}$ | $2.1738 \cdot 10^{-1}$ | $5.4888 \cdot 10^2$ | $1.3860 \cdot 10^6$    |
| 2550  | $2.8588 \cdot 10^{-8}$ | $7.2899 \cdot 10^{-5}$ | $1.8590 \cdot 10^{-1}$ | $4.7403 \cdot 10^2$ | $1.2088 \cdot 10^6$    |
| 2575  | $2.3988 \cdot 10^{-8}$ | $6.1769 \cdot 10^{-5}$ | $1.5906 \cdot 10^{-1}$ | $4.0957 \cdot 10^2$ | $1.0547 \cdot 10^6$    |
| 2600  | $2.0143 \cdot 10^{-8}$ | $5.2372 \cdot 10^{-5}$ | $1.3617 \cdot 10^{-1}$ | $3.5404 \cdot 10^2$ | $9.2049 \cdot 10^5$    |
| 2625  | $1.6927 \cdot 10^{-8}$ | $4.4432 \cdot 10^{-5}$ | $1.1664 \cdot 10^{-1}$ | $3.0617 \cdot 10^2$ | $8.0369 \cdot 10^5$    |
| 2650  | $1.4234 \cdot 10^{-8}$ | $3.7720 \cdot 10^{-5}$ | $9.9957 \cdot 10^{-2}$ | $2.6489 \cdot 10^2$ | $7.0195 \cdot 10^5$    |
| 2675  | $1.1978 \cdot 10^{-8}$ | $3.2041 \cdot 10^{-5}$ | $8.5710 \cdot 10^{-2}$ | $2.2928 \cdot 10^2$ | $6.1331 \cdot 10^5$    |
| 2700  | $1.0087 \cdot 10^{-8}$ | $2.7234 \cdot 10^{-5}$ | $7.3532 \cdot 10^{-2}$ | $1.9854 \cdot 10^2$ | $5.3605 \cdot 10^5$    |
| 2725  | $8.4999 \cdot 10^{-9}$ | $2.3163 \cdot 10^{-5}$ | $6.3117 \cdot 10^{-2}$ | $1.7200 \cdot 10^2$ | $4.6868 \cdot 10^5$    |
| 2750  | $7.1676 \cdot 10^{-9}$ | $1.9711 \cdot 10^{-5}$ | $5.4205 \cdot 10^{-2}$ | $1.4907 \cdot 10^2$ | $4.0992 \cdot 10^5$    |
| 2775  | $6.0481 \cdot 10^{-9}$ | $1.6784 \cdot 10^{-5}$ | $4.6575 \cdot 10^{-2}$ | $1.2925 \cdot 10^2$ | $3.5865 \cdot 10^5$    |
| 2800  | $5.1070 \cdot 10^{-9}$ | $1.4300 \cdot 10^{-5}$ | $4.0039 \cdot 10^{-2}$ | $1.1211 \cdot 10^2$ | $3.1390 \cdot 10^5$    |
| 2825  | $4.3151 \cdot 10^{-9}$ | $1.2190 \cdot 10^{-5}$ | $3.4437 \cdot 10^{-2}$ | $9.7283 \cdot 10^1$ | $2.7483 \cdot 10^5$    |

Continued on next page



Table 9 – continued from previous page

| $b_j$ | $\mathcal{A}_1$         | $\mathcal{A}_2$        | $\mathcal{A}_3$        | $\mathcal{A}_4$        | $\mathcal{A}_5$     |
|-------|-------------------------|------------------------|------------------------|------------------------|---------------------|
| 2850  | $3.6483 \cdot 10^{-9}$  | $1.0398 \cdot 10^{-5}$ | $2.9634 \cdot 10^{-2}$ | $8.4455 \cdot 10^1$    | $2.4070 \cdot 10^5$ |
| 2875  | $3.0866 \cdot 10^{-9}$  | $8.8738 \cdot 10^{-6}$ | $2.5513 \cdot 10^{-2}$ | $7.3348 \cdot 10^1$    | $2.1088 \cdot 10^5$ |
| 2900  | $2.6130 \cdot 10^{-9}$  | $7.5776 \cdot 10^{-6}$ | $2.1975 \cdot 10^{-2}$ | $6.3727 \cdot 10^1$    | $1.8481 \cdot 10^5$ |
| 2925  | $2.2134 \cdot 10^{-9}$  | $6.4742 \cdot 10^{-6}$ | $1.8938 \cdot 10^{-2}$ | $5.5391 \cdot 10^1$    | $1.6202 \cdot 10^5$ |
| 2950  | $1.8762 \cdot 10^{-9}$  | $5.5346 \cdot 10^{-6}$ | $1.6327 \cdot 10^{-2}$ | $4.8165 \cdot 10^1$    | $1.4209 \cdot 10^5$ |
| 2975  | $1.5912 \cdot 10^{-9}$  | $4.7339 \cdot 10^{-6}$ | $1.4084 \cdot 10^{-2}$ | $4.1898 \cdot 10^1$    | $1.2465 \cdot 10^5$ |
| 3000  | $1.3504 \cdot 10^{-9}$  | $4.0512 \cdot 10^{-6}$ | $1.2154 \cdot 10^{-2}$ | $3.6460 \cdot 10^1$    | $1.0938 \cdot 10^5$ |
| 3025  | $1.1467 \cdot 10^{-9}$  | $3.4687 \cdot 10^{-6}$ | $1.0493 \cdot 10^{-2}$ | $3.1741 \cdot 10^1$    | $9.6016 \cdot 10^4$ |
| 3050  | $9.7429 \cdot 10^{-10}$ | $2.9716 \cdot 10^{-6}$ | $9.0633 \cdot 10^{-3}$ | $2.7644 \cdot 10^1$    | $8.4312 \cdot 10^4$ |
| 3075  | $8.2830 \cdot 10^{-10}$ | $2.5471 \cdot 10^{-6}$ | $7.8321 \cdot 10^{-3}$ | $2.4084 \cdot 10^1$    | $7.4057 \cdot 10^4$ |
| 3100  | $7.0459 \cdot 10^{-10}$ | $2.1843 \cdot 10^{-6}$ | $6.7712 \cdot 10^{-3}$ | $2.0991 \cdot 10^1$    | $6.5071 \cdot 10^4$ |
| 3125  | $5.9971 \cdot 10^{-10}$ | $1.8741 \cdot 10^{-6}$ | $5.8565 \cdot 10^{-3}$ | $1.8302 \cdot 10^1$    | $5.7193 \cdot 10^4$ |
| 3150  | $5.1072 \cdot 10^{-10}$ | $1.6088 \cdot 10^{-6}$ | $5.0676 \cdot 10^{-3}$ | $1.5963 \cdot 10^1$    | $5.0284 \cdot 10^4$ |
| 3175  | $4.3519 \cdot 10^{-10}$ | $1.3818 \cdot 10^{-6}$ | $4.3869 \cdot 10^{-3}$ | $1.3929 \cdot 10^1$    | $4.4223 \cdot 10^4$ |
| 3200  | $3.7103 \cdot 10^{-10}$ | $1.1873 \cdot 10^{-6}$ | $3.7993 \cdot 10^{-3}$ | $1.2158 \cdot 10^1$    | $3.8905 \cdot 10^4$ |
| 3225  | $3.1650 \cdot 10^{-10}$ | $1.0207 \cdot 10^{-6}$ | $3.2918 \cdot 10^{-3}$ | $1.0616 \cdot 10^1$    | $3.4237 \cdot 10^4$ |
| 3250  | $2.7013 \cdot 10^{-10}$ | $8.7793 \cdot 10^{-7}$ | $2.8533 \cdot 10^{-3}$ | $9.2731 \cdot 10^0$    | $3.0138 \cdot 10^4$ |
| 3275  | $2.3069 \cdot 10^{-10}$ | $7.5548 \cdot 10^{-7}$ | $2.4742 \cdot 10^{-3}$ | $8.1030 \cdot 10^0$    | $2.6538 \cdot 10^4$ |
| 3300  | $1.9710 \cdot 10^{-10}$ | $6.5042 \cdot 10^{-7}$ | $2.1464 \cdot 10^{-3}$ | $7.0831 \cdot 10^0$    | $2.3375 \cdot 10^4$ |
| 3325  | $1.6850 \cdot 10^{-10}$ | $5.6024 \cdot 10^{-7}$ | $1.8628 \cdot 10^{-3}$ | $6.1938 \cdot 10^0$    | $2.0595 \cdot 10^4$ |
| 3350  | $1.4412 \cdot 10^{-10}$ | $4.8278 \cdot 10^{-7}$ | $1.6173 \cdot 10^{-3}$ | $5.4180 \cdot 10^0$    | $1.8151 \cdot 10^4$ |
| 3375  | $1.2333 \cdot 10^{-10}$ | $4.1622 \cdot 10^{-7}$ | $1.4048 \cdot 10^{-3}$ | $4.7410 \cdot 10^0$    | $1.6001 \cdot 10^4$ |
| 3400  | $1.0559 \cdot 10^{-10}$ | $3.5901 \cdot 10^{-7}$ | $1.2207 \cdot 10^{-3}$ | $4.1501 \cdot 10^0$    | $1.4111 \cdot 10^4$ |
| 3425  | $9.0450 \cdot 10^{-11}$ | $3.0979 \cdot 10^{-7}$ | $1.0611 \cdot 10^{-3}$ | $3.6341 \cdot 10^0$    | $1.2447 \cdot 10^4$ |
| 3450  | $7.7520 \cdot 10^{-11}$ | $2.6745 \cdot 10^{-7}$ | $9.2268 \cdot 10^{-4}$ | $3.1833 \cdot 10^0$    | $1.0983 \cdot 10^4$ |
| 3475  | $6.6472 \cdot 10^{-11}$ | $2.3099 \cdot 10^{-7}$ | $8.0269 \cdot 10^{-4}$ | $2.7894 \cdot 10^0$    | $9.6929 \cdot 10^3$ |
| 3500  | $5.7026 \cdot 10^{-11}$ | $1.9959 \cdot 10^{-7}$ | $6.9857 \cdot 10^{-4}$ | $2.4450 \cdot 10^0$    | $8.5574 \cdot 10^3$ |
| 3525  | $4.8946 \cdot 10^{-11}$ | $1.7254 \cdot 10^{-7}$ | $6.0819 \cdot 10^{-4}$ | $2.1439 \cdot 10^0$    | $7.5571 \cdot 10^3$ |
| 3550  | $4.2032 \cdot 10^{-11}$ | $1.4922 \cdot 10^{-7}$ | $5.2970 \cdot 10^{-4}$ | $1.8805 \cdot 10^0$    | $6.6756 \cdot 10^3$ |
| 3575  | $3.6111 \cdot 10^{-11}$ | $1.2910 \cdot 10^{-7}$ | $4.6152 \cdot 10^{-4}$ | $1.6500 \cdot 10^0$    | $5.8985 \cdot 10^3$ |
| 3600  | $3.1039 \cdot 10^{-11}$ | $1.1174 \cdot 10^{-7}$ | $4.0226 \cdot 10^{-4}$ | $1.4482 \cdot 10^0$    | $5.2133 \cdot 10^3$ |
| 3625  | $2.6692 \cdot 10^{-11}$ | $9.6757 \cdot 10^{-8}$ | $3.5075 \cdot 10^{-4}$ | $1.2715 \cdot 10^0$    | $4.6090 \cdot 10^3$ |
| 3650  | $2.2964 \cdot 10^{-11}$ | $8.3819 \cdot 10^{-8}$ | $3.0594 \cdot 10^{-4}$ | $1.1167 \cdot 10^0$    | $4.0759 \cdot 10^3$ |
| 3675  | $1.9766 \cdot 10^{-11}$ | $7.2640 \cdot 10^{-8}$ | $2.6696 \cdot 10^{-4}$ | $9.8105 \cdot 10^{-1}$ | $3.6054 \cdot 10^3$ |
| 3700  | $1.7022 \cdot 10^{-11}$ | $6.2978 \cdot 10^{-8}$ | $2.3302 \cdot 10^{-4}$ | $8.6217 \cdot 10^{-1}$ | $3.1901 \cdot 10^3$ |
| 3725  | $1.4665 \cdot 10^{-11}$ | $5.4624 \cdot 10^{-8}$ | $2.0348 \cdot 10^{-4}$ | $7.5794 \cdot 10^{-1}$ | $2.8234 \cdot 10^3$ |
| 3750  | $1.2639 \cdot 10^{-11}$ | $4.7397 \cdot 10^{-8}$ | $1.7774 \cdot 10^{-4}$ | $6.6651 \cdot 10^{-1}$ | $2.4995 \cdot 10^3$ |
| 3775  | $1.0899 \cdot 10^{-11}$ | $4.1142 \cdot 10^{-8}$ | $1.5531 \cdot 10^{-4}$ | $5.8630 \cdot 10^{-1}$ | $2.2133 \cdot 10^3$ |
| 3800  | $9.4017 \cdot 10^{-12}$ | $3.5727 \cdot 10^{-8}$ | $1.3577 \cdot 10^{-4}$ | $5.1589 \cdot 10^{-1}$ | $1.9604 \cdot 10^3$ |
| 3825  | $8.1141 \cdot 10^{-12}$ | $3.1037 \cdot 10^{-8}$ | $1.1872 \cdot 10^{-4}$ | $4.5408 \cdot 10^{-1}$ | $1.7369 \cdot 10^3$ |
| 3850  | $7.0058 \cdot 10^{-12}$ | $2.6973 \cdot 10^{-8}$ | $1.0385 \cdot 10^{-4}$ | $3.9980 \cdot 10^{-1}$ | $1.5393 \cdot 10^3$ |
| 3875  | $6.0515 \cdot 10^{-12}$ | $2.3450 \cdot 10^{-8}$ | $9.0867 \cdot 10^{-5}$ | $3.5211 \cdot 10^{-1}$ | $1.3645 \cdot 10^3$ |
| 3900  | $5.2294 \cdot 10^{-12}$ | $2.0395 \cdot 10^{-8}$ | $7.9539 \cdot 10^{-5}$ | $3.1020 \cdot 10^{-1}$ | $1.2098 \cdot 10^3$ |
| 3925  | $4.5209 \cdot 10^{-12}$ | $1.7745 \cdot 10^{-8}$ | $6.9647 \cdot 10^{-5}$ | $2.7337 \cdot 10^{-1}$ | $1.0730 \cdot 10^3$ |
| 3950  | $3.9100 \cdot 10^{-12}$ | $1.5445 \cdot 10^{-8}$ | $6.1005 \cdot 10^{-5}$ | $2.4097 \cdot 10^{-1}$ | $9.5183 \cdot 10^2$ |
| 3975  | $3.3830 \cdot 10^{-12}$ | $1.3448 \cdot 10^{-8}$ | $5.3453 \cdot 10^{-5}$ | $2.1248 \cdot 10^{-1}$ | $8.4460 \cdot 10^2$ |
| 4000  | $2.9283 \cdot 10^{-12}$ | $1.1713 \cdot 10^{-8}$ | $4.6852 \cdot 10^{-5}$ | $1.8741 \cdot 10^{-1}$ | $7.4963 \cdot 10^2$ |
| 4025  | $2.5357 \cdot 10^{-12}$ | $1.0206 \cdot 10^{-8}$ | $4.1080 \cdot 10^{-5}$ | $1.6535 \cdot 10^{-1}$ | $6.6551 \cdot 10^2$ |
| 4050  | $2.1966 \cdot 10^{-12}$ | $8.8962 \cdot 10^{-9}$ | $3.6030 \cdot 10^{-5}$ | $1.4592 \cdot 10^{-1}$ | $5.9098 \cdot 10^2$ |
| 4075  | $1.9037 \cdot 10^{-12}$ | $7.7573 \cdot 10^{-9}$ | $3.1611 \cdot 10^{-5}$ | $1.2882 \cdot 10^{-1}$ | $5.2492 \cdot 10^2$ |
| 4100  | $1.6504 \cdot 10^{-12}$ | $6.7666 \cdot 10^{-9}$ | $2.7743 \cdot 10^{-5}$ | $1.1375 \cdot 10^{-1}$ | $4.6636 \cdot 10^2$ |
| 4125  | $1.4314 \cdot 10^{-12}$ | $5.9045 \cdot 10^{-9}$ | $2.4356 \cdot 10^{-5}$ | $1.0047 \cdot 10^{-1}$ | $4.1443 \cdot 10^2$ |
| 4150  | $1.2420 \cdot 10^{-12}$ | $5.1540 \cdot 10^{-9}$ | $2.1390 \cdot 10^{-5}$ | $8.8765 \cdot 10^{-2}$ | $3.6838 \cdot 10^2$ |
| 4175  | $1.0780 \cdot 10^{-12}$ | $4.5005 \cdot 10^{-9}$ | $1.8790 \cdot 10^{-5}$ | $7.8447 \cdot 10^{-2}$ | $3.2752 \cdot 10^2$ |
| 4200  | $9.3601 \cdot 10^{-13}$ | $3.9313 \cdot 10^{-9}$ | $1.6512 \cdot 10^{-5}$ | $6.9347 \cdot 10^{-2}$ | $2.9126 \cdot 10^2$ |

Continued on next page

Table 9 – continued from previous page

| $b_j$ | $\mathcal{A}_1$         | $\mathcal{A}_2$         | $\mathcal{A}_3$         | $\mathcal{A}_4$        | $\mathcal{A}_5$        |
|-------|-------------------------|-------------------------|-------------------------|------------------------|------------------------|
| 4225  | $8.1306 \cdot 10^{-13}$ | $3.4352 \cdot 10^{-9}$  | $1.4514 \cdot 10^{-5}$  | $6.1320 \cdot 10^{-2}$ | $2.5908 \cdot 10^2$    |
| 4250  | $7.0652 \cdot 10^{-13}$ | $3.0027 \cdot 10^{-9}$  | $1.2762 \cdot 10^{-5}$  | $5.4237 \cdot 10^{-2}$ | $2.3051 \cdot 10^2$    |
| 4275  | $6.1417 \cdot 10^{-13}$ | $2.6256 \cdot 10^{-9}$  | $1.1225 \cdot 10^{-5}$  | $4.7984 \cdot 10^{-2}$ | $2.0514 \cdot 10^2$    |
| 4300  | $5.3409 \cdot 10^{-13}$ | $2.2966 \cdot 10^{-9}$  | $9.8753 \cdot 10^{-6}$  | $4.2464 \cdot 10^{-2}$ | $1.8260 \cdot 10^2$    |
| 4325  | $4.6463 \cdot 10^{-13}$ | $2.0095 \cdot 10^{-9}$  | $8.6911 \cdot 10^{-6}$  | $3.7589 \cdot 10^{-2}$ | $1.6258 \cdot 10^2$    |
| 4350  | $4.0434 \cdot 10^{-13}$ | $1.7589 \cdot 10^{-9}$  | $7.6511 \cdot 10^{-6}$  | $3.3283 \cdot 10^{-2}$ | $1.4478 \cdot 10^2$    |
| 4375  | $3.5200 \cdot 10^{-13}$ | $1.5400 \cdot 10^{-9}$  | $6.7375 \cdot 10^{-6}$  | $2.9477 \cdot 10^{-2}$ | $1.2896 \cdot 10^2$    |
| 4400  | $2.9127 \cdot 10^{-13}$ | $1.2816 \cdot 10^{-9}$  | $5.6389 \cdot 10^{-6}$  | $2.4811 \cdot 10^{-2}$ | $1.0917 \cdot 10^2$    |
| 4425  | $2.3892 \cdot 10^{-13}$ | $1.0573 \cdot 10^{-9}$  | $4.6782 \cdot 10^{-6}$  | $2.0701 \cdot 10^{-2}$ | $9.1601 \cdot 10^1$    |
| 4450  | $1.9646 \cdot 10^{-13}$ | $8.7423 \cdot 10^{-10}$ | $3.8904 \cdot 10^{-6}$  | $1.7312 \cdot 10^{-2}$ | $7.7038 \cdot 10^1$    |
| 4475  | $1.6195 \cdot 10^{-13}$ | $7.2470 \cdot 10^{-10}$ | $3.2431 \cdot 10^{-6}$  | $1.4513 \cdot 10^{-2}$ | $6.4944 \cdot 10^1$    |
| 4500  | $1.3384 \cdot 10^{-13}$ | $6.0225 \cdot 10^{-10}$ | $2.7101 \cdot 10^{-6}$  | $1.2196 \cdot 10^{-2}$ | $5.4880 \cdot 10^1$    |
| 4525  | $1.1089 \cdot 10^{-13}$ | $5.0175 \cdot 10^{-10}$ | $2.2705 \cdot 10^{-6}$  | $1.0274 \cdot 10^{-2}$ | $4.6489 \cdot 10^1$    |
| 4550  | $9.2109 \cdot 10^{-14}$ | $4.1910 \cdot 10^{-10}$ | $1.9069 \cdot 10^{-6}$  | $8.6763 \cdot 10^{-3}$ | $3.9477 \cdot 10^1$    |
| 4575  | $7.6711 \cdot 10^{-14}$ | $3.5096 \cdot 10^{-10}$ | $1.6057 \cdot 10^{-6}$  | $7.3457 \cdot 10^{-3}$ | $3.3607 \cdot 10^1$    |
| 4600  | $6.4053 \cdot 10^{-14}$ | $2.9465 \cdot 10^{-10}$ | $1.3554 \cdot 10^{-6}$  | $6.2347 \cdot 10^{-3}$ | $2.8680 \cdot 10^1$    |
| 4625  | $5.3622 \cdot 10^{-14}$ | $2.4800 \cdot 10^{-10}$ | $1.1470 \cdot 10^{-6}$  | $5.3049 \cdot 10^{-3}$ | $2.4535 \cdot 10^1$    |
| 4650  | $4.5004 \cdot 10^{-14}$ | $2.0927 \cdot 10^{-10}$ | $9.7309 \cdot 10^{-7}$  | $4.5249 \cdot 10^{-3}$ | $2.1041 \cdot 10^1$    |
| 4675  | $3.7866 \cdot 10^{-14}$ | $1.7703 \cdot 10^{-10}$ | $8.2757 \cdot 10^{-7}$  | $3.8689 \cdot 10^{-3}$ | $1.8088 \cdot 10^1$    |
| 4700  | $3.1938 \cdot 10^{-14}$ | $1.5011 \cdot 10^{-10}$ | $7.0551 \cdot 10^{-7}$  | $3.3159 \cdot 10^{-3}$ | $1.5585 \cdot 10^1$    |
| 4725  | $2.7004 \cdot 10^{-14}$ | $1.2760 \cdot 10^{-10}$ | $6.0287 \cdot 10^{-7}$  | $2.8486 \cdot 10^{-3}$ | $1.3460 \cdot 10^1$    |
| 4750  | $2.2885 \cdot 10^{-14}$ | $1.0871 \cdot 10^{-10}$ | $5.1633 \cdot 10^{-7}$  | $2.4526 \cdot 10^{-3}$ | $1.1650 \cdot 10^1$    |
| 4775  | $1.9438 \cdot 10^{-14}$ | $9.2816 \cdot 10^{-11}$ | $4.4320 \cdot 10^{-7}$  | $2.1163 \cdot 10^{-3}$ | $1.0106 \cdot 10^1$    |
| 4800  | $1.6547 \cdot 10^{-14}$ | $7.9423 \cdot 10^{-11}$ | $3.8123 \cdot 10^{-7}$  | $1.8299 \cdot 10^{-3}$ | $8.7835 \cdot 10^0$    |
| 4825  | $1.4115 \cdot 10^{-14}$ | $6.8103 \cdot 10^{-11}$ | $3.2860 \cdot 10^{-7}$  | $1.5855 \cdot 10^{-3}$ | $7.6500 \cdot 10^0$    |
| 4850  | $1.2065 \cdot 10^{-14}$ | $5.8513 \cdot 10^{-11}$ | $2.8379 \cdot 10^{-7}$  | $1.3764 \cdot 10^{-3}$ | $6.6754 \cdot 10^0$    |
| 4875  | $1.0332 \cdot 10^{-14}$ | $5.0369 \cdot 10^{-11}$ | $2.4555 \cdot 10^{-7}$  | $1.1971 \cdot 10^{-3}$ | $5.8356 \cdot 10^0$    |
| 4900  | $8.8645 \cdot 10^{-15}$ | $4.3436 \cdot 10^{-11}$ | $2.1284 \cdot 10^{-7}$  | $1.0429 \cdot 10^{-3}$ | $5.1102 \cdot 10^0$    |
| 4925  | $7.6187 \cdot 10^{-15}$ | $3.7522 \cdot 10^{-11}$ | $1.8480 \cdot 10^{-7}$  | $9.1012 \cdot 10^{-4}$ | $4.4824 \cdot 10^0$    |
| 4950  | $6.5587 \cdot 10^{-15}$ | $3.2466 \cdot 10^{-11}$ | $1.6071 \cdot 10^{-7}$  | $7.9549 \cdot 10^{-4}$ | $3.9377 \cdot 10^0$    |
| 4975  | $5.6551 \cdot 10^{-15}$ | $2.8134 \cdot 10^{-11}$ | $1.3997 \cdot 10^{-7}$  | $6.9633 \cdot 10^{-4}$ | $3.4643 \cdot 10^0$    |
| 5000  | $4.8831 \cdot 10^{-15}$ | $2.4416 \cdot 10^{-11}$ | $1.2208 \cdot 10^{-7}$  | $6.1039 \cdot 10^{-4}$ | $3.0520 \cdot 10^0$    |
| 5100  | $2.7505 \cdot 10^{-15}$ | $1.4028 \cdot 10^{-11}$ | $7.1540 \cdot 10^{-8}$  | $3.6486 \cdot 10^{-4}$ | $1.8608 \cdot 10^0$    |
| 5200  | $1.5765 \cdot 10^{-15}$ | $8.1977 \cdot 10^{-12}$ | $4.2628 \cdot 10^{-8}$  | $2.2167 \cdot 10^{-4}$ | $1.1527 \cdot 10^0$    |
| 5300  | $9.1594 \cdot 10^{-16}$ | $4.8545 \cdot 10^{-12}$ | $2.5729 \cdot 10^{-8}$  | $1.3637 \cdot 10^{-4}$ | $7.2272 \cdot 10^{-1}$ |
| 5400  | $5.3785 \cdot 10^{-16}$ | $2.9044 \cdot 10^{-12}$ | $1.5684 \cdot 10^{-8}$  | $8.4692 \cdot 10^{-5}$ | $4.5734 \cdot 10^{-1}$ |
| 5500  | $3.1854 \cdot 10^{-16}$ | $1.7520 \cdot 10^{-12}$ | $9.6357 \cdot 10^{-9}$  | $5.2997 \cdot 10^{-5}$ | $2.9148 \cdot 10^{-1}$ |
| 5600  | $1.8998 \cdot 10^{-16}$ | $1.0639 \cdot 10^{-12}$ | $5.9577 \cdot 10^{-9}$  | $3.3363 \cdot 10^{-5}$ | $1.8684 \cdot 10^{-1}$ |
| 5700  | $1.1399 \cdot 10^{-16}$ | $6.4969 \cdot 10^{-13}$ | $3.7033 \cdot 10^{-9}$  | $2.1109 \cdot 10^{-5}$ | $1.2032 \cdot 10^{-1}$ |
| 5800  | $6.8742 \cdot 10^{-17}$ | $3.9871 \cdot 10^{-13}$ | $2.3125 \cdot 10^{-9}$  | $1.3413 \cdot 10^{-5}$ | $7.7792 \cdot 10^{-2}$ |
| 5900  | $4.1654 \cdot 10^{-17}$ | $2.4576 \cdot 10^{-13}$ | $1.4500 \cdot 10^{-9}$  | $8.5548 \cdot 10^{-6}$ | $5.0474 \cdot 10^{-2}$ |
| 6000  | $2.5350 \cdot 10^{-17}$ | $1.5210 \cdot 10^{-13}$ | $9.1257 \cdot 10^{-10}$ | $5.4755 \cdot 10^{-6}$ | $3.2853 \cdot 10^{-2}$ |
| 6100  | $1.5490 \cdot 10^{-17}$ | $9.4486 \cdot 10^{-14}$ | $5.7637 \cdot 10^{-10}$ | $3.5159 \cdot 10^{-6}$ | $2.1447 \cdot 10^{-2}$ |
| 6200  | $9.5014 \cdot 10^{-18}$ | $5.8909 \cdot 10^{-14}$ | $3.6524 \cdot 10^{-10}$ | $2.2645 \cdot 10^{-6}$ | $1.4040 \cdot 10^{-2}$ |
| 6300  | $5.8498 \cdot 10^{-18}$ | $3.6854 \cdot 10^{-14}$ | $2.3218 \cdot 10^{-10}$ | $1.4628 \cdot 10^{-6}$ | $9.2152 \cdot 10^{-3}$ |
| 6400  | $3.6145 \cdot 10^{-18}$ | $2.3133 \cdot 10^{-14}$ | $1.4805 \cdot 10^{-10}$ | $9.4752 \cdot 10^{-7}$ | $6.0642 \cdot 10^{-3}$ |
| 6500  | $2.2412 \cdot 10^{-18}$ | $1.4568 \cdot 10^{-14}$ | $9.4687 \cdot 10^{-11}$ | $6.1547 \cdot 10^{-7}$ | $4.0006 \cdot 10^{-3}$ |
| 6600  | $1.3943 \cdot 10^{-18}$ | $9.2021 \cdot 10^{-15}$ | $6.0734 \cdot 10^{-11}$ | $4.0085 \cdot 10^{-7}$ | $2.6456 \cdot 10^{-3}$ |
| 6700  | $8.7028 \cdot 10^{-19}$ | $5.8309 \cdot 10^{-15}$ | $3.9067 \cdot 10^{-11}$ | $2.6175 \cdot 10^{-7}$ | $1.7537 \cdot 10^{-3}$ |
| 6800  | $5.4496 \cdot 10^{-19}$ | $3.7058 \cdot 10^{-15}$ | $2.5199 \cdot 10^{-11}$ | $1.7136 \cdot 10^{-7}$ | $1.1652 \cdot 10^{-3}$ |
| 6900  | $3.4233 \cdot 10^{-19}$ | $2.3621 \cdot 10^{-15}$ | $1.6299 \cdot 10^{-11}$ | $1.1246 \cdot 10^{-7}$ | $7.7596 \cdot 10^{-4}$ |
| 7000  | $2.1571 \cdot 10^{-19}$ | $1.5100 \cdot 10^{-15}$ | $1.0570 \cdot 10^{-11}$ | $7.3987 \cdot 10^{-8}$ | $5.1791 \cdot 10^{-4}$ |
| 7100  | $1.3633 \cdot 10^{-19}$ | $9.6793 \cdot 10^{-16}$ | $6.8723 \cdot 10^{-12}$ | $4.8794 \cdot 10^{-8}$ | $3.4644 \cdot 10^{-4}$ |
| 7200  | $8.6417 \cdot 10^{-20}$ | $6.2220 \cdot 10^{-16}$ | $4.4799 \cdot 10^{-12}$ | $3.2255 \cdot 10^{-8}$ | $2.3224 \cdot 10^{-4}$ |
| 7300  | $5.4938 \cdot 10^{-20}$ | $4.0105 \cdot 10^{-16}$ | $2.9277 \cdot 10^{-12}$ | $2.1372 \cdot 10^{-8}$ | $1.5602 \cdot 10^{-4}$ |

Continued on next page

Table 9 – continued from previous page

| $b_j$ | $\mathcal{A}_1$         | $\mathcal{A}_2$         | $\mathcal{A}_3$         | $\mathcal{A}_4$         | $\mathcal{A}_5$         |
|-------|-------------------------|-------------------------|-------------------------|-------------------------|-------------------------|
| 7400  | $3.5025 \cdot 10^{-20}$ | $2.5919 \cdot 10^{-16}$ | $1.9180 \cdot 10^{-12}$ | $1.4193 \cdot 10^{-8}$  | $1.0503 \cdot 10^{-4}$  |
| 7500  | $2.2393 \cdot 10^{-20}$ | $1.6795 \cdot 10^{-16}$ | $1.2596 \cdot 10^{-12}$ | $9.4468 \cdot 10^{-9}$  | $7.0851 \cdot 10^{-5}$  |
| 7600  | $1.4356 \cdot 10^{-20}$ | $1.0910 \cdot 10^{-16}$ | $8.2915 \cdot 10^{-13}$ | $6.3016 \cdot 10^{-9}$  | $4.7892 \cdot 10^{-5}$  |
| 7700  | $9.2275 \cdot 10^{-21}$ | $7.1052 \cdot 10^{-17}$ | $5.4710 \cdot 10^{-13}$ | $4.2127 \cdot 10^{-9}$  | $3.2438 \cdot 10^{-5}$  |
| 7800  | $5.9471 \cdot 10^{-21}$ | $4.6388 \cdot 10^{-17}$ | $3.6183 \cdot 10^{-13}$ | $2.8222 \cdot 10^{-9}$  | $2.2014 \cdot 10^{-5}$  |
| 7900  | $3.8429 \cdot 10^{-21}$ | $3.0359 \cdot 10^{-17}$ | $2.3984 \cdot 10^{-13}$ | $1.8947 \cdot 10^{-9}$  | $1.4968 \cdot 10^{-5}$  |
| 8000  | $2.4895 \cdot 10^{-21}$ | $1.9916 \cdot 10^{-17}$ | $1.5933 \cdot 10^{-13}$ | $1.2747 \cdot 10^{-9}$  | $1.0197 \cdot 10^{-5}$  |
| 8100  | $1.6168 \cdot 10^{-21}$ | $1.3096 \cdot 10^{-17}$ | $1.0608 \cdot 10^{-13}$ | $8.5921 \cdot 10^{-10}$ | $6.9596 \cdot 10^{-6}$  |
| 8200  | $1.0526 \cdot 10^{-21}$ | $8.6311 \cdot 10^{-18}$ | $7.0775 \cdot 10^{-14}$ | $5.8036 \cdot 10^{-10}$ | $4.7589 \cdot 10^{-6}$  |
| 8300  | $6.8692 \cdot 10^{-22}$ | $5.7015 \cdot 10^{-18}$ | $4.7322 \cdot 10^{-14}$ | $3.9278 \cdot 10^{-10}$ | $3.2600 \cdot 10^{-6}$  |
| 8400  | $4.4936 \cdot 10^{-22}$ | $3.7746 \cdot 10^{-18}$ | $3.1707 \cdot 10^{-14}$ | $2.6634 \cdot 10^{-10}$ | $2.2373 \cdot 10^{-6}$  |
| 8500  | $2.9465 \cdot 10^{-22}$ | $2.5045 \cdot 10^{-18}$ | $2.1288 \cdot 10^{-14}$ | $1.8095 \cdot 10^{-10}$ | $1.5381 \cdot 10^{-6}$  |
| 8600  | $1.9364 \cdot 10^{-22}$ | $1.6653 \cdot 10^{-18}$ | $1.4322 \cdot 10^{-14}$ | $1.2317 \cdot 10^{-10}$ | $1.0593 \cdot 10^{-6}$  |
| 8700  | $1.2755 \cdot 10^{-22}$ | $1.1097 \cdot 10^{-18}$ | $9.6540 \cdot 10^{-15}$ | $8.3990 \cdot 10^{-11}$ | $7.3071 \cdot 10^{-7}$  |
| 8800  | $8.4200 \cdot 10^{-23}$ | $7.4096 \cdot 10^{-19}$ | $6.5205 \cdot 10^{-15}$ | $5.7380 \cdot 10^{-11}$ | $5.0495 \cdot 10^{-7}$  |
| 8900  | $5.5707 \cdot 10^{-23}$ | $4.9579 \cdot 10^{-19}$ | $4.4125 \cdot 10^{-15}$ | $3.9272 \cdot 10^{-11}$ | $3.4952 \cdot 10^{-7}$  |
| 9000  | $3.6935 \cdot 10^{-23}$ | $3.3241 \cdot 10^{-19}$ | $2.9917 \cdot 10^{-15}$ | $2.6926 \cdot 10^{-11}$ | $2.4233 \cdot 10^{-7}$  |
| 9100  | $2.4541 \cdot 10^{-23}$ | $2.2332 \cdot 10^{-19}$ | $2.0322 \cdot 10^{-15}$ | $1.8493 \cdot 10^{-11}$ | $1.6829 \cdot 10^{-7}$  |
| 9200  | $1.6340 \cdot 10^{-23}$ | $1.5032 \cdot 10^{-19}$ | $1.3830 \cdot 10^{-15}$ | $1.2724 \cdot 10^{-11}$ | $1.1706 \cdot 10^{-7}$  |
| 9300  | $1.0902 \cdot 10^{-23}$ | $1.0139 \cdot 10^{-19}$ | $9.4285 \cdot 10^{-16}$ | $8.7685 \cdot 10^{-12}$ | $8.1547 \cdot 10^{-8}$  |
| 9400  | $7.2878 \cdot 10^{-24}$ | $6.8506 \cdot 10^{-20}$ | $6.4395 \cdot 10^{-16}$ | $6.0532 \cdot 10^{-12}$ | $5.6900 \cdot 10^{-8}$  |
| 9500  | $4.8819 \cdot 10^{-24}$ | $4.6378 \cdot 10^{-20}$ | $4.4059 \cdot 10^{-16}$ | $4.1856 \cdot 10^{-12}$ | $3.9763 \cdot 10^{-8}$  |
| 9600  | $3.2766 \cdot 10^{-24}$ | $3.1456 \cdot 10^{-20}$ | $3.0197 \cdot 10^{-16}$ | $2.8990 \cdot 10^{-12}$ | $2.7830 \cdot 10^{-8}$  |
| 9700  | $2.2035 \cdot 10^{-24}$ | $2.1374 \cdot 10^{-20}$ | $2.0733 \cdot 10^{-16}$ | $2.0111 \cdot 10^{-12}$ | $1.9507 \cdot 10^{-8}$  |
| 9800  | $1.4846 \cdot 10^{-24}$ | $1.4549 \cdot 10^{-20}$ | $1.4258 \cdot 10^{-16}$ | $1.3973 \cdot 10^{-12}$ | $1.3694 \cdot 10^{-8}$  |
| 9900  | $1.0022 \cdot 10^{-24}$ | $9.9212 \cdot 10^{-21}$ | $9.8219 \cdot 10^{-17}$ | $9.7237 \cdot 10^{-13}$ | $9.6265 \cdot 10^{-9}$  |
| 10000 | $6.7772 \cdot 10^{-25}$ | $6.7772 \cdot 10^{-21}$ | $6.7772 \cdot 10^{-17}$ | $6.7772 \cdot 10^{-13}$ | $6.7772 \cdot 10^{-9}$  |
| 10100 | $4.5917 \cdot 10^{-25}$ | $4.6376 \cdot 10^{-21}$ | $4.6840 \cdot 10^{-17}$ | $4.7308 \cdot 10^{-13}$ | $4.7781 \cdot 10^{-9}$  |
| 10200 | $3.1165 \cdot 10^{-25}$ | $3.1789 \cdot 10^{-21}$ | $3.2424 \cdot 10^{-17}$ | $3.3073 \cdot 10^{-13}$ | $3.3734 \cdot 10^{-9}$  |
| 10300 | $2.1191 \cdot 10^{-25}$ | $2.1826 \cdot 10^{-21}$ | $2.2481 \cdot 10^{-17}$ | $2.3155 \cdot 10^{-13}$ | $2.3850 \cdot 10^{-9}$  |
| 10400 | $1.4434 \cdot 10^{-25}$ | $1.5011 \cdot 10^{-21}$ | $1.5611 \cdot 10^{-17}$ | $1.6236 \cdot 10^{-13}$ | $1.6885 \cdot 10^{-9}$  |
| 10500 | $9.8478 \cdot 10^{-26}$ | $1.0341 \cdot 10^{-21}$ | $1.0858 \cdot 10^{-17}$ | $1.1401 \cdot 10^{-13}$ | $1.1971 \cdot 10^{-9}$  |
| 10600 | $6.7307 \cdot 10^{-26}$ | $7.1345 \cdot 10^{-22}$ | $7.5626 \cdot 10^{-18}$ | $8.0163 \cdot 10^{-14}$ | $8.4973 \cdot 10^{-10}$ |
| 10700 | $4.6079 \cdot 10^{-26}$ | $4.9305 \cdot 10^{-22}$ | $5.2756 \cdot 10^{-18}$ | $5.6449 \cdot 10^{-14}$ | $6.0400 \cdot 10^{-10}$ |
| 10800 | $3.1599 \cdot 10^{-26}$ | $3.4127 \cdot 10^{-22}$ | $3.6857 \cdot 10^{-18}$ | $3.9805 \cdot 10^{-14}$ | $4.2990 \cdot 10^{-10}$ |
| 10900 | $2.1705 \cdot 10^{-26}$ | $2.3658 \cdot 10^{-22}$ | $2.5787 \cdot 10^{-18}$ | $2.8108 \cdot 10^{-14}$ | $3.0638 \cdot 10^{-10}$ |
| 11000 | $1.4933 \cdot 10^{-26}$ | $1.6426 \cdot 10^{-22}$ | $1.8068 \cdot 10^{-18}$ | $1.9875 \cdot 10^{-14}$ | $2.1862 \cdot 10^{-10}$ |
| 11100 | $1.0290 \cdot 10^{-26}$ | $1.1422 \cdot 10^{-22}$ | $1.2678 \cdot 10^{-18}$ | $1.4073 \cdot 10^{-14}$ | $1.5620 \cdot 10^{-10}$ |
| 11200 | $7.1014 \cdot 10^{-27}$ | $7.9535 \cdot 10^{-23}$ | $8.9079 \cdot 10^{-19}$ | $9.9769 \cdot 10^{-15}$ | $1.1175 \cdot 10^{-10}$ |
| 11300 | $4.9087 \cdot 10^{-27}$ | $5.5469 \cdot 10^{-23}$ | $6.2680 \cdot 10^{-19}$ | $7.0828 \cdot 10^{-15}$ | $8.0035 \cdot 10^{-11}$ |
| 11400 | $3.3983 \cdot 10^{-27}$ | $3.8741 \cdot 10^{-23}$ | $4.4164 \cdot 10^{-19}$ | $5.0347 \cdot 10^{-15}$ | $5.7396 \cdot 10^{-11}$ |
| 11500 | $2.3562 \cdot 10^{-27}$ | $2.7097 \cdot 10^{-23}$ | $3.1161 \cdot 10^{-19}$ | $3.5835 \cdot 10^{-15}$ | $4.1210 \cdot 10^{-11}$ |
| 11600 | $1.6361 \cdot 10^{-27}$ | $1.8979 \cdot 10^{-23}$ | $2.2016 \cdot 10^{-19}$ | $2.5538 \cdot 10^{-15}$ | $2.9624 \cdot 10^{-11}$ |
| 11700 | $1.1378 \cdot 10^{-27}$ | $1.3312 \cdot 10^{-23}$ | $1.5575 \cdot 10^{-19}$ | $1.8223 \cdot 10^{-15}$ | $2.1321 \cdot 10^{-11}$ |
| 11800 | $7.9236 \cdot 10^{-28}$ | $9.3499 \cdot 10^{-24}$ | $1.1033 \cdot 10^{-19}$ | $1.3019 \cdot 10^{-15}$ | $1.5363 \cdot 10^{-11}$ |
| 11900 | $5.5262 \cdot 10^{-28}$ | $6.5762 \cdot 10^{-24}$ | $7.8256 \cdot 10^{-20}$ | $9.3125 \cdot 10^{-16}$ | $1.1082 \cdot 10^{-11}$ |
| 12000 | $3.8597 \cdot 10^{-28}$ | $4.6316 \cdot 10^{-24}$ | $5.5579 \cdot 10^{-20}$ | $6.6694 \cdot 10^{-16}$ | $8.0033 \cdot 10^{-12}$ |
| 12100 | $2.6995 \cdot 10^{-28}$ | $3.2664 \cdot 10^{-24}$ | $3.9523 \cdot 10^{-20}$ | $4.7823 \cdot 10^{-16}$ | $5.7865 \cdot 10^{-12}$ |
| 12200 | $1.8907 \cdot 10^{-28}$ | $2.3066 \cdot 10^{-24}$ | $2.8141 \cdot 10^{-20}$ | $3.4332 \cdot 10^{-16}$ | $4.1884 \cdot 10^{-12}$ |
| 12300 | $1.3260 \cdot 10^{-28}$ | $1.6310 \cdot 10^{-24}$ | $2.0061 \cdot 10^{-20}$ | $2.4675 \cdot 10^{-16}$ | $3.0351 \cdot 10^{-12}$ |
| 12400 | $9.3124 \cdot 10^{-29}$ | $1.1548 \cdot 10^{-24}$ | $1.4319 \cdot 10^{-20}$ | $1.7756 \cdot 10^{-16}$ | $2.2017 \cdot 10^{-12}$ |
| 12500 | $6.5489 \cdot 10^{-29}$ | $8.1861 \cdot 10^{-25}$ | $1.0233 \cdot 10^{-20}$ | $1.2791 \cdot 10^{-16}$ | $1.5989 \cdot 10^{-12}$ |
| 12600 | $4.6116 \cdot 10^{-29}$ | $5.8106 \cdot 10^{-25}$ | $7.3214 \cdot 10^{-21}$ | $9.2249 \cdot 10^{-17}$ | $1.1624 \cdot 10^{-12}$ |
| 12700 | $3.2517 \cdot 10^{-29}$ | $4.1296 \cdot 10^{-25}$ | $5.2446 \cdot 10^{-21}$ | $6.6606 \cdot 10^{-17}$ | $8.4590 \cdot 10^{-13}$ |
| 12800 | $2.2958 \cdot 10^{-29}$ | $2.9385 \cdot 10^{-25}$ | $3.7613 \cdot 10^{-21}$ | $4.8145 \cdot 10^{-17}$ | $6.1625 \cdot 10^{-13}$ |

Continued on next page

Table 9 – continued from previous page

| $b_j$      | $\mathcal{A}_1$         | $\mathcal{A}_2$         | $\mathcal{A}_3$         | $\mathcal{A}_4$         | $\mathcal{A}_5$         |
|------------|-------------------------|-------------------------|-------------------------|-------------------------|-------------------------|
| 12900      | $1.6229 \cdot 10^{-29}$ | $2.0936 \cdot 10^{-25}$ | $2.7007 \cdot 10^{-21}$ | $3.4839 \cdot 10^{-17}$ | $4.4942 \cdot 10^{-13}$ |
| 13000      | $1.1488 \cdot 10^{-29}$ | $1.4934 \cdot 10^{-25}$ | $1.9414 \cdot 10^{-21}$ | $2.5238 \cdot 10^{-17}$ | $3.2809 \cdot 10^{-13}$ |
| 13500      | $2.0792 \cdot 10^{-30}$ | $2.8070 \cdot 10^{-26}$ | $3.7894 \cdot 10^{-22}$ | $5.1157 \cdot 10^{-18}$ | $6.9061 \cdot 10^{-14}$ |
| 13800.7464 | $7.5451 \cdot 10^{-31}$ | $1.0413 \cdot 10^{-26}$ | $1.4371 \cdot 10^{-22}$ | $1.9833 \cdot 10^{-18}$ | $2.7370 \cdot 10^{-14}$ |
| 14000      | $3.8771 \cdot 10^{-31}$ | $5.4279 \cdot 10^{-27}$ | $7.5990 \cdot 10^{-23}$ | $1.0639 \cdot 10^{-18}$ | $1.4894 \cdot 10^{-14}$ |
| 15000      | $1.4652 \cdot 10^{-32}$ | $2.1978 \cdot 10^{-28}$ | $3.2967 \cdot 10^{-24}$ | $4.9450 \cdot 10^{-20}$ | $7.4175 \cdot 10^{-16}$ |
| 16000      | $6.1341 \cdot 10^{-34}$ | $9.8146 \cdot 10^{-30}$ | $1.5704 \cdot 10^{-25}$ | $2.5126 \cdot 10^{-21}$ | $4.0201 \cdot 10^{-17}$ |
| 17000      | $2.8193 \cdot 10^{-35}$ | $4.7928 \cdot 10^{-31}$ | $8.1478 \cdot 10^{-27}$ | $1.3852 \cdot 10^{-22}$ | $2.3547 \cdot 10^{-18}$ |
| 18000      | $1.4115 \cdot 10^{-36}$ | $2.5406 \cdot 10^{-32}$ | $4.5731 \cdot 10^{-28}$ | $8.2315 \cdot 10^{-24}$ | $1.4817 \cdot 10^{-19}$ |
| 19000      | $7.6449 \cdot 10^{-38}$ | $1.4526 \cdot 10^{-33}$ | $2.7599 \cdot 10^{-29}$ | $5.2437 \cdot 10^{-25}$ | $9.9630 \cdot 10^{-21}$ |
| 20000      | $4.4536 \cdot 10^{-39}$ | $8.9071 \cdot 10^{-35}$ | $1.7815 \cdot 10^{-30}$ | $3.5629 \cdot 10^{-26}$ | $7.1257 \cdot 10^{-22}$ |
| 21000      | $2.7759 \cdot 10^{-40}$ | $5.8293 \cdot 10^{-36}$ | $1.2242 \cdot 10^{-31}$ | $2.5708 \cdot 10^{-27}$ | $5.3985 \cdot 10^{-23}$ |
| 22000      | $1.8427 \cdot 10^{-41}$ | $4.0538 \cdot 10^{-37}$ | $8.9184 \cdot 10^{-33}$ | $1.9621 \cdot 10^{-28}$ | $4.3165 \cdot 10^{-24}$ |
| 23000      | $1.2974 \cdot 10^{-42}$ | $2.9839 \cdot 10^{-38}$ | $6.8629 \cdot 10^{-34}$ | $1.5785 \cdot 10^{-29}$ | $3.6305 \cdot 10^{-25}$ |
| 24000      | $9.6521 \cdot 10^{-44}$ | $2.3165 \cdot 10^{-39}$ | $5.5596 \cdot 10^{-35}$ | $1.3344 \cdot 10^{-30}$ | $3.2024 \cdot 10^{-26}$ |
| 25000      | $7.5635 \cdot 10^{-45}$ | $1.8909 \cdot 10^{-40}$ | $4.7272 \cdot 10^{-36}$ | $1.1818 \cdot 10^{-31}$ | $3.0000 \cdot 10^{-27}$ |

4. TABLE 10: SHARPER BOUNDS FOR  $\theta(x)$ :  $x$  IN A MIDDLE RANGE ( $e^{20} \leq x \leq e^{25000}$ )

TABLE 10. Values for  $B_{j,k}$  in  $|\theta(x) - x| < \frac{B_{j,k}x}{(\log x)^k}$  calculated using the method described in Corollary 8.1, Section 3.2. Each  $B_{j,k}$  is valid for  $e^{b_j} \leq x \leq e^{b_{j+1}}$ . The last line is valid for  $e^{24000} \leq x \leq e^{25000}$ .

| $b_j$     | $B_{j,1}$               | $B_{j,2}$              | $B_{j,3}$              | $B_{j,4}$              | $B_{j,5}$              |
|-----------|-------------------------|------------------------|------------------------|------------------------|------------------------|
| 20        | $1.8077 \cdot 10^{-3}$  | $3.6154 \cdot 10^{-2}$ | $7.2309 \cdot 10^{-1}$ | $1.4462 \cdot 10^1$    | $2.9160 \cdot 10^2$    |
| 21        | $1.1458 \cdot 10^{-3}$  | $2.4062 \cdot 10^{-2}$ | $5.0530 \cdot 10^{-1}$ | $1.0611 \cdot 10^1$    | $2.2284 \cdot 10^2$    |
| 22        | $7.2527 \cdot 10^{-4}$  | $1.5956 \cdot 10^{-2}$ | $3.5103 \cdot 10^{-1}$ | $7.7226 \cdot 10^0$    | $1.6990 \cdot 10^2$    |
| 23        | $4.5848 \cdot 10^{-4}$  | $1.0545 \cdot 10^{-2}$ | $2.4254 \cdot 10^{-1}$ | $5.5783 \cdot 10^0$    | $1.2830 \cdot 10^2$    |
| 24        | $2.8945 \cdot 10^{-4}$  | $6.9468 \cdot 10^{-3}$ | $1.6672 \cdot 10^{-1}$ | $4.0013 \cdot 10^0$    | $9.6032 \cdot 10^1$    |
| 25        | $1.8251 \cdot 10^{-4}$  | $4.5626 \cdot 10^{-3}$ | $1.1407 \cdot 10^{-1}$ | $2.8516 \cdot 10^0$    | $7.1291 \cdot 10^1$    |
| 26        | $1.1493 \cdot 10^{-4}$  | $2.9882 \cdot 10^{-3}$ | $7.7694 \cdot 10^{-2}$ | $2.0200 \cdot 10^0$    | $5.2521 \cdot 10^1$    |
| 27        | $7.2293 \cdot 10^{-5}$  | $1.9519 \cdot 10^{-3}$ | $5.2702 \cdot 10^{-2}$ | $1.4229 \cdot 10^0$    | $3.8419 \cdot 10^1$    |
| 28        | $4.5421 \cdot 10^{-5}$  | $1.2718 \cdot 10^{-3}$ | $3.5610 \cdot 10^{-2}$ | $9.9708 \cdot 10^{-1}$ | $2.7918 \cdot 10^1$    |
| 29        | $2.8507 \cdot 10^{-5}$  | $8.2670 \cdot 10^{-4}$ | $2.3974 \cdot 10^{-2}$ | $6.9525 \cdot 10^{-1}$ | $2.0162 \cdot 10^1$    |
| 30        | $1.7873 \cdot 10^{-5}$  | $5.3619 \cdot 10^{-4}$ | $1.6086 \cdot 10^{-2}$ | $4.8257 \cdot 10^{-1}$ | $1.4477 \cdot 10^1$    |
| 31        | $1.1195 \cdot 10^{-5}$  | $3.4704 \cdot 10^{-4}$ | $1.0758 \cdot 10^{-2}$ | $3.3350 \cdot 10^{-1}$ | $1.0339 \cdot 10^1$    |
| 32        | $7.0053 \cdot 10^{-6}$  | $2.2417 \cdot 10^{-4}$ | $7.1734 \cdot 10^{-3}$ | $2.2955 \cdot 10^{-1}$ | $7.3456 \cdot 10^0$    |
| 33        | $4.3798 \cdot 10^{-6}$  | $1.4453 \cdot 10^{-4}$ | $4.7696 \cdot 10^{-3}$ | $1.5740 \cdot 10^{-1}$ | $5.1941 \cdot 10^0$    |
| 34        | $2.7360 \cdot 10^{-6}$  | $9.3023 \cdot 10^{-5}$ | $3.1628 \cdot 10^{-3}$ | $1.0754 \cdot 10^{-1}$ | $3.6562 \cdot 10^0$    |
| 35        | $1.7077 \cdot 10^{-6}$  | $5.9770 \cdot 10^{-5}$ | $2.0920 \cdot 10^{-3}$ | $7.3219 \cdot 10^{-2}$ | $2.5627 \cdot 10^0$    |
| 36        | $1.2459 \cdot 10^{-6}$  | $4.4852 \cdot 10^{-5}$ | $1.6147 \cdot 10^{-3}$ | $5.8128 \cdot 10^{-2}$ | $2.0926 \cdot 10^0$    |
| 37        | $1.0581 \cdot 10^{-6}$  | $3.9148 \cdot 10^{-5}$ | $1.4485 \cdot 10^{-3}$ | $5.3593 \cdot 10^{-2}$ | $1.9830 \cdot 10^0$    |
| 38        | $9.4814 \cdot 10^{-7}$  | $3.6029 \cdot 10^{-5}$ | $1.3691 \cdot 10^{-3}$ | $5.2611 \cdot 10^{-2}$ | $2.0518 \cdot 10^0$    |
| 39        | $8.8692 \cdot 10^{-7}$  | $3.4590 \cdot 10^{-5}$ | $1.3697 \cdot 10^{-3}$ | $5.4788 \cdot 10^{-2}$ | $2.1915 \cdot 10^0$    |
| 40        | $8.5607 \cdot 10^{-7}$  | $3.4611 \cdot 10^{-5}$ | $1.4190 \cdot 10^{-3}$ | $5.8181 \cdot 10^{-2}$ | $2.3854 \cdot 10^0$    |
| 41        | $8.4416 \cdot 10^{-7}$  | $3.5451 \cdot 10^{-5}$ | $1.4889 \cdot 10^{-3}$ | $6.2535 \cdot 10^{-2}$ | $2.6265 \cdot 10^0$    |
| 42        | $8.5132 \cdot 10^{-7}$  | $3.6607 \cdot 10^{-5}$ | $1.5741 \cdot 10^{-3}$ | $6.7686 \cdot 10^{-2}$ | $2.9105 \cdot 10^0$    |
| 43        | $8.5986 \cdot 10^{-7}$  | $3.7618 \cdot 10^{-5}$ | $1.6458 \cdot 10^{-3}$ | $7.2000 \cdot 10^{-2}$ | $3.1500 \cdot 10^0$    |
| 19 log 10 | $8.6315 \cdot 10^{-7}$  | $3.7978 \cdot 10^{-5}$ | $1.6711 \cdot 10^{-3}$ | $7.3526 \cdot 10^{-2}$ | $3.2352 \cdot 10^0$    |
| 44        | $7.8162 \cdot 10^{-7}$  | $3.5173 \cdot 10^{-5}$ | $1.5828 \cdot 10^{-3}$ | $7.1225 \cdot 10^{-2}$ | $3.2052 \cdot 10^0$    |
| 45        | $5.0646 \cdot 10^{-7}$  | $2.3297 \cdot 10^{-5}$ | $1.0717 \cdot 10^{-3}$ | $4.9297 \cdot 10^{-2}$ | $2.2677 \cdot 10^0$    |
| 46        | $3.2935 \cdot 10^{-7}$  | $1.5479 \cdot 10^{-5}$ | $7.2752 \cdot 10^{-4}$ | $3.4194 \cdot 10^{-2}$ | $1.6071 \cdot 10^0$    |
| 47        | $2.1307 \cdot 10^{-7}$  | $1.0228 \cdot 10^{-5}$ | $4.9092 \cdot 10^{-4}$ | $2.3564 \cdot 10^{-2}$ | $1.1311 \cdot 10^0$    |
| 48        | $1.3790 \cdot 10^{-7}$  | $6.7572 \cdot 10^{-6}$ | $3.3110 \cdot 10^{-4}$ | $1.6224 \cdot 10^{-2}$ | $7.9498 \cdot 10^{-1}$ |
| 49        | $8.9139 \cdot 10^{-8}$  | $4.4570 \cdot 10^{-6}$ | $2.2285 \cdot 10^{-4}$ | $1.1142 \cdot 10^{-2}$ | $5.5712 \cdot 10^{-1}$ |
| 50        | $5.7545 \cdot 10^{-8}$  | $2.9348 \cdot 10^{-6}$ | $1.4967 \cdot 10^{-4}$ | $7.6334 \cdot 10^{-3}$ | $3.8930 \cdot 10^{-1}$ |
| 51        | $3.7146 \cdot 10^{-8}$  | $1.9316 \cdot 10^{-6}$ | $1.0044 \cdot 10^{-4}$ | $5.2231 \cdot 10^{-3}$ | $2.7160 \cdot 10^{-1}$ |
| 52        | $2.3898 \cdot 10^{-8}$  | $1.2666 \cdot 10^{-6}$ | $6.7130 \cdot 10^{-5}$ | $3.5579 \cdot 10^{-3}$ | $1.8857 \cdot 10^{-1}$ |
| 53        | $1.5373 \cdot 10^{-8}$  | $8.3012 \cdot 10^{-7}$ | $4.4826 \cdot 10^{-5}$ | $2.4206 \cdot 10^{-3}$ | $1.3071 \cdot 10^{-1}$ |
| 54        | $9.8777 \cdot 10^{-9}$  | $5.4328 \cdot 10^{-7}$ | $2.9880 \cdot 10^{-5}$ | $1.6434 \cdot 10^{-3}$ | $9.0388 \cdot 10^{-2}$ |
| 55        | $6.3417 \cdot 10^{-9}$  | $3.5514 \cdot 10^{-7}$ | $1.9888 \cdot 10^{-5}$ | $1.1137 \cdot 10^{-3}$ | $6.2367 \cdot 10^{-2}$ |
| 56        | $4.0668 \cdot 10^{-9}$  | $2.3181 \cdot 10^{-7}$ | $1.3213 \cdot 10^{-5}$ | $7.5315 \cdot 10^{-4}$ | $4.2929 \cdot 10^{-2}$ |
| 57        | $2.6047 \cdot 10^{-9}$  | $1.5107 \cdot 10^{-7}$ | $8.7623 \cdot 10^{-6}$ | $5.0821 \cdot 10^{-4}$ | $2.9476 \cdot 10^{-2}$ |
| 58        | $1.6805 \cdot 10^{-9}$  | $9.9147 \cdot 10^{-8}$ | $5.8497 \cdot 10^{-6}$ | $3.4513 \cdot 10^{-4}$ | $2.0363 \cdot 10^{-2}$ |
| 59        | $1.1120 \cdot 10^{-9}$  | $6.6721 \cdot 10^{-8}$ | $4.0033 \cdot 10^{-6}$ | $2.4020 \cdot 10^{-4}$ | $1.4412 \cdot 10^{-2}$ |
| 60        | $7.9446 \cdot 10^{-10}$ | $5.1640 \cdot 10^{-8}$ | $3.3566 \cdot 10^{-6}$ | $2.1818 \cdot 10^{-4}$ | $1.4182 \cdot 10^{-2}$ |
| 65        | $2.5003 \cdot 10^{-10}$ | $1.7502 \cdot 10^{-8}$ | $1.2252 \cdot 10^{-6}$ | $8.5761 \cdot 10^{-5}$ | $6.0033 \cdot 10^{-3}$ |
| 70        | $2.0943 \cdot 10^{-10}$ | $1.5707 \cdot 10^{-8}$ | $1.1780 \cdot 10^{-6}$ | $8.8353 \cdot 10^{-5}$ | $6.6265 \cdot 10^{-3}$ |
| 75        | $2.1629 \cdot 10^{-10}$ | $1.7303 \cdot 10^{-8}$ | $1.3842 \cdot 10^{-6}$ | $1.1074 \cdot 10^{-4}$ | $8.8591 \cdot 10^{-3}$ |
| 80        | $2.2192 \cdot 10^{-10}$ | $1.8863 \cdot 10^{-8}$ | $1.6034 \cdot 10^{-6}$ | $1.3629 \cdot 10^{-4}$ | $1.1584 \cdot 10^{-2}$ |
| 85        | $2.3123 \cdot 10^{-10}$ | $2.0811 \cdot 10^{-8}$ | $1.8730 \cdot 10^{-6}$ | $1.6857 \cdot 10^{-4}$ | $1.5171 \cdot 10^{-2}$ |

Continued on next page

Table 10 – continued from previous page

| $b_j$ | $B_{j,1}$               | $B_{j,2}$              | $B_{j,3}$              | $B_{j,4}$              | $B_{j,5}$              |
|-------|-------------------------|------------------------|------------------------|------------------------|------------------------|
| 90    | $2.3952 \cdot 10^{-10}$ | $2.2755 \cdot 10^{-8}$ | $2.1617 \cdot 10^{-6}$ | $2.0536 \cdot 10^{-4}$ | $1.9509 \cdot 10^{-2}$ |
| 95    | $2.4919 \cdot 10^{-10}$ | $2.4919 \cdot 10^{-8}$ | $2.4919 \cdot 10^{-6}$ | $2.4919 \cdot 10^{-4}$ | $2.4919 \cdot 10^{-2}$ |
| 100   | $4.9060 \cdot 10^{-10}$ | $9.8120 \cdot 10^{-8}$ | $1.9624 \cdot 10^{-5}$ | $3.9248 \cdot 10^{-3}$ | $7.8496 \cdot 10^{-1}$ |
| 200   | $6.5446 \cdot 10^{-10}$ | $1.9634 \cdot 10^{-7}$ | $5.8902 \cdot 10^{-5}$ | $1.7671 \cdot 10^{-2}$ | $5.3012 \cdot 10^0$    |
| 300   | $8.3609 \cdot 10^{-10}$ | $3.3444 \cdot 10^{-7}$ | $1.3378 \cdot 10^{-4}$ | $5.3510 \cdot 10^{-2}$ | $2.1404 \cdot 10^1$    |
| 400   | $1.0199 \cdot 10^{-9}$  | $5.0995 \cdot 10^{-7}$ | $2.5498 \cdot 10^{-4}$ | $1.2749 \cdot 10^{-1}$ | $6.3744 \cdot 10^1$    |
| 500   | $1.1999 \cdot 10^{-9}$  | $7.1995 \cdot 10^{-7}$ | $4.3197 \cdot 10^{-4}$ | $2.5918 \cdot 10^{-1}$ | $1.5551 \cdot 10^2$    |
| 600   | $1.3923 \cdot 10^{-9}$  | $9.7458 \cdot 10^{-7}$ | $6.8221 \cdot 10^{-4}$ | $4.7755 \cdot 10^{-1}$ | $3.3428 \cdot 10^2$    |
| 700   | $1.5812 \cdot 10^{-9}$  | $1.2649 \cdot 10^{-6}$ | $1.0119 \cdot 10^{-3}$ | $8.0955 \cdot 10^{-1}$ | $6.4764 \cdot 10^2$    |
| 800   | $1.7704 \cdot 10^{-9}$  | $1.5934 \cdot 10^{-6}$ | $1.4340 \cdot 10^{-3}$ | $1.2906 \cdot 10^0$    | $1.1616 \cdot 10^3$    |
| 900   | $1.9599 \cdot 10^{-9}$  | $1.9599 \cdot 10^{-6}$ | $1.9599 \cdot 10^{-3}$ | $1.9599 \cdot 10^0$    | $1.9599 \cdot 10^3$    |
| 1000  | $2.9213 \cdot 10^{-9}$  | $4.3819 \cdot 10^{-6}$ | $6.5729 \cdot 10^{-3}$ | $9.8593 \cdot 10^0$    | $1.4789 \cdot 10^4$    |
| 1500  | $3.0988 \cdot 10^{-9}$  | $4.9581 \cdot 10^{-6}$ | $7.9330 \cdot 10^{-3}$ | $1.2693 \cdot 10^1$    | $2.0309 \cdot 10^4$    |
| 1600  | $3.2797 \cdot 10^{-9}$  | $5.5755 \cdot 10^{-6}$ | $9.4783 \cdot 10^{-3}$ | $1.6113 \cdot 10^1$    | $2.7392 \cdot 10^4$    |
| 1700  | $3.3247 \cdot 10^{-9}$  | $5.7350 \cdot 10^{-6}$ | $9.8929 \cdot 10^{-3}$ | $1.7065 \cdot 10^1$    | $2.9438 \cdot 10^4$    |
| 1725  | $3.3721 \cdot 10^{-9}$  | $5.9011 \cdot 10^{-6}$ | $1.0327 \cdot 10^{-2}$ | $1.8072 \cdot 10^1$    | $3.1626 \cdot 10^4$    |
| 1750  | $3.4195 \cdot 10^{-9}$  | $6.0696 \cdot 10^{-6}$ | $1.0774 \cdot 10^{-2}$ | $1.9123 \cdot 10^1$    | $3.3943 \cdot 10^4$    |
| 1775  | $3.4669 \cdot 10^{-9}$  | $6.2404 \cdot 10^{-6}$ | $1.1233 \cdot 10^{-2}$ | $2.0219 \cdot 10^1$    | $3.6394 \cdot 10^4$    |
| 1800  | $3.5143 \cdot 10^{-9}$  | $6.4136 \cdot 10^{-6}$ | $1.1705 \cdot 10^{-2}$ | $2.1361 \cdot 10^1$    | $3.8984 \cdot 10^4$    |
| 1825  | $3.5617 \cdot 10^{-9}$  | $6.5892 \cdot 10^{-6}$ | $1.2190 \cdot 10^{-2}$ | $2.2552 \cdot 10^1$    | $4.1720 \cdot 10^4$    |
| 1850  | $3.6091 \cdot 10^{-9}$  | $6.7671 \cdot 10^{-6}$ | $1.2688 \cdot 10^{-2}$ | $2.3791 \cdot 10^1$    | $4.4608 \cdot 10^4$    |
| 1875  | $3.6566 \cdot 10^{-9}$  | $6.9475 \cdot 10^{-6}$ | $1.3200 \cdot 10^{-2}$ | $2.5080 \cdot 10^1$    | $4.7653 \cdot 10^4$    |
| 1900  | $3.7040 \cdot 10^{-9}$  | $7.1302 \cdot 10^{-6}$ | $1.3726 \cdot 10^{-2}$ | $2.6422 \cdot 10^1$    | $5.0862 \cdot 10^4$    |
| 1925  | $3.7514 \cdot 10^{-9}$  | $7.3152 \cdot 10^{-6}$ | $1.4265 \cdot 10^{-2}$ | $2.7816 \cdot 10^1$    | $5.4241 \cdot 10^4$    |
| 1950  | $3.7988 \cdot 10^{-9}$  | $7.5026 \cdot 10^{-6}$ | $1.4818 \cdot 10^{-2}$ | $2.9265 \cdot 10^1$    | $5.7798 \cdot 10^4$    |
| 1975  | $3.8462 \cdot 10^{-9}$  | $7.6924 \cdot 10^{-6}$ | $1.5385 \cdot 10^{-2}$ | $3.0770 \cdot 10^1$    | $6.1540 \cdot 10^4$    |
| 2000  | $3.8937 \cdot 10^{-9}$  | $7.8847 \cdot 10^{-6}$ | $1.5966 \cdot 10^{-2}$ | $3.2332 \cdot 10^1$    | $6.5472 \cdot 10^4$    |
| 2025  | $3.9411 \cdot 10^{-9}$  | $8.0792 \cdot 10^{-6}$ | $1.6562 \cdot 10^{-2}$ | $3.3953 \cdot 10^1$    | $6.9603 \cdot 10^4$    |
| 2050  | $3.9885 \cdot 10^{-9}$  | $8.2761 \cdot 10^{-6}$ | $1.7173 \cdot 10^{-2}$ | $3.5634 \cdot 10^1$    | $7.3940 \cdot 10^4$    |
| 2075  | $4.0359 \cdot 10^{-9}$  | $8.4754 \cdot 10^{-6}$ | $1.7798 \cdot 10^{-2}$ | $3.7377 \cdot 10^1$    | $7.8491 \cdot 10^4$    |
| 2100  | $4.0833 \cdot 10^{-9}$  | $8.6771 \cdot 10^{-6}$ | $1.8439 \cdot 10^{-2}$ | $3.9182 \cdot 10^1$    | $8.3262 \cdot 10^4$    |
| 2125  | $4.1308 \cdot 10^{-9}$  | $8.8811 \cdot 10^{-6}$ | $1.9095 \cdot 10^{-2}$ | $4.1053 \cdot 10^1$    | $8.8264 \cdot 10^4$    |
| 2150  | $4.1782 \cdot 10^{-9}$  | $9.0875 \cdot 10^{-6}$ | $1.9765 \cdot 10^{-2}$ | $4.2990 \cdot 10^1$    | $9.3503 \cdot 10^4$    |
| 2175  | $4.2256 \cdot 10^{-9}$  | $9.2963 \cdot 10^{-6}$ | $2.0452 \cdot 10^{-2}$ | $4.4994 \cdot 10^1$    | $9.8987 \cdot 10^4$    |
| 2200  | $4.2730 \cdot 10^{-9}$  | $9.5075 \cdot 10^{-6}$ | $2.1154 \cdot 10^{-2}$ | $4.7068 \cdot 10^1$    | $1.0473 \cdot 10^5$    |
| 2225  | $4.3204 \cdot 10^{-9}$  | $9.7210 \cdot 10^{-6}$ | $2.1872 \cdot 10^{-2}$ | $4.9212 \cdot 10^1$    | $1.1073 \cdot 10^5$    |
| 2250  | $4.3679 \cdot 10^{-9}$  | $9.9369 \cdot 10^{-6}$ | $2.2607 \cdot 10^{-2}$ | $5.1430 \cdot 10^1$    | $1.1700 \cdot 10^5$    |
| 2275  | $4.4153 \cdot 10^{-9}$  | $1.0155 \cdot 10^{-5}$ | $2.3357 \cdot 10^{-2}$ | $5.3721 \cdot 10^1$    | $1.2356 \cdot 10^5$    |
| 2300  | $4.4627 \cdot 10^{-9}$  | $1.0376 \cdot 10^{-5}$ | $2.4124 \cdot 10^{-2}$ | $5.6088 \cdot 10^1$    | $1.3040 \cdot 10^5$    |
| 2325  | $4.4062 \cdot 10^{-9}$  | $1.0355 \cdot 10^{-5}$ | $2.4333 \cdot 10^{-2}$ | $5.7184 \cdot 10^1$    | $1.3438 \cdot 10^5$    |
| 2350  | $4.2245 \cdot 10^{-9}$  | $1.0033 \cdot 10^{-5}$ | $2.3829 \cdot 10^{-2}$ | $5.6593 \cdot 10^1$    | $1.3441 \cdot 10^5$    |
| 2375  | $4.0498 \cdot 10^{-9}$  | $9.7196 \cdot 10^{-6}$ | $2.3327 \cdot 10^{-2}$ | $5.5985 \cdot 10^1$    | $1.3436 \cdot 10^5$    |
| 2400  | $3.8820 \cdot 10^{-9}$  | $9.4139 \cdot 10^{-6}$ | $2.2829 \cdot 10^{-2}$ | $5.5360 \cdot 10^1$    | $1.3425 \cdot 10^5$    |
| 2425  | $3.4832 \cdot 10^{-9}$  | $8.5339 \cdot 10^{-6}$ | $2.0908 \cdot 10^{-2}$ | $5.1225 \cdot 10^1$    | $1.2550 \cdot 10^5$    |
| 2450  | $3.0228 \cdot 10^{-9}$  | $7.4814 \cdot 10^{-6}$ | $1.8517 \cdot 10^{-2}$ | $4.5828 \cdot 10^1$    | $1.1343 \cdot 10^5$    |
| 2475  | $2.6278 \cdot 10^{-9}$  | $6.5696 \cdot 10^{-6}$ | $1.6424 \cdot 10^{-2}$ | $4.1060 \cdot 10^1$    | $1.0265 \cdot 10^5$    |
| 2500  | $2.2884 \cdot 10^{-9}$  | $5.7783 \cdot 10^{-6}$ | $1.4590 \cdot 10^{-2}$ | $3.6840 \cdot 10^1$    | $9.3021 \cdot 10^4$    |
| 2525  | $1.9873 \cdot 10^{-9}$  | $5.0676 \cdot 10^{-6}$ | $1.2922 \cdot 10^{-2}$ | $3.2952 \cdot 10^1$    | $8.4027 \cdot 10^4$    |
| 2550  | $1.7270 \cdot 10^{-9}$  | $4.4470 \cdot 10^{-6}$ | $1.1451 \cdot 10^{-2}$ | $2.9487 \cdot 10^1$    | $7.5928 \cdot 10^4$    |
| 2575  | $1.4992 \cdot 10^{-9}$  | $3.8979 \cdot 10^{-6}$ | $1.0135 \cdot 10^{-2}$ | $2.6350 \cdot 10^1$    | $6.8509 \cdot 10^4$    |
| 2600  | $1.3022 \cdot 10^{-9}$  | $3.4184 \cdot 10^{-6}$ | $8.9732 \cdot 10^{-3}$ | $2.3555 \cdot 10^1$    | $6.1831 \cdot 10^4$    |
| 2625  | $1.1314 \cdot 10^{-9}$  | $2.9981 \cdot 10^{-6}$ | $7.9449 \cdot 10^{-3}$ | $2.1054 \cdot 10^1$    | $5.5793 \cdot 10^4$    |
| 2650  | $9.8296 \cdot 10^{-10}$ | $2.6294 \cdot 10^{-6}$ | $7.0337 \cdot 10^{-3}$ | $1.8815 \cdot 10^1$    | $5.0330 \cdot 10^4$    |
| 2675  | $8.5431 \cdot 10^{-10}$ | $2.3067 \cdot 10^{-6}$ | $6.2279 \cdot 10^{-3}$ | $1.6816 \cdot 10^1$    | $4.5402 \cdot 10^4$    |
| 2700  | $7.4234 \cdot 10^{-10}$ | $2.0229 \cdot 10^{-6}$ | $5.5123 \cdot 10^{-3}$ | $1.5021 \cdot 10^1$    | $4.0932 \cdot 10^4$    |

Continued on next page

Table 10 – continued from previous page

| $b_j$ | $B_{j,1}$               | $B_{j,2}$              | $B_{j,3}$              | $B_{j,4}$              | $B_{j,5}$           |
|-------|-------------------------|------------------------|------------------------|------------------------|---------------------|
| 2725  | $6.4498 \cdot 10^{-10}$ | $1.7737 \cdot 10^{-6}$ | $4.8777 \cdot 10^{-3}$ | $1.3414 \cdot 10^1$    | $3.6887 \cdot 10^4$ |
| 2750  | $5.6071 \cdot 10^{-10}$ | $1.5560 \cdot 10^{-6}$ | $4.3178 \cdot 10^{-3}$ | $1.1982 \cdot 10^1$    | $3.3250 \cdot 10^4$ |
| 2775  | $4.8730 \cdot 10^{-10}$ | $1.3644 \cdot 10^{-6}$ | $3.8204 \cdot 10^{-3}$ | $1.0697 \cdot 10^1$    | $2.9952 \cdot 10^4$ |
| 2800  | $4.2388 \cdot 10^{-10}$ | $1.1975 \cdot 10^{-6}$ | $3.3829 \cdot 10^{-3}$ | $9.5565 \cdot 10^0$    | $2.6997 \cdot 10^4$ |
| 2825  | $3.6911 \cdot 10^{-10}$ | $1.0520 \cdot 10^{-6}$ | $2.9981 \cdot 10^{-3}$ | $8.5446 \cdot 10^0$    | $2.4352 \cdot 10^4$ |
| 2850  | $3.2167 \cdot 10^{-10}$ | $9.2481 \cdot 10^{-7}$ | $2.6588 \cdot 10^{-3}$ | $7.6442 \cdot 10^0$    | $2.1977 \cdot 10^4$ |
| 2875  | $2.7953 \cdot 10^{-10}$ | $8.1062 \cdot 10^{-7}$ | $2.3508 \cdot 10^{-3}$ | $6.8173 \cdot 10^0$    | $1.9770 \cdot 10^4$ |
| 2900  | $2.4326 \cdot 10^{-10}$ | $7.1154 \cdot 10^{-7}$ | $2.0813 \cdot 10^{-3}$ | $6.0877 \cdot 10^0$    | $1.7806 \cdot 10^4$ |
| 2925  | $2.1140 \cdot 10^{-10}$ | $6.2363 \cdot 10^{-7}$ | $1.8397 \cdot 10^{-3}$ | $5.4272 \cdot 10^0$    | $1.6010 \cdot 10^4$ |
| 2950  | $1.8391 \cdot 10^{-10}$ | $5.4712 \cdot 10^{-7}$ | $1.6277 \cdot 10^{-3}$ | $4.8423 \cdot 10^0$    | $1.4406 \cdot 10^4$ |
| 2975  | $1.6015 \cdot 10^{-10}$ | $4.8044 \cdot 10^{-7}$ | $1.4413 \cdot 10^{-3}$ | $4.3240 \cdot 10^0$    | $1.2972 \cdot 10^4$ |
| 3000  | $1.3914 \cdot 10^{-10}$ | $4.2090 \cdot 10^{-7}$ | $1.2732 \cdot 10^{-3}$ | $3.8515 \cdot 10^0$    | $1.1651 \cdot 10^4$ |
| 3025  | $1.2115 \cdot 10^{-10}$ | $3.6949 \cdot 10^{-7}$ | $1.1270 \cdot 10^{-3}$ | $3.4372 \cdot 10^0$    | $1.0484 \cdot 10^4$ |
| 3050  | $1.0531 \cdot 10^{-10}$ | $3.2382 \cdot 10^{-7}$ | $9.9573 \cdot 10^{-4}$ | $3.0619 \cdot 10^0$    | $9.4152 \cdot 10^3$ |
| 3075  | $9.1684 \cdot 10^{-11}$ | $2.8422 \cdot 10^{-7}$ | $8.8108 \cdot 10^{-4}$ | $2.7314 \cdot 10^0$    | $8.4672 \cdot 10^3$ |
| 3100  | $7.9793 \cdot 10^{-11}$ | $2.4935 \cdot 10^{-7}$ | $7.7922 \cdot 10^{-4}$ | $2.4351 \cdot 10^0$    | $7.6096 \cdot 10^3$ |
| 3125  | $6.9396 \cdot 10^{-11}$ | $2.1860 \cdot 10^{-7}$ | $6.8858 \cdot 10^{-4}$ | $2.1690 \cdot 10^0$    | $6.8325 \cdot 10^3$ |
| 3150  | $6.0410 \cdot 10^{-11}$ | $1.9180 \cdot 10^{-7}$ | $6.0897 \cdot 10^{-4}$ | $1.9335 \cdot 10^0$    | $6.1388 \cdot 10^3$ |
| 3175  | $5.2572 \cdot 10^{-11}$ | $1.6823 \cdot 10^{-7}$ | $5.3834 \cdot 10^{-4}$ | $1.7227 \cdot 10^0$    | $5.5126 \cdot 10^3$ |
| 3200  | $4.5782 \cdot 10^{-11}$ | $1.4765 \cdot 10^{-7}$ | $4.7616 \cdot 10^{-4}$ | $1.5356 \cdot 10^0$    | $4.9524 \cdot 10^3$ |
| 3225  | $3.9901 \cdot 10^{-11}$ | $1.2968 \cdot 10^{-7}$ | $4.2146 \cdot 10^{-4}$ | $1.3697 \cdot 10^0$    | $4.4516 \cdot 10^3$ |
| 3250  | $3.4800 \cdot 10^{-11}$ | $1.1397 \cdot 10^{-7}$ | $3.7326 \cdot 10^{-4}$ | $1.2224 \cdot 10^0$    | $4.0034 \cdot 10^3$ |
| 3275  | $3.0332 \cdot 10^{-11}$ | $1.0009 \cdot 10^{-7}$ | $3.3031 \cdot 10^{-4}$ | $1.0900 \cdot 10^0$    | $3.5971 \cdot 10^3$ |
| 3300  | $2.6412 \cdot 10^{-11}$ | $8.7820 \cdot 10^{-8}$ | $2.9200 \cdot 10^{-4}$ | $9.7090 \cdot 10^{-1}$ | $3.2283 \cdot 10^3$ |
| 3325  | $2.3015 \cdot 10^{-11}$ | $7.7100 \cdot 10^{-8}$ | $2.5829 \cdot 10^{-4}$ | $8.6525 \cdot 10^{-1}$ | $2.8986 \cdot 10^3$ |
| 3350  | $2.0043 \cdot 10^{-11}$ | $6.7644 \cdot 10^{-8}$ | $2.2830 \cdot 10^{-4}$ | $7.7051 \cdot 10^{-1}$ | $2.6005 \cdot 10^3$ |
| 3375  | $1.7453 \cdot 10^{-11}$ | $5.9340 \cdot 10^{-8}$ | $2.0176 \cdot 10^{-4}$ | $6.8597 \cdot 10^{-1}$ | $2.3323 \cdot 10^3$ |
| 3400  | $1.5212 \cdot 10^{-11}$ | $5.2099 \cdot 10^{-8}$ | $1.7844 \cdot 10^{-4}$ | $6.1116 \cdot 10^{-1}$ | $2.0932 \cdot 10^3$ |
| 3425  | $1.3266 \cdot 10^{-11}$ | $4.5768 \cdot 10^{-8}$ | $1.5790 \cdot 10^{-4}$ | $5.4476 \cdot 10^{-1}$ | $1.8794 \cdot 10^3$ |
| 3450  | $1.1554 \cdot 10^{-11}$ | $4.0151 \cdot 10^{-8}$ | $1.3953 \cdot 10^{-4}$ | $4.8485 \cdot 10^{-1}$ | $1.6849 \cdot 10^3$ |
| 3475  | $1.0059 \cdot 10^{-11}$ | $3.5206 \cdot 10^{-8}$ | $1.2322 \cdot 10^{-4}$ | $4.3127 \cdot 10^{-1}$ | $1.5095 \cdot 10^3$ |
| 3500  | $8.7646 \cdot 10^{-12}$ | $3.0895 \cdot 10^{-8}$ | $1.0891 \cdot 10^{-4}$ | $3.8389 \cdot 10^{-1}$ | $1.3532 \cdot 10^3$ |
| 3525  | $7.6403 \cdot 10^{-12}$ | $2.7123 \cdot 10^{-8}$ | $9.6287 \cdot 10^{-5}$ | $3.4182 \cdot 10^{-1}$ | $1.2135 \cdot 10^3$ |
| 3550  | $6.6608 \cdot 10^{-12}$ | $2.3812 \cdot 10^{-8}$ | $8.5129 \cdot 10^{-5}$ | $3.0434 \cdot 10^{-1}$ | $1.0880 \cdot 10^3$ |
| 3575  | $5.8042 \cdot 10^{-12}$ | $2.0895 \cdot 10^{-8}$ | $7.5222 \cdot 10^{-5}$ | $2.7080 \cdot 10^{-1}$ | $9.7488 \cdot 10^2$ |
| 3600  | $5.0621 \cdot 10^{-12}$ | $1.8350 \cdot 10^{-8}$ | $6.6520 \cdot 10^{-5}$ | $2.4113 \cdot 10^{-1}$ | $8.7411 \cdot 10^2$ |
| 3625  | $4.4165 \cdot 10^{-12}$ | $1.6120 \cdot 10^{-8}$ | $5.8839 \cdot 10^{-5}$ | $2.1476 \cdot 10^{-1}$ | $7.8388 \cdot 10^2$ |
| 3650  | $3.8475 \cdot 10^{-12}$ | $1.4140 \cdot 10^{-8}$ | $5.1963 \cdot 10^{-5}$ | $1.9096 \cdot 10^{-1}$ | $7.0179 \cdot 10^2$ |
| 3675  | $3.3560 \cdot 10^{-12}$ | $1.2417 \cdot 10^{-8}$ | $4.5944 \cdot 10^{-5}$ | $1.6999 \cdot 10^{-1}$ | $6.2897 \cdot 10^2$ |
| 3700  | $2.9296 \cdot 10^{-12}$ | $1.0913 \cdot 10^{-8}$ | $4.0649 \cdot 10^{-5}$ | $1.5142 \cdot 10^{-1}$ | $5.6404 \cdot 10^2$ |
| 3725  | $2.5580 \cdot 10^{-12}$ | $9.5924 \cdot 10^{-9}$ | $3.5971 \cdot 10^{-5}$ | $1.3489 \cdot 10^{-1}$ | $5.0585 \cdot 10^2$ |
| 3750  | $2.2346 \cdot 10^{-12}$ | $8.4357 \cdot 10^{-9}$ | $3.1845 \cdot 10^{-5}$ | $1.2022 \cdot 10^{-1}$ | $4.5381 \cdot 10^2$ |
| 3775  | $1.9513 \cdot 10^{-12}$ | $7.4151 \cdot 10^{-9}$ | $2.8177 \cdot 10^{-5}$ | $1.0707 \cdot 10^{-1}$ | $4.0688 \cdot 10^2$ |
| 3800  | $1.7020 \cdot 10^{-12}$ | $6.5099 \cdot 10^{-9}$ | $2.4901 \cdot 10^{-5}$ | $9.5244 \cdot 10^{-2}$ | $3.6431 \cdot 10^2$ |
| 3825  | $1.4854 \cdot 10^{-12}$ | $5.7189 \cdot 10^{-9}$ | $2.2018 \cdot 10^{-5}$ | $8.4768 \cdot 10^{-2}$ | $3.2636 \cdot 10^2$ |
| 3850  | $1.2972 \cdot 10^{-12}$ | $5.0267 \cdot 10^{-9}$ | $1.9478 \cdot 10^{-5}$ | $7.5479 \cdot 10^{-2}$ | $2.9248 \cdot 10^2$ |
| 3875  | $1.1314 \cdot 10^{-12}$ | $4.4124 \cdot 10^{-9}$ | $1.7208 \cdot 10^{-5}$ | $6.7112 \cdot 10^{-2}$ | $2.6174 \cdot 10^2$ |
| 3900  | $9.8800 \cdot 10^{-13}$ | $3.8779 \cdot 10^{-9}$ | $1.5221 \cdot 10^{-5}$ | $5.9741 \cdot 10^{-2}$ | $2.3449 \cdot 10^2$ |
| 3925  | $8.6323 \cdot 10^{-13}$ | $3.4098 \cdot 10^{-9}$ | $1.3469 \cdot 10^{-5}$ | $5.3201 \cdot 10^{-2}$ | $2.1014 \cdot 10^2$ |
| 3950  | $7.5449 \cdot 10^{-13}$ | $2.9991 \cdot 10^{-9}$ | $1.1922 \cdot 10^{-5}$ | $4.7388 \cdot 10^{-2}$ | $1.8837 \cdot 10^2$ |
| 3975  | $6.5788 \cdot 10^{-13}$ | $2.6315 \cdot 10^{-9}$ | $1.0526 \cdot 10^{-5}$ | $4.2104 \cdot 10^{-2}$ | $1.6842 \cdot 10^2$ |
| 4000  | $5.7409 \cdot 10^{-13}$ | $2.3107 \cdot 10^{-9}$ | $9.3007 \cdot 10^{-6}$ | $3.7435 \cdot 10^{-2}$ | $1.5068 \cdot 10^2$ |
| 4025  | $5.0264 \cdot 10^{-13}$ | $2.0357 \cdot 10^{-9}$ | $8.2446 \cdot 10^{-6}$ | $3.3391 \cdot 10^{-2}$ | $1.3523 \cdot 10^2$ |
| 4050  | $4.3803 \cdot 10^{-13}$ | $1.7850 \cdot 10^{-9}$ | $7.2737 \cdot 10^{-6}$ | $2.9640 \cdot 10^{-2}$ | $1.2078 \cdot 10^2$ |
| 4075  | $3.8285 \cdot 10^{-13}$ | $1.5697 \cdot 10^{-9}$ | $6.4356 \cdot 10^{-6}$ | $2.6386 \cdot 10^{-2}$ | $1.0818 \cdot 10^2$ |

Continued on next page

Table 10 – continued from previous page

| $b_j$ | $B_{j,1}$               | $B_{j,2}$               | $B_{j,3}$               | $B_{j,4}$              | $B_{j,5}$              |
|-------|-------------------------|-------------------------|-------------------------|------------------------|------------------------|
| 4100  | $3.3428 \cdot 10^{-13}$ | $1.3789 \cdot 10^{-9}$  | $5.6879 \cdot 10^{-6}$  | $2.3463 \cdot 10^{-2}$ | $9.6783 \cdot 10^1$    |
| 4125  | $2.9206 \cdot 10^{-13}$ | $1.2120 \cdot 10^{-9}$  | $5.0299 \cdot 10^{-6}$  | $2.0874 \cdot 10^{-2}$ | $8.6628 \cdot 10^1$    |
| 4150  | $2.5566 \cdot 10^{-13}$ | $1.0674 \cdot 10^{-9}$  | $4.4563 \cdot 10^{-6}$  | $1.8605 \cdot 10^{-2}$ | $7.7676 \cdot 10^1$    |
| 4175  | $2.2309 \cdot 10^{-13}$ | $9.3698 \cdot 10^{-10}$ | $3.9353 \cdot 10^{-6}$  | $1.6528 \cdot 10^{-2}$ | $6.9419 \cdot 10^1$    |
| 4200  | $1.9496 \cdot 10^{-13}$ | $8.2370 \cdot 10^{-10}$ | $3.4801 \cdot 10^{-6}$  | $1.4704 \cdot 10^{-2}$ | $6.2122 \cdot 10^1$    |
| 4225  | $1.7047 \cdot 10^{-13}$ | $7.2449 \cdot 10^{-10}$ | $3.0791 \cdot 10^{-6}$  | $1.3086 \cdot 10^{-2}$ | $5.5616 \cdot 10^1$    |
| 4250  | $1.4913 \cdot 10^{-13}$ | $6.3751 \cdot 10^{-10}$ | $2.7254 \cdot 10^{-6}$  | $1.1651 \cdot 10^{-2}$ | $4.9808 \cdot 10^1$    |
| 4275  | $1.3036 \cdot 10^{-13}$ | $5.6056 \cdot 10^{-10}$ | $2.4104 \cdot 10^{-6}$  | $1.0365 \cdot 10^{-2}$ | $4.4568 \cdot 10^1$    |
| 4300  | $1.1396 \cdot 10^{-13}$ | $4.9288 \cdot 10^{-10}$ | $2.1317 \cdot 10^{-6}$  | $9.2195 \cdot 10^{-3}$ | $3.9875 \cdot 10^1$    |
| 4325  | $9.9670 \cdot 10^{-14}$ | $4.3356 \cdot 10^{-10}$ | $1.8860 \cdot 10^{-6}$  | $8.2041 \cdot 10^{-3}$ | $3.5688 \cdot 10^1$    |
| 4350  | $8.7210 \cdot 10^{-14}$ | $3.8154 \cdot 10^{-10}$ | $1.6693 \cdot 10^{-6}$  | $7.3030 \cdot 10^{-3}$ | $3.1951 \cdot 10^1$    |
| 4375  | $7.6274 \cdot 10^{-14}$ | $3.3561 \cdot 10^{-10}$ | $1.4767 \cdot 10^{-6}$  | $6.4973 \cdot 10^{-3}$ | $2.8588 \cdot 10^1$    |
| 4400  | $6.6744 \cdot 10^{-14}$ | $2.9534 \cdot 10^{-10}$ | $1.3069 \cdot 10^{-6}$  | $5.7829 \cdot 10^{-3}$ | $2.5590 \cdot 10^1$    |
| 4425  | $5.8436 \cdot 10^{-14}$ | $2.6004 \cdot 10^{-10}$ | $1.1572 \cdot 10^{-6}$  | $5.1495 \cdot 10^{-3}$ | $2.2915 \cdot 10^1$    |
| 4450  | $5.1174 \cdot 10^{-14}$ | $2.2901 \cdot 10^{-10}$ | $1.0248 \cdot 10^{-6}$  | $4.5860 \cdot 10^{-3}$ | $2.0522 \cdot 10^1$    |
| 4475  | $4.4832 \cdot 10^{-14}$ | $2.0174 \cdot 10^{-10}$ | $9.0785 \cdot 10^{-7}$  | $4.0853 \cdot 10^{-3}$ | $1.8384 \cdot 10^1$    |
| 4500  | $3.9290 \cdot 10^{-14}$ | $1.7779 \cdot 10^{-10}$ | $8.0450 \cdot 10^{-7}$  | $3.6403 \cdot 10^{-3}$ | $1.6473 \cdot 10^1$    |
| 4525  | $3.4446 \cdot 10^{-14}$ | $1.5673 \cdot 10^{-10}$ | $7.1312 \cdot 10^{-7}$  | $3.2447 \cdot 10^{-3}$ | $1.4763 \cdot 10^1$    |
| 4550  | $3.0155 \cdot 10^{-14}$ | $1.3796 \cdot 10^{-10}$ | $6.3117 \cdot 10^{-7}$  | $2.8876 \cdot 10^{-3}$ | $1.3211 \cdot 10^1$    |
| 4575  | $2.6404 \cdot 10^{-14}$ | $1.2146 \cdot 10^{-10}$ | $5.5870 \cdot 10^{-7}$  | $2.5700 \cdot 10^{-3}$ | $1.1822 \cdot 10^1$    |
| 4600  | $2.3157 \cdot 10^{-14}$ | $1.0710 \cdot 10^{-10}$ | $4.9535 \cdot 10^{-7}$  | $2.2910 \cdot 10^{-3}$ | $1.0596 \cdot 10^1$    |
| 4625  | $2.0259 \cdot 10^{-14}$ | $9.4206 \cdot 10^{-11}$ | $4.3806 \cdot 10^{-7}$  | $2.0370 \cdot 10^{-3}$ | $9.4719 \cdot 10^0$    |
| 4650  | $1.7753 \cdot 10^{-14}$ | $8.2997 \cdot 10^{-11}$ | $3.8801 \cdot 10^{-7}$  | $1.8140 \cdot 10^{-3}$ | $8.4802 \cdot 10^0$    |
| 4675  | $1.5563 \cdot 10^{-14}$ | $7.3144 \cdot 10^{-11}$ | $3.4378 \cdot 10^{-7}$  | $1.6158 \cdot 10^{-3}$ | $7.5941 \cdot 10^0$    |
| 4700  | $1.3648 \cdot 10^{-14}$ | $6.4486 \cdot 10^{-11}$ | $3.0470 \cdot 10^{-7}$  | $1.4397 \cdot 10^{-3}$ | $6.8026 \cdot 10^0$    |
| 4725  | $1.1976 \cdot 10^{-14}$ | $5.6887 \cdot 10^{-11}$ | $2.7021 \cdot 10^{-7}$  | $1.2835 \cdot 10^{-3}$ | $6.0967 \cdot 10^0$    |
| 4750  | $1.0491 \cdot 10^{-14}$ | $5.0095 \cdot 10^{-11}$ | $2.3920 \cdot 10^{-7}$  | $1.1422 \cdot 10^{-3}$ | $5.4540 \cdot 10^0$    |
| 4775  | $9.1894 \cdot 10^{-15}$ | $4.4109 \cdot 10^{-11}$ | $2.1172 \cdot 10^{-7}$  | $1.0163 \cdot 10^{-3}$ | $4.8781 \cdot 10^0$    |
| 4800  | $8.0537 \cdot 10^{-15}$ | $3.8859 \cdot 10^{-11}$ | $1.8750 \cdot 10^{-7}$  | $9.0466 \cdot 10^{-4}$ | $4.3650 \cdot 10^0$    |
| 4825  | $7.0614 \cdot 10^{-15}$ | $3.4248 \cdot 10^{-11}$ | $1.6610 \cdot 10^{-7}$  | $8.0560 \cdot 10^{-4}$ | $3.9072 \cdot 10^0$    |
| 4850  | $6.1951 \cdot 10^{-15}$ | $3.0201 \cdot 10^{-11}$ | $1.4723 \cdot 10^{-7}$  | $7.1775 \cdot 10^{-4}$ | $3.4990 \cdot 10^0$    |
| 4875  | $5.4361 \cdot 10^{-15}$ | $2.6637 \cdot 10^{-11}$ | $1.3052 \cdot 10^{-7}$  | $6.3955 \cdot 10^{-4}$ | $3.1338 \cdot 10^0$    |
| 4900  | $4.7720 \cdot 10^{-15}$ | $2.3502 \cdot 10^{-11}$ | $1.1575 \cdot 10^{-7}$  | $5.7006 \cdot 10^{-4}$ | $2.8076 \cdot 10^0$    |
| 4925  | $4.1878 \cdot 10^{-15}$ | $2.0729 \cdot 10^{-11}$ | $1.0261 \cdot 10^{-7}$  | $5.0792 \cdot 10^{-4}$ | $2.5142 \cdot 10^0$    |
| 4950  | $3.6731 \cdot 10^{-15}$ | $1.8274 \cdot 10^{-11}$ | $9.0911 \cdot 10^{-8}$  | $4.5228 \cdot 10^{-4}$ | $2.2501 \cdot 10^0$    |
| 4975  | $3.2229 \cdot 10^{-15}$ | $1.6114 \cdot 10^{-11}$ | $8.0571 \cdot 10^{-8}$  | $4.0286 \cdot 10^{-4}$ | $2.0143 \cdot 10^0$    |
| 5000  | $2.8715 \cdot 10^{-15}$ | $1.4645 \cdot 10^{-11}$ | $7.4687 \cdot 10^{-8}$  | $3.8090 \cdot 10^{-4}$ | $1.9426 \cdot 10^0$    |
| 5100  | $1.7087 \cdot 10^{-15}$ | $8.8850 \cdot 10^{-12}$ | $4.6202 \cdot 10^{-8}$  | $2.4025 \cdot 10^{-4}$ | $1.2493 \cdot 10^0$    |
| 5200  | $1.0185 \cdot 10^{-15}$ | $5.3980 \cdot 10^{-12}$ | $2.8610 \cdot 10^{-8}$  | $1.5163 \cdot 10^{-4}$ | $8.0364 \cdot 10^{-1}$ |
| 5300  | $6.0977 \cdot 10^{-16}$ | $3.2927 \cdot 10^{-12}$ | $1.7781 \cdot 10^{-8}$  | $9.6016 \cdot 10^{-5}$ | $5.1849 \cdot 10^{-1}$ |
| 5400  | $3.6472 \cdot 10^{-16}$ | $2.0059 \cdot 10^{-12}$ | $1.1033 \cdot 10^{-8}$  | $6.0679 \cdot 10^{-5}$ | $3.3374 \cdot 10^{-1}$ |
| 5500  | $2.1916 \cdot 10^{-16}$ | $1.2273 \cdot 10^{-12}$ | $6.8727 \cdot 10^{-9}$  | $3.8487 \cdot 10^{-5}$ | $2.1553 \cdot 10^{-1}$ |
| 5600  | $1.3217 \cdot 10^{-16}$ | $7.5337 \cdot 10^{-13}$ | $4.2942 \cdot 10^{-9}$  | $2.4477 \cdot 10^{-5}$ | $1.3952 \cdot 10^{-1}$ |
| 5700  | $8.0079 \cdot 10^{-17}$ | $4.6446 \cdot 10^{-13}$ | $2.6938 \cdot 10^{-9}$  | $1.5624 \cdot 10^{-5}$ | $9.0621 \cdot 10^{-2}$ |
| 5800  | $4.8518 \cdot 10^{-17}$ | $2.8626 \cdot 10^{-13}$ | $1.6889 \cdot 10^{-9}$  | $9.9646 \cdot 10^{-6}$ | $5.8791 \cdot 10^{-2}$ |
| 5900  | $2.9482 \cdot 10^{-17}$ | $1.7689 \cdot 10^{-13}$ | $1.0614 \cdot 10^{-9}$  | $6.3682 \cdot 10^{-6}$ | $3.8209 \cdot 10^{-2}$ |
| 6000  | $1.7952 \cdot 10^{-17}$ | $1.0951 \cdot 10^{-13}$ | $6.6798 \cdot 10^{-10}$ | $4.0747 \cdot 10^{-6}$ | $2.4855 \cdot 10^{-2}$ |
| 6100  | $1.0987 \cdot 10^{-17}$ | $6.8120 \cdot 10^{-14}$ | $4.2234 \cdot 10^{-10}$ | $2.6185 \cdot 10^{-6}$ | $1.6235 \cdot 10^{-2}$ |
| 6200  | $6.7178 \cdot 10^{-18}$ | $4.2322 \cdot 10^{-14}$ | $2.6663 \cdot 10^{-10}$ | $1.6798 \cdot 10^{-6}$ | $1.0583 \cdot 10^{-2}$ |
| 6300  | $4.1267 \cdot 10^{-18}$ | $2.6411 \cdot 10^{-14}$ | $1.6903 \cdot 10^{-10}$ | $1.0818 \cdot 10^{-6}$ | $6.9235 \cdot 10^{-3}$ |
| 6400  | $2.5481 \cdot 10^{-18}$ | $1.6563 \cdot 10^{-14}$ | $1.0766 \cdot 10^{-10}$ | $6.9977 \cdot 10^{-7}$ | $4.5485 \cdot 10^{-3}$ |
| 6500  | $1.5741 \cdot 10^{-18}$ | $1.0389 \cdot 10^{-14}$ | $6.8566 \cdot 10^{-11}$ | $4.5253 \cdot 10^{-7}$ | $2.9867 \cdot 10^{-3}$ |
| 6600  | $9.7287 \cdot 10^{-19}$ | $6.5182 \cdot 10^{-15}$ | $4.3672 \cdot 10^{-11}$ | $2.9260 \cdot 10^{-7}$ | $1.9604 \cdot 10^{-3}$ |
| 6700  | $6.0447 \cdot 10^{-19}$ | $4.1104 \cdot 10^{-15}$ | $2.7951 \cdot 10^{-11}$ | $1.9007 \cdot 10^{-7}$ | $1.2924 \cdot 10^{-3}$ |
| 6800  | $3.7651 \cdot 10^{-19}$ | $2.5979 \cdot 10^{-15}$ | $1.7926 \cdot 10^{-11}$ | $1.2369 \cdot 10^{-7}$ | $8.5344 \cdot 10^{-4}$ |

Continued on next page



Table 10 – continued from previous page

| $b_j$ | $B_{j,1}$               | $B_{j,2}$               | $B_{j,3}$               | $B_{j,4}$               | $B_{j,5}$               |
|-------|-------------------------|-------------------------|-------------------------|-------------------------|-------------------------|
| 6900  | $2.3554 \cdot 10^{-19}$ | $1.6488 \cdot 10^{-15}$ | $1.1542 \cdot 10^{-11}$ | $8.0791 \cdot 10^{-8}$  | $5.6554 \cdot 10^{-4}$  |
| 7000  | $1.4744 \cdot 10^{-19}$ | $1.0468 \cdot 10^{-15}$ | $7.4322 \cdot 10^{-12}$ | $5.2769 \cdot 10^{-8}$  | $3.7466 \cdot 10^{-4}$  |
| 7100  | $9.2826 \cdot 10^{-20}$ | $6.6834 \cdot 10^{-16}$ | $4.8121 \cdot 10^{-12}$ | $3.4647 \cdot 10^{-8}$  | $2.4946 \cdot 10^{-4}$  |
| 7200  | $5.8601 \cdot 10^{-20}$ | $4.2779 \cdot 10^{-16}$ | $3.1229 \cdot 10^{-12}$ | $2.2797 \cdot 10^{-8}$  | $1.6642 \cdot 10^{-4}$  |
| 7300  | $3.7014 \cdot 10^{-20}$ | $2.7390 \cdot 10^{-16}$ | $2.0269 \cdot 10^{-12}$ | $1.4999 \cdot 10^{-8}$  | $1.1099 \cdot 10^{-4}$  |
| 7400  | $2.3488 \cdot 10^{-20}$ | $1.7616 \cdot 10^{-16}$ | $1.3212 \cdot 10^{-12}$ | $9.9091 \cdot 10^{-9}$  | $7.4318 \cdot 10^{-5}$  |
| 7500  | $1.4907 \cdot 10^{-20}$ | $1.1330 \cdot 10^{-16}$ | $8.6105 \cdot 10^{-13}$ | $6.5440 \cdot 10^{-9}$  | $4.9734 \cdot 10^{-5}$  |
| 7600  | $9.4822 \cdot 10^{-21}$ | $7.3013 \cdot 10^{-17}$ | $5.6220 \cdot 10^{-13}$ | $4.3289 \cdot 10^{-9}$  | $3.3333 \cdot 10^{-5}$  |
| 7700  | $6.0569 \cdot 10^{-21}$ | $4.7244 \cdot 10^{-17}$ | $3.6850 \cdot 10^{-13}$ | $2.8743 \cdot 10^{-9}$  | $2.2420 \cdot 10^{-5}$  |
| 7800  | $3.8811 \cdot 10^{-21}$ | $3.0661 \cdot 10^{-17}$ | $2.4222 \cdot 10^{-13}$ | $1.9136 \cdot 10^{-9}$  | $1.5117 \cdot 10^{-5}$  |
| 7900  | $2.4928 \cdot 10^{-21}$ | $1.9942 \cdot 10^{-17}$ | $1.5954 \cdot 10^{-13}$ | $1.2763 \cdot 10^{-9}$  | $1.0211 \cdot 10^{-5}$  |
| 8000  | $1.6007 \cdot 10^{-21}$ | $1.2965 \cdot 10^{-17}$ | $1.0502 \cdot 10^{-13}$ | $8.5065 \cdot 10^{-10}$ | $6.8903 \cdot 10^{-6}$  |
| 8100  | $1.0326 \cdot 10^{-21}$ | $8.4674 \cdot 10^{-18}$ | $6.9433 \cdot 10^{-14}$ | $5.6935 \cdot 10^{-10}$ | $4.6687 \cdot 10^{-6}$  |
| 8200  | $6.6828 \cdot 10^{-22}$ | $5.5467 \cdot 10^{-18}$ | $4.6038 \cdot 10^{-14}$ | $3.8212 \cdot 10^{-10}$ | $3.1716 \cdot 10^{-6}$  |
| 8300  | $4.3257 \cdot 10^{-22}$ | $3.6336 \cdot 10^{-18}$ | $3.0522 \cdot 10^{-14}$ | $2.5639 \cdot 10^{-10}$ | $2.1536 \cdot 10^{-6}$  |
| 8400  | $2.8105 \cdot 10^{-22}$ | $2.3889 \cdot 10^{-18}$ | $2.0306 \cdot 10^{-14}$ | $1.7260 \cdot 10^{-10}$ | $1.4671 \cdot 10^{-6}$  |
| 8500  | $1.8315 \cdot 10^{-22}$ | $1.5751 \cdot 10^{-18}$ | $1.3546 \cdot 10^{-14}$ | $1.1650 \cdot 10^{-10}$ | $1.0019 \cdot 10^{-6}$  |
| 8600  | $1.1981 \cdot 10^{-22}$ | $1.0423 \cdot 10^{-18}$ | $9.0682 \cdot 10^{-15}$ | $7.8893 \cdot 10^{-11}$ | $6.8637 \cdot 10^{-7}$  |
| 8700  | $7.8220 \cdot 10^{-23}$ | $6.8834 \cdot 10^{-19}$ | $6.0574 \cdot 10^{-15}$ | $5.3305 \cdot 10^{-11}$ | $4.6908 \cdot 10^{-7}$  |
| 8800  | $5.1585 \cdot 10^{-23}$ | $4.5910 \cdot 10^{-19}$ | $4.0860 \cdot 10^{-15}$ | $3.6366 \cdot 10^{-11}$ | $3.2365 \cdot 10^{-7}$  |
| 8900  | $3.3882 \cdot 10^{-23}$ | $3.0494 \cdot 10^{-19}$ | $2.7445 \cdot 10^{-15}$ | $2.4700 \cdot 10^{-11}$ | $2.2230 \cdot 10^{-7}$  |
| 9000  | $2.2252 \cdot 10^{-23}$ | $2.0250 \cdot 10^{-19}$ | $1.8427 \cdot 10^{-15}$ | $1.6769 \cdot 10^{-11}$ | $1.5260 \cdot 10^{-7}$  |
| 9100  | $1.4641 \cdot 10^{-23}$ | $1.3470 \cdot 10^{-19}$ | $1.2392 \cdot 10^{-15}$ | $1.1401 \cdot 10^{-11}$ | $1.0489 \cdot 10^{-7}$  |
| 9200  | $9.6777 \cdot 10^{-24}$ | $9.0003 \cdot 10^{-20}$ | $8.3703 \cdot 10^{-16}$ | $7.7844 \cdot 10^{-12}$ | $7.2395 \cdot 10^{-8}$  |
| 9300  | $6.4195 \cdot 10^{-24}$ | $6.0343 \cdot 10^{-20}$ | $5.6723 \cdot 10^{-16}$ | $5.3319 \cdot 10^{-12}$ | $5.0120 \cdot 10^{-8}$  |
| 9400  | $4.2972 \cdot 10^{-24}$ | $4.0823 \cdot 10^{-20}$ | $3.8782 \cdot 10^{-16}$ | $3.6843 \cdot 10^{-12}$ | $3.5001 \cdot 10^{-8}$  |
| 9500  | $2.8512 \cdot 10^{-24}$ | $2.7372 \cdot 10^{-20}$ | $2.6277 \cdot 10^{-16}$ | $2.5226 \cdot 10^{-12}$ | $2.4217 \cdot 10^{-8}$  |
| 9600  | $1.9059 \cdot 10^{-24}$ | $1.8487 \cdot 10^{-20}$ | $1.7932 \cdot 10^{-16}$ | $1.7395 \cdot 10^{-12}$ | $1.6873 \cdot 10^{-8}$  |
| 9700  | $1.2689 \cdot 10^{-24}$ | $1.2435 \cdot 10^{-20}$ | $1.2187 \cdot 10^{-16}$ | $1.1943 \cdot 10^{-12}$ | $1.1704 \cdot 10^{-8}$  |
| 9800  | $8.4841 \cdot 10^{-25}$ | $8.3992 \cdot 10^{-21}$ | $8.3152 \cdot 10^{-17}$ | $8.2321 \cdot 10^{-13}$ | $8.1497 \cdot 10^{-9}$  |
| 9900  | $5.7395 \cdot 10^{-25}$ | $5.7395 \cdot 10^{-21}$ | $5.7395 \cdot 10^{-17}$ | $5.7395 \cdot 10^{-13}$ | $5.7395 \cdot 10^{-9}$  |
| 10000 | $3.8228 \cdot 10^{-25}$ | $3.8610 \cdot 10^{-21}$ | $3.8996 \cdot 10^{-17}$ | $3.9386 \cdot 10^{-13}$ | $3.9780 \cdot 10^{-9}$  |
| 10100 | $2.5745 \cdot 10^{-25}$ | $2.6260 \cdot 10^{-21}$ | $2.6785 \cdot 10^{-17}$ | $2.7321 \cdot 10^{-13}$ | $2.7867 \cdot 10^{-9}$  |
| 10200 | $1.7389 \cdot 10^{-25}$ | $1.7911 \cdot 10^{-21}$ | $1.8448 \cdot 10^{-17}$ | $1.9001 \cdot 10^{-13}$ | $1.9571 \cdot 10^{-9}$  |
| 10300 | $1.1734 \cdot 10^{-25}$ | $1.2203 \cdot 10^{-21}$ | $1.2691 \cdot 10^{-17}$ | $1.3199 \cdot 10^{-13}$ | $1.3727 \cdot 10^{-9}$  |
| 10400 | $7.9556 \cdot 10^{-26}$ | $8.3534 \cdot 10^{-22}$ | $8.7710 \cdot 10^{-18}$ | $9.2096 \cdot 10^{-14}$ | $9.6701 \cdot 10^{-10}$ |
| 10500 | $5.4076 \cdot 10^{-26}$ | $5.7321 \cdot 10^{-22}$ | $6.0760 \cdot 10^{-18}$ | $6.4406 \cdot 10^{-14}$ | $6.8270 \cdot 10^{-10}$ |
| 10600 | $3.6845 \cdot 10^{-26}$ | $3.9424 \cdot 10^{-22}$ | $4.2184 \cdot 10^{-18}$ | $4.5136 \cdot 10^{-14}$ | $4.8296 \cdot 10^{-10}$ |
| 10700 | $2.5150 \cdot 10^{-26}$ | $2.7162 \cdot 10^{-22}$ | $2.9335 \cdot 10^{-18}$ | $3.1682 \cdot 10^{-14}$ | $3.4216 \cdot 10^{-10}$ |
| 10800 | $1.7201 \cdot 10^{-26}$ | $1.8749 \cdot 10^{-22}$ | $2.0436 \cdot 10^{-18}$ | $2.2276 \cdot 10^{-14}$ | $2.4280 \cdot 10^{-10}$ |
| 10900 | $1.1639 \cdot 10^{-26}$ | $1.2803 \cdot 10^{-22}$ | $1.4083 \cdot 10^{-18}$ | $1.5492 \cdot 10^{-14}$ | $1.7041 \cdot 10^{-10}$ |
| 11000 | $7.9283 \cdot 10^{-27}$ | $8.8005 \cdot 10^{-23}$ | $9.7685 \cdot 10^{-19}$ | $1.0843 \cdot 10^{-14}$ | $1.2036 \cdot 10^{-10}$ |
| 11100 | $5.4156 \cdot 10^{-27}$ | $6.0654 \cdot 10^{-23}$ | $6.7933 \cdot 10^{-19}$ | $7.6085 \cdot 10^{-15}$ | $8.5215 \cdot 10^{-11}$ |
| 11200 | $3.7120 \cdot 10^{-27}$ | $4.1945 \cdot 10^{-23}$ | $4.7398 \cdot 10^{-19}$ | $5.3560 \cdot 10^{-15}$ | $6.0522 \cdot 10^{-11}$ |
| 11300 | $2.5509 \cdot 10^{-27}$ | $2.9080 \cdot 10^{-23}$ | $3.3151 \cdot 10^{-19}$ | $3.7792 \cdot 10^{-15}$ | $4.3083 \cdot 10^{-11}$ |
| 11400 | $1.7569 \cdot 10^{-27}$ | $2.0205 \cdot 10^{-23}$ | $2.3235 \cdot 10^{-19}$ | $2.6721 \cdot 10^{-15}$ | $3.0729 \cdot 10^{-11}$ |
| 11500 | $1.2102 \cdot 10^{-27}$ | $1.4039 \cdot 10^{-23}$ | $1.6285 \cdot 10^{-19}$ | $1.8890 \cdot 10^{-15}$ | $2.1913 \cdot 10^{-11}$ |
| 11600 | $8.3444 \cdot 10^{-28}$ | $9.7630 \cdot 10^{-24}$ | $1.1423 \cdot 10^{-19}$ | $1.3365 \cdot 10^{-15}$ | $1.5637 \cdot 10^{-11}$ |
| 11700 | $5.7692 \cdot 10^{-28}$ | $6.8076 \cdot 10^{-24}$ | $8.0330 \cdot 10^{-20}$ | $9.4789 \cdot 10^{-16}$ | $1.1185 \cdot 10^{-11}$ |
| 11800 | $3.9987 \cdot 10^{-28}$ | $4.7584 \cdot 10^{-24}$ | $5.6625 \cdot 10^{-20}$ | $6.7384 \cdot 10^{-16}$ | $8.0187 \cdot 10^{-12}$ |
| 11900 | $2.7776 \cdot 10^{-28}$ | $3.3331 \cdot 10^{-24}$ | $3.9997 \cdot 10^{-20}$ | $4.7996 \cdot 10^{-16}$ | $5.7595 \cdot 10^{-12}$ |
| 12000 | $1.9330 \cdot 10^{-28}$ | $2.3390 \cdot 10^{-24}$ | $2.8302 \cdot 10^{-20}$ | $3.4245 \cdot 10^{-16}$ | $4.1436 \cdot 10^{-12}$ |
| 12100 | $1.3477 \cdot 10^{-28}$ | $1.6442 \cdot 10^{-24}$ | $2.0060 \cdot 10^{-20}$ | $2.4473 \cdot 10^{-16}$ | $2.9857 \cdot 10^{-12}$ |
| 12200 | $9.3146 \cdot 10^{-29}$ | $1.1457 \cdot 10^{-24}$ | $1.4092 \cdot 10^{-20}$ | $1.7333 \cdot 10^{-16}$ | $2.1320 \cdot 10^{-12}$ |
| 12300 | $6.5069 \cdot 10^{-29}$ | $8.0685 \cdot 10^{-25}$ | $1.0005 \cdot 10^{-20}$ | $1.2406 \cdot 10^{-16}$ | $1.5384 \cdot 10^{-12}$ |

Continued on next page

Table 10 – continued from previous page

| $b_j$      | $B_{j,1}$               | $B_{j,2}$               | $B_{j,3}$               | $B_{j,4}$               | $B_{j,5}$               |
|------------|-------------------------|-------------------------|-------------------------|-------------------------|-------------------------|
| 12400      | $4.5539 \cdot 10^{-29}$ | $5.6924 \cdot 10^{-25}$ | $7.1155 \cdot 10^{-21}$ | $8.8944 \cdot 10^{-17}$ | $1.1118 \cdot 10^{-12}$ |
| 12500      | $3.1924 \cdot 10^{-29}$ | $4.0224 \cdot 10^{-25}$ | $5.0682 \cdot 10^{-21}$ | $6.3859 \cdot 10^{-17}$ | $8.0462 \cdot 10^{-13}$ |
| 12600      | $2.2307 \cdot 10^{-29}$ | $2.8330 \cdot 10^{-25}$ | $3.5979 \cdot 10^{-21}$ | $4.5693 \cdot 10^{-17}$ | $5.8030 \cdot 10^{-13}$ |
| 12700      | $1.5599 \cdot 10^{-29}$ | $1.9967 \cdot 10^{-25}$ | $2.5558 \cdot 10^{-21}$ | $3.2714 \cdot 10^{-17}$ | $4.1873 \cdot 10^{-13}$ |
| 12800      | $1.0940 \cdot 10^{-29}$ | $1.4112 \cdot 10^{-25}$ | $1.8205 \cdot 10^{-21}$ | $2.3484 \cdot 10^{-17}$ | $3.0294 \cdot 10^{-13}$ |
| 12900      | $7.6899 \cdot 10^{-30}$ | $9.9969 \cdot 10^{-26}$ | $1.2996 \cdot 10^{-21}$ | $1.6895 \cdot 10^{-17}$ | $2.1963 \cdot 10^{-13}$ |
| 13000      | $5.5830 \cdot 10^{-30}$ | $7.5370 \cdot 10^{-26}$ | $1.0175 \cdot 10^{-21}$ | $1.3736 \cdot 10^{-17}$ | $1.8544 \cdot 10^{-13}$ |
| 13500      | $9.9578 \cdot 10^{-31}$ | $1.3743 \cdot 10^{-26}$ | $1.8966 \cdot 10^{-22}$ | $2.6174 \cdot 10^{-18}$ | $3.6122 \cdot 10^{-14}$ |
| 13800.7464 | $3.5592 \cdot 10^{-31}$ | $4.9829 \cdot 10^{-27}$ | $6.9761 \cdot 10^{-23}$ | $9.7665 \cdot 10^{-19}$ | $1.3673 \cdot 10^{-14}$ |
| 14000      | $1.8398 \cdot 10^{-31}$ | $2.7597 \cdot 10^{-27}$ | $4.1396 \cdot 10^{-23}$ | $6.2094 \cdot 10^{-19}$ | $9.3141 \cdot 10^{-15}$ |
| 15000      | $6.5711 \cdot 10^{-33}$ | $1.0514 \cdot 10^{-28}$ | $1.6822 \cdot 10^{-24}$ | $2.6915 \cdot 10^{-20}$ | $4.3065 \cdot 10^{-16}$ |
| 16000      | $2.5738 \cdot 10^{-34}$ | $4.3755 \cdot 10^{-30}$ | $7.4384 \cdot 10^{-26}$ | $1.2645 \cdot 10^{-21}$ | $2.1497 \cdot 10^{-17}$ |
| 17000      | $1.1167 \cdot 10^{-35}$ | $2.0101 \cdot 10^{-31}$ | $3.6182 \cdot 10^{-27}$ | $6.5127 \cdot 10^{-23}$ | $1.1723 \cdot 10^{-18}$ |
| 18000      | $5.3738 \cdot 10^{-37}$ | $1.0210 \cdot 10^{-32}$ | $1.9400 \cdot 10^{-28}$ | $3.6859 \cdot 10^{-24}$ | $7.0032 \cdot 10^{-20}$ |
| 19000      | $2.7357 \cdot 10^{-38}$ | $5.4714 \cdot 10^{-34}$ | $1.0943 \cdot 10^{-29}$ | $2.1886 \cdot 10^{-25}$ | $4.3771 \cdot 10^{-21}$ |
| 20000      | $1.5040 \cdot 10^{-39}$ | $3.1585 \cdot 10^{-35}$ | $6.6328 \cdot 10^{-31}$ | $1.3929 \cdot 10^{-26}$ | $2.9251 \cdot 10^{-22}$ |
| 21000      | $9.0605 \cdot 10^{-41}$ | $1.9933 \cdot 10^{-36}$ | $4.3853 \cdot 10^{-32}$ | $9.6476 \cdot 10^{-28}$ | $2.1225 \cdot 10^{-23}$ |
| 22000      | $5.6101 \cdot 10^{-42}$ | $1.2903 \cdot 10^{-37}$ | $2.9677 \cdot 10^{-33}$ | $6.8258 \cdot 10^{-29}$ | $1.5699 \cdot 10^{-24}$ |
| 23000      | $3.7554 \cdot 10^{-43}$ | $9.0129 \cdot 10^{-39}$ | $2.1631 \cdot 10^{-34}$ | $5.1914 \cdot 10^{-30}$ | $1.2460 \cdot 10^{-25}$ |
| 24000      | $2.6755 \cdot 10^{-44}$ | $6.6888 \cdot 10^{-40}$ | $1.6722 \cdot 10^{-35}$ | $4.1805 \cdot 10^{-31}$ | $1.0451 \cdot 10^{-26}$ |

TABLE 11. Supplement for Table 10. Values for  $\mathcal{B}_{j,k}$  in  $|\theta(x) - x| < \frac{\mathcal{B}_{j,k}x}{(\log x)^k}$  calculated using the method described in Corollary 8.1, Section 3.2 of [1]. Each  $\mathcal{B}_{j,k}$  is valid for  $x \in [e^{b_j}, e^{25000}]$ .

| $b_j$ | $\mathcal{B}_{j,1}$    | $\mathcal{B}_{j,2}$    | $\mathcal{B}_{j,3}$    | $\mathcal{B}_{j,4}$ | $\mathcal{B}_{j,5}$ |
|-------|------------------------|------------------------|------------------------|---------------------|---------------------|
| 20    | $1.6844 \cdot 10^{-3}$ | $3.3688 \cdot 10^{-2}$ | $6.7375 \cdot 10^{-1}$ | $5.7184 \cdot 10^1$ | $1.3441 \cdot 10^5$ |
| 21    | $1.0684 \cdot 10^{-3}$ | $2.2435 \cdot 10^{-2}$ | $4.7114 \cdot 10^{-1}$ | $5.7184 \cdot 10^1$ | $1.3441 \cdot 10^5$ |
| 22    | $6.7654 \cdot 10^{-4}$ | $1.4884 \cdot 10^{-2}$ | $3.2746 \cdot 10^{-1}$ | $5.7184 \cdot 10^1$ | $1.3441 \cdot 10^5$ |
| 23    | $4.2780 \cdot 10^{-4}$ | $9.8392 \cdot 10^{-3}$ | $2.2631 \cdot 10^{-1}$ | $5.7184 \cdot 10^1$ | $1.3441 \cdot 10^5$ |
| 24    | $2.7011 \cdot 10^{-4}$ | $6.4827 \cdot 10^{-3}$ | $1.5559 \cdot 10^{-1}$ | $5.7184 \cdot 10^1$ | $1.3441 \cdot 10^5$ |
| 25    | $1.7500 \cdot 10^{-4}$ | $4.3750 \cdot 10^{-3}$ | $1.0938 \cdot 10^{-1}$ | $5.7184 \cdot 10^1$ | $1.3441 \cdot 10^5$ |
| 26    | $1.1022 \cdot 10^{-4}$ | $2.8655 \cdot 10^{-3}$ | $7.4503 \cdot 10^{-2}$ | $5.7184 \cdot 10^1$ | $1.3441 \cdot 10^5$ |
| 27    | $6.9322 \cdot 10^{-5}$ | $1.8717 \cdot 10^{-3}$ | $5.0536 \cdot 10^{-2}$ | $5.7184 \cdot 10^1$ | $1.3441 \cdot 10^5$ |
| 28    | $4.3555 \cdot 10^{-5}$ | $1.2196 \cdot 10^{-3}$ | $3.4148 \cdot 10^{-2}$ | $5.7184 \cdot 10^1$ | $1.3441 \cdot 10^5$ |
| 29    | $2.7336 \cdot 10^{-5}$ | $7.9272 \cdot 10^{-4}$ | $2.4334 \cdot 10^{-2}$ | $5.7184 \cdot 10^1$ | $1.3441 \cdot 10^5$ |
| 30    | $1.7139 \cdot 10^{-5}$ | $5.1415 \cdot 10^{-4}$ | $2.4334 \cdot 10^{-2}$ | $5.7184 \cdot 10^1$ | $1.3441 \cdot 10^5$ |
| 31    | $1.0735 \cdot 10^{-5}$ | $3.3277 \cdot 10^{-4}$ | $2.4334 \cdot 10^{-2}$ | $5.7184 \cdot 10^1$ | $1.3441 \cdot 10^5$ |
| 32    | $7.0053 \cdot 10^{-6}$ | $2.2417 \cdot 10^{-4}$ | $2.4334 \cdot 10^{-2}$ | $5.7184 \cdot 10^1$ | $1.3441 \cdot 10^5$ |
| 33    | $4.3798 \cdot 10^{-6}$ | $1.4454 \cdot 10^{-4}$ | $2.4334 \cdot 10^{-2}$ | $5.7184 \cdot 10^1$ | $1.3441 \cdot 10^5$ |
| 34    | $2.7360 \cdot 10^{-6}$ | $9.3023 \cdot 10^{-5}$ | $2.4334 \cdot 10^{-2}$ | $5.7184 \cdot 10^1$ | $1.3441 \cdot 10^5$ |
| 35    | $1.7078 \cdot 10^{-6}$ | $5.9771 \cdot 10^{-5}$ | $2.4334 \cdot 10^{-2}$ | $5.7184 \cdot 10^1$ | $1.3441 \cdot 10^5$ |
| 36    | $1.0652 \cdot 10^{-6}$ | $3.8345 \cdot 10^{-5}$ | $2.4334 \cdot 10^{-2}$ | $5.7184 \cdot 10^1$ | $1.3441 \cdot 10^5$ |
| 37    | $8.6315 \cdot 10^{-7}$ | $3.7979 \cdot 10^{-5}$ | $2.4334 \cdot 10^{-2}$ | $5.7184 \cdot 10^1$ | $1.3441 \cdot 10^5$ |
| 38    | $8.6315 \cdot 10^{-7}$ | $3.7979 \cdot 10^{-5}$ | $2.4334 \cdot 10^{-2}$ | $5.7184 \cdot 10^1$ | $1.3441 \cdot 10^5$ |
| 39    | $8.6315 \cdot 10^{-7}$ | $3.7979 \cdot 10^{-5}$ | $2.4334 \cdot 10^{-2}$ | $5.7184 \cdot 10^1$ | $1.3441 \cdot 10^5$ |
| 40    | $8.6315 \cdot 10^{-7}$ | $3.7979 \cdot 10^{-5}$ | $2.4334 \cdot 10^{-2}$ | $5.7184 \cdot 10^1$ | $1.3441 \cdot 10^5$ |
| 41    | $8.6315 \cdot 10^{-7}$ | $3.7979 \cdot 10^{-5}$ | $2.4334 \cdot 10^{-2}$ | $5.7184 \cdot 10^1$ | $1.3441 \cdot 10^5$ |
| 42    | $8.6315 \cdot 10^{-7}$ | $3.7979 \cdot 10^{-5}$ | $2.4334 \cdot 10^{-2}$ | $5.7184 \cdot 10^1$ | $1.3441 \cdot 10^5$ |
| 43    | $8.6315 \cdot 10^{-7}$ | $3.7979 \cdot 10^{-5}$ | $2.4334 \cdot 10^{-2}$ | $5.7184 \cdot 10^1$ | $1.3441 \cdot 10^5$ |
| 43    | $8.6315 \cdot 10^{-7}$ | $3.7979 \cdot 10^{-5}$ | $2.4334 \cdot 10^{-2}$ | $5.7184 \cdot 10^1$ | $1.3441 \cdot 10^5$ |
| 44    | $7.8163 \cdot 10^{-7}$ | $3.5174 \cdot 10^{-5}$ | $2.4334 \cdot 10^{-2}$ | $5.7184 \cdot 10^1$ | $1.3441 \cdot 10^5$ |
| 45    | $5.0646 \cdot 10^{-7}$ | $2.3298 \cdot 10^{-5}$ | $2.4334 \cdot 10^{-2}$ | $5.7184 \cdot 10^1$ | $1.3441 \cdot 10^5$ |
| 46    | $3.2935 \cdot 10^{-7}$ | $1.5480 \cdot 10^{-5}$ | $2.4334 \cdot 10^{-2}$ | $5.7184 \cdot 10^1$ | $1.3441 \cdot 10^5$ |
| 47    | $2.1308 \cdot 10^{-7}$ | $1.0376 \cdot 10^{-5}$ | $2.4334 \cdot 10^{-2}$ | $5.7184 \cdot 10^1$ | $1.3441 \cdot 10^5$ |
| 48    | $1.3791 \cdot 10^{-7}$ | $1.0376 \cdot 10^{-5}$ | $2.4334 \cdot 10^{-2}$ | $5.7184 \cdot 10^1$ | $1.3441 \cdot 10^5$ |
| 49    | $8.9140 \cdot 10^{-8}$ | $1.0376 \cdot 10^{-5}$ | $2.4334 \cdot 10^{-2}$ | $5.7184 \cdot 10^1$ | $1.3441 \cdot 10^5$ |
| 50    | $5.7545 \cdot 10^{-8}$ | $1.0376 \cdot 10^{-5}$ | $2.4334 \cdot 10^{-2}$ | $5.7184 \cdot 10^1$ | $1.3441 \cdot 10^5$ |
| 51    | $3.7147 \cdot 10^{-8}$ | $1.0376 \cdot 10^{-5}$ | $2.4334 \cdot 10^{-2}$ | $5.7184 \cdot 10^1$ | $1.3441 \cdot 10^5$ |
| 52    | $2.3898 \cdot 10^{-8}$ | $1.0376 \cdot 10^{-5}$ | $2.4334 \cdot 10^{-2}$ | $5.7184 \cdot 10^1$ | $1.3441 \cdot 10^5$ |
| 53    | $1.5373 \cdot 10^{-8}$ | $1.0376 \cdot 10^{-5}$ | $2.4334 \cdot 10^{-2}$ | $5.7184 \cdot 10^1$ | $1.3441 \cdot 10^5$ |
| 54    | $9.8778 \cdot 10^{-9}$ | $1.0376 \cdot 10^{-5}$ | $2.4334 \cdot 10^{-2}$ | $5.7184 \cdot 10^1$ | $1.3441 \cdot 10^5$ |
| 55    | $6.3417 \cdot 10^{-9}$ | $1.0376 \cdot 10^{-5}$ | $2.4334 \cdot 10^{-2}$ | $5.7184 \cdot 10^1$ | $1.3441 \cdot 10^5$ |
| 56    | $4.4627 \cdot 10^{-9}$ | $1.0376 \cdot 10^{-5}$ | $2.4334 \cdot 10^{-2}$ | $5.7184 \cdot 10^1$ | $1.3441 \cdot 10^5$ |
| 57    | $4.4627 \cdot 10^{-9}$ | $1.0376 \cdot 10^{-5}$ | $2.4334 \cdot 10^{-2}$ | $5.7184 \cdot 10^1$ | $1.3441 \cdot 10^5$ |
| 58    | $4.4627 \cdot 10^{-9}$ | $1.0376 \cdot 10^{-5}$ | $2.4334 \cdot 10^{-2}$ | $5.7184 \cdot 10^1$ | $1.3441 \cdot 10^5$ |
| 59    | $4.4627 \cdot 10^{-9}$ | $1.0376 \cdot 10^{-5}$ | $2.4334 \cdot 10^{-2}$ | $5.7184 \cdot 10^1$ | $1.3441 \cdot 10^5$ |
| 60    | $4.4627 \cdot 10^{-9}$ | $1.0376 \cdot 10^{-5}$ | $2.4334 \cdot 10^{-2}$ | $5.7184 \cdot 10^1$ | $1.3441 \cdot 10^5$ |
| 65    | $4.4627 \cdot 10^{-9}$ | $1.0376 \cdot 10^{-5}$ | $2.4334 \cdot 10^{-2}$ | $5.7184 \cdot 10^1$ | $1.3441 \cdot 10^5$ |
| 70    | $4.4627 \cdot 10^{-9}$ | $1.0376 \cdot 10^{-5}$ | $2.4334 \cdot 10^{-2}$ | $5.7184 \cdot 10^1$ | $1.3441 \cdot 10^5$ |
| 75    | $4.4627 \cdot 10^{-9}$ | $1.0376 \cdot 10^{-5}$ | $2.4334 \cdot 10^{-2}$ | $5.7184 \cdot 10^1$ | $1.3441 \cdot 10^5$ |
| 80    | $4.4627 \cdot 10^{-9}$ | $1.0376 \cdot 10^{-5}$ | $2.4334 \cdot 10^{-2}$ | $5.7184 \cdot 10^1$ | $1.3441 \cdot 10^5$ |
| 85    | $4.4627 \cdot 10^{-9}$ | $1.0376 \cdot 10^{-5}$ | $2.4334 \cdot 10^{-2}$ | $5.7184 \cdot 10^1$ | $1.3441 \cdot 10^5$ |
| 90    | $4.4627 \cdot 10^{-9}$ | $1.0376 \cdot 10^{-5}$ | $2.4334 \cdot 10^{-2}$ | $5.7184 \cdot 10^1$ | $1.3441 \cdot 10^5$ |
| 95    | $4.4627 \cdot 10^{-9}$ | $1.0376 \cdot 10^{-5}$ | $2.4334 \cdot 10^{-2}$ | $5.7184 \cdot 10^1$ | $1.3441 \cdot 10^5$ |
| 100   | $4.4627 \cdot 10^{-9}$ | $1.0376 \cdot 10^{-5}$ | $2.4334 \cdot 10^{-2}$ | $5.7184 \cdot 10^1$ | $1.3441 \cdot 10^5$ |

Continued on next page

Table 11 – continued from previous page

| $b_j$ | $\mathcal{B}_{j,1}$     | $\mathcal{B}_{j,2}$    | $\mathcal{B}_{j,3}$    | $\mathcal{B}_{j,4}$ | $\mathcal{B}_{j,5}$ |
|-------|-------------------------|------------------------|------------------------|---------------------|---------------------|
| 200   | $4.4627 \cdot 10^{-9}$  | $1.0376 \cdot 10^{-5}$ | $2.4334 \cdot 10^{-2}$ | $5.7184 \cdot 10^1$ | $1.3441 \cdot 10^5$ |
| 300   | $4.4627 \cdot 10^{-9}$  | $1.0376 \cdot 10^{-5}$ | $2.4334 \cdot 10^{-2}$ | $5.7184 \cdot 10^1$ | $1.3441 \cdot 10^5$ |
| 400   | $4.4627 \cdot 10^{-9}$  | $1.0376 \cdot 10^{-5}$ | $2.4334 \cdot 10^{-2}$ | $5.7184 \cdot 10^1$ | $1.3441 \cdot 10^5$ |
| 500   | $4.4627 \cdot 10^{-9}$  | $1.0376 \cdot 10^{-5}$ | $2.4334 \cdot 10^{-2}$ | $5.7184 \cdot 10^1$ | $1.3441 \cdot 10^5$ |
| 600   | $4.4627 \cdot 10^{-9}$  | $1.0376 \cdot 10^{-5}$ | $2.4334 \cdot 10^{-2}$ | $5.7184 \cdot 10^1$ | $1.3441 \cdot 10^5$ |
| 700   | $4.4627 \cdot 10^{-9}$  | $1.0376 \cdot 10^{-5}$ | $2.4334 \cdot 10^{-2}$ | $5.7184 \cdot 10^1$ | $1.3441 \cdot 10^5$ |
| 800   | $4.4627 \cdot 10^{-9}$  | $1.0376 \cdot 10^{-5}$ | $2.4334 \cdot 10^{-2}$ | $5.7184 \cdot 10^1$ | $1.3441 \cdot 10^5$ |
| 900   | $4.4627 \cdot 10^{-9}$  | $1.0376 \cdot 10^{-5}$ | $2.4334 \cdot 10^{-2}$ | $5.7184 \cdot 10^1$ | $1.3441 \cdot 10^5$ |
| 1000  | $4.4627 \cdot 10^{-9}$  | $1.0376 \cdot 10^{-5}$ | $2.4334 \cdot 10^{-2}$ | $5.7184 \cdot 10^1$ | $1.3441 \cdot 10^5$ |
| 1500  | $4.4627 \cdot 10^{-9}$  | $1.0376 \cdot 10^{-5}$ | $2.4334 \cdot 10^{-2}$ | $5.7184 \cdot 10^1$ | $1.3441 \cdot 10^5$ |
| 1600  | $4.4627 \cdot 10^{-9}$  | $1.0376 \cdot 10^{-5}$ | $2.4334 \cdot 10^{-2}$ | $5.7184 \cdot 10^1$ | $1.3441 \cdot 10^5$ |
| 1700  | $4.4627 \cdot 10^{-9}$  | $1.0376 \cdot 10^{-5}$ | $2.4334 \cdot 10^{-2}$ | $5.7184 \cdot 10^1$ | $1.3441 \cdot 10^5$ |
| 1725  | $4.4627 \cdot 10^{-9}$  | $1.0376 \cdot 10^{-5}$ | $2.4334 \cdot 10^{-2}$ | $5.7184 \cdot 10^1$ | $1.3441 \cdot 10^5$ |
| 1750  | $4.4627 \cdot 10^{-9}$  | $1.0376 \cdot 10^{-5}$ | $2.4334 \cdot 10^{-2}$ | $5.7184 \cdot 10^1$ | $1.3441 \cdot 10^5$ |
| 1775  | $4.4627 \cdot 10^{-9}$  | $1.0376 \cdot 10^{-5}$ | $2.4334 \cdot 10^{-2}$ | $5.7184 \cdot 10^1$ | $1.3441 \cdot 10^5$ |
| 1800  | $4.4627 \cdot 10^{-9}$  | $1.0376 \cdot 10^{-5}$ | $2.4334 \cdot 10^{-2}$ | $5.7184 \cdot 10^1$ | $1.3441 \cdot 10^5$ |
| 1825  | $4.4627 \cdot 10^{-9}$  | $1.0376 \cdot 10^{-5}$ | $2.4334 \cdot 10^{-2}$ | $5.7184 \cdot 10^1$ | $1.3441 \cdot 10^5$ |
| 1850  | $4.4627 \cdot 10^{-9}$  | $1.0376 \cdot 10^{-5}$ | $2.4334 \cdot 10^{-2}$ | $5.7184 \cdot 10^1$ | $1.3441 \cdot 10^5$ |
| 1875  | $4.4627 \cdot 10^{-9}$  | $1.0376 \cdot 10^{-5}$ | $2.4334 \cdot 10^{-2}$ | $5.7184 \cdot 10^1$ | $1.3441 \cdot 10^5$ |
| 1900  | $4.4627 \cdot 10^{-9}$  | $1.0376 \cdot 10^{-5}$ | $2.4334 \cdot 10^{-2}$ | $5.7184 \cdot 10^1$ | $1.3441 \cdot 10^5$ |
| 1925  | $4.4627 \cdot 10^{-9}$  | $1.0376 \cdot 10^{-5}$ | $2.4334 \cdot 10^{-2}$ | $5.7184 \cdot 10^1$ | $1.3441 \cdot 10^5$ |
| 1950  | $4.4627 \cdot 10^{-9}$  | $1.0376 \cdot 10^{-5}$ | $2.4334 \cdot 10^{-2}$ | $5.7184 \cdot 10^1$ | $1.3441 \cdot 10^5$ |
| 1975  | $4.4627 \cdot 10^{-9}$  | $1.0376 \cdot 10^{-5}$ | $2.4334 \cdot 10^{-2}$ | $5.7184 \cdot 10^1$ | $1.3441 \cdot 10^5$ |
| 2000  | $4.4627 \cdot 10^{-9}$  | $1.0376 \cdot 10^{-5}$ | $2.4334 \cdot 10^{-2}$ | $5.7184 \cdot 10^1$ | $1.3441 \cdot 10^5$ |
| 2025  | $4.4627 \cdot 10^{-9}$  | $1.0376 \cdot 10^{-5}$ | $2.4334 \cdot 10^{-2}$ | $5.7184 \cdot 10^1$ | $1.3441 \cdot 10^5$ |
| 2050  | $4.4627 \cdot 10^{-9}$  | $1.0376 \cdot 10^{-5}$ | $2.4334 \cdot 10^{-2}$ | $5.7184 \cdot 10^1$ | $1.3441 \cdot 10^5$ |
| 2075  | $4.4627 \cdot 10^{-9}$  | $1.0376 \cdot 10^{-5}$ | $2.4334 \cdot 10^{-2}$ | $5.7184 \cdot 10^1$ | $1.3441 \cdot 10^5$ |
| 2100  | $4.4627 \cdot 10^{-9}$  | $1.0376 \cdot 10^{-5}$ | $2.4334 \cdot 10^{-2}$ | $5.7184 \cdot 10^1$ | $1.3441 \cdot 10^5$ |
| 2125  | $4.4627 \cdot 10^{-9}$  | $1.0376 \cdot 10^{-5}$ | $2.4334 \cdot 10^{-2}$ | $5.7184 \cdot 10^1$ | $1.3441 \cdot 10^5$ |
| 2150  | $4.4627 \cdot 10^{-9}$  | $1.0376 \cdot 10^{-5}$ | $2.4334 \cdot 10^{-2}$ | $5.7184 \cdot 10^1$ | $1.3441 \cdot 10^5$ |
| 2175  | $4.4627 \cdot 10^{-9}$  | $1.0376 \cdot 10^{-5}$ | $2.4334 \cdot 10^{-2}$ | $5.7184 \cdot 10^1$ | $1.3441 \cdot 10^5$ |
| 2200  | $4.4627 \cdot 10^{-9}$  | $1.0376 \cdot 10^{-5}$ | $2.4334 \cdot 10^{-2}$ | $5.7184 \cdot 10^1$ | $1.3441 \cdot 10^5$ |
| 2225  | $4.4627 \cdot 10^{-9}$  | $1.0376 \cdot 10^{-5}$ | $2.4334 \cdot 10^{-2}$ | $5.7184 \cdot 10^1$ | $1.3441 \cdot 10^5$ |
| 2250  | $4.4627 \cdot 10^{-9}$  | $1.0376 \cdot 10^{-5}$ | $2.4334 \cdot 10^{-2}$ | $5.7184 \cdot 10^1$ | $1.3441 \cdot 10^5$ |
| 2275  | $4.4627 \cdot 10^{-9}$  | $1.0376 \cdot 10^{-5}$ | $2.4334 \cdot 10^{-2}$ | $5.7184 \cdot 10^1$ | $1.3441 \cdot 10^5$ |
| 2300  | $4.4627 \cdot 10^{-9}$  | $1.0376 \cdot 10^{-5}$ | $2.4334 \cdot 10^{-2}$ | $5.7184 \cdot 10^1$ | $1.3441 \cdot 10^5$ |
| 2325  | $4.4063 \cdot 10^{-9}$  | $1.0355 \cdot 10^{-5}$ | $2.4334 \cdot 10^{-2}$ | $5.7184 \cdot 10^1$ | $1.3441 \cdot 10^5$ |
| 2350  | $4.2245 \cdot 10^{-9}$  | $1.0034 \cdot 10^{-5}$ | $2.3829 \cdot 10^{-2}$ | $5.6594 \cdot 10^1$ | $1.3441 \cdot 10^5$ |
| 2375  | $4.0499 \cdot 10^{-9}$  | $9.7196 \cdot 10^{-6}$ | $2.3328 \cdot 10^{-2}$ | $5.5985 \cdot 10^1$ | $1.3437 \cdot 10^5$ |
| 2400  | $3.8821 \cdot 10^{-9}$  | $9.4139 \cdot 10^{-6}$ | $2.2829 \cdot 10^{-2}$ | $5.5360 \cdot 10^1$ | $1.3425 \cdot 10^5$ |
| 2425  | $3.4833 \cdot 10^{-9}$  | $8.5339 \cdot 10^{-6}$ | $2.0909 \cdot 10^{-2}$ | $5.1225 \cdot 10^1$ | $1.2551 \cdot 10^5$ |
| 2450  | $3.0228 \cdot 10^{-9}$  | $7.4814 \cdot 10^{-6}$ | $1.8517 \cdot 10^{-2}$ | $4.5829 \cdot 10^1$ | $1.1343 \cdot 10^5$ |
| 2475  | $2.6279 \cdot 10^{-9}$  | $6.5696 \cdot 10^{-6}$ | $1.6424 \cdot 10^{-2}$ | $4.1060 \cdot 10^1$ | $1.0265 \cdot 10^5$ |
| 2500  | $2.2885 \cdot 10^{-9}$  | $5.7783 \cdot 10^{-6}$ | $1.4591 \cdot 10^{-2}$ | $3.6840 \cdot 10^1$ | $9.3021 \cdot 10^4$ |
| 2525  | $1.9873 \cdot 10^{-9}$  | $5.0676 \cdot 10^{-6}$ | $1.2923 \cdot 10^{-2}$ | $3.2952 \cdot 10^1$ | $8.4028 \cdot 10^4$ |
| 2550  | $1.7270 \cdot 10^{-9}$  | $4.4471 \cdot 10^{-6}$ | $1.1452 \cdot 10^{-2}$ | $2.9487 \cdot 10^1$ | $7.5928 \cdot 10^4$ |
| 2575  | $1.4992 \cdot 10^{-9}$  | $3.8979 \cdot 10^{-6}$ | $1.0135 \cdot 10^{-2}$ | $2.6350 \cdot 10^1$ | $6.8510 \cdot 10^4$ |
| 2600  | $1.3023 \cdot 10^{-9}$  | $3.4184 \cdot 10^{-6}$ | $8.9732 \cdot 10^{-3}$ | $2.3555 \cdot 10^1$ | $6.1831 \cdot 10^4$ |
| 2625  | $1.1314 \cdot 10^{-9}$  | $2.9981 \cdot 10^{-6}$ | $7.9450 \cdot 10^{-3}$ | $2.1055 \cdot 10^1$ | $5.5794 \cdot 10^4$ |
| 2650  | $9.8296 \cdot 10^{-10}$ | $2.6295 \cdot 10^{-6}$ | $7.0337 \cdot 10^{-3}$ | $1.8816 \cdot 10^1$ | $5.0331 \cdot 10^4$ |
| 2675  | $8.5432 \cdot 10^{-10}$ | $2.3067 \cdot 10^{-6}$ | $6.2280 \cdot 10^{-3}$ | $1.6816 \cdot 10^1$ | $4.5402 \cdot 10^4$ |
| 2700  | $7.4234 \cdot 10^{-10}$ | $2.0229 \cdot 10^{-6}$ | $5.5124 \cdot 10^{-3}$ | $1.5022 \cdot 10^1$ | $4.0933 \cdot 10^4$ |
| 2725  | $6.4498 \cdot 10^{-10}$ | $1.7737 \cdot 10^{-6}$ | $4.8777 \cdot 10^{-3}$ | $1.3414 \cdot 10^1$ | $3.6888 \cdot 10^4$ |
| 2750  | $5.6072 \cdot 10^{-10}$ | $1.5560 \cdot 10^{-6}$ | $4.3179 \cdot 10^{-3}$ | $1.1982 \cdot 10^1$ | $3.3250 \cdot 10^4$ |
| 2775  | $4.8730 \cdot 10^{-10}$ | $1.3645 \cdot 10^{-6}$ | $3.8204 \cdot 10^{-3}$ | $1.0698 \cdot 10^1$ | $2.9952 \cdot 10^4$ |

Continued on next page

Table 11 – continued from previous page

| $b_j$ | $\mathcal{B}_{j,1}$     | $\mathcal{B}_{j,2}$    | $\mathcal{B}_{j,3}$    | $\mathcal{B}_{j,4}$    | $\mathcal{B}_{j,5}$ |
|-------|-------------------------|------------------------|------------------------|------------------------|---------------------|
| 2800  | $4.2389 \cdot 10^{-10}$ | $1.1975 \cdot 10^{-6}$ | $3.3829 \cdot 10^{-3}$ | $9.5566 \cdot 10^0$    | $2.6998 \cdot 10^4$ |
| 2825  | $3.6912 \cdot 10^{-10}$ | $1.0520 \cdot 10^{-6}$ | $2.9982 \cdot 10^{-3}$ | $8.5447 \cdot 10^0$    | $2.4353 \cdot 10^4$ |
| 2850  | $3.2168 \cdot 10^{-10}$ | $9.2482 \cdot 10^{-7}$ | $2.6589 \cdot 10^{-3}$ | $7.6442 \cdot 10^0$    | $2.1977 \cdot 10^4$ |
| 2875  | $2.7953 \cdot 10^{-10}$ | $8.1063 \cdot 10^{-7}$ | $2.3509 \cdot 10^{-3}$ | $6.8174 \cdot 10^0$    | $1.9771 \cdot 10^4$ |
| 2900  | $2.4327 \cdot 10^{-10}$ | $7.1154 \cdot 10^{-7}$ | $2.0813 \cdot 10^{-3}$ | $6.0877 \cdot 10^0$    | $1.7807 \cdot 10^4$ |
| 2925  | $2.1141 \cdot 10^{-10}$ | $6.2364 \cdot 10^{-7}$ | $1.8398 \cdot 10^{-3}$ | $5.4272 \cdot 10^0$    | $1.6011 \cdot 10^4$ |
| 2950  | $1.8391 \cdot 10^{-10}$ | $5.4712 \cdot 10^{-7}$ | $1.6277 \cdot 10^{-3}$ | $4.8424 \cdot 10^0$    | $1.4406 \cdot 10^4$ |
| 2975  | $1.6015 \cdot 10^{-10}$ | $4.8044 \cdot 10^{-7}$ | $1.4414 \cdot 10^{-3}$ | $4.3240 \cdot 10^0$    | $1.2972 \cdot 10^4$ |
| 3000  | $1.3915 \cdot 10^{-10}$ | $4.2091 \cdot 10^{-7}$ | $1.2733 \cdot 10^{-3}$ | $3.8516 \cdot 10^0$    | $1.1651 \cdot 10^4$ |
| 3025  | $1.2115 \cdot 10^{-10}$ | $3.6950 \cdot 10^{-7}$ | $1.1270 \cdot 10^{-3}$ | $3.4373 \cdot 10^0$    | $1.0484 \cdot 10^4$ |
| 3050  | $1.0531 \cdot 10^{-10}$ | $3.2382 \cdot 10^{-7}$ | $9.9573 \cdot 10^{-4}$ | $3.0619 \cdot 10^0$    | $9.4153 \cdot 10^3$ |
| 3075  | $9.1684 \cdot 10^{-11}$ | $2.8422 \cdot 10^{-7}$ | $8.8109 \cdot 10^{-4}$ | $2.7314 \cdot 10^0$    | $8.4672 \cdot 10^3$ |
| 3100  | $7.9793 \cdot 10^{-11}$ | $2.4936 \cdot 10^{-7}$ | $7.7923 \cdot 10^{-4}$ | $2.4351 \cdot 10^0$    | $7.6097 \cdot 10^3$ |
| 3125  | $6.9396 \cdot 10^{-11}$ | $2.1860 \cdot 10^{-7}$ | $6.8859 \cdot 10^{-4}$ | $2.1691 \cdot 10^0$    | $6.8325 \cdot 10^3$ |
| 3150  | $6.0410 \cdot 10^{-11}$ | $1.9180 \cdot 10^{-7}$ | $6.0897 \cdot 10^{-4}$ | $1.9335 \cdot 10^0$    | $6.1388 \cdot 10^3$ |
| 3175  | $5.2572 \cdot 10^{-11}$ | $1.6824 \cdot 10^{-7}$ | $5.3834 \cdot 10^{-4}$ | $1.7227 \cdot 10^0$    | $5.5126 \cdot 10^3$ |
| 3200  | $4.5782 \cdot 10^{-11}$ | $1.4765 \cdot 10^{-7}$ | $4.7616 \cdot 10^{-4}$ | $1.5357 \cdot 10^0$    | $4.9524 \cdot 10^3$ |
| 3225  | $3.9902 \cdot 10^{-11}$ | $1.2968 \cdot 10^{-7}$ | $4.2146 \cdot 10^{-4}$ | $1.3698 \cdot 10^0$    | $4.4517 \cdot 10^3$ |
| 3250  | $3.4801 \cdot 10^{-11}$ | $1.1398 \cdot 10^{-7}$ | $3.7326 \cdot 10^{-4}$ | $1.2225 \cdot 10^0$    | $4.0034 \cdot 10^3$ |
| 3275  | $3.0332 \cdot 10^{-11}$ | $1.0010 \cdot 10^{-7}$ | $3.3031 \cdot 10^{-4}$ | $1.0901 \cdot 10^0$    | $3.5971 \cdot 10^3$ |
| 3300  | $2.6412 \cdot 10^{-11}$ | $8.7820 \cdot 10^{-8}$ | $2.9200 \cdot 10^{-4}$ | $9.7090 \cdot 10^{-1}$ | $3.2283 \cdot 10^3$ |
| 3325  | $2.3015 \cdot 10^{-11}$ | $7.7100 \cdot 10^{-8}$ | $2.5829 \cdot 10^{-4}$ | $8.6526 \cdot 10^{-1}$ | $2.8987 \cdot 10^3$ |
| 3350  | $2.0043 \cdot 10^{-11}$ | $6.7644 \cdot 10^{-8}$ | $2.2830 \cdot 10^{-4}$ | $7.7051 \cdot 10^{-1}$ | $2.6005 \cdot 10^3$ |
| 3375  | $1.7453 \cdot 10^{-11}$ | $5.9340 \cdot 10^{-8}$ | $2.0176 \cdot 10^{-4}$ | $6.8597 \cdot 10^{-1}$ | $2.3323 \cdot 10^3$ |
| 3400  | $1.5212 \cdot 10^{-11}$ | $5.2100 \cdot 10^{-8}$ | $1.7844 \cdot 10^{-4}$ | $6.1116 \cdot 10^{-1}$ | $2.0933 \cdot 10^3$ |
| 3425  | $1.3267 \cdot 10^{-11}$ | $4.5769 \cdot 10^{-8}$ | $1.5791 \cdot 10^{-4}$ | $5.4476 \cdot 10^{-1}$ | $1.8795 \cdot 10^3$ |
| 3450  | $1.1555 \cdot 10^{-11}$ | $4.0151 \cdot 10^{-8}$ | $1.3953 \cdot 10^{-4}$ | $4.8485 \cdot 10^{-1}$ | $1.6849 \cdot 10^3$ |
| 3475  | $1.0059 \cdot 10^{-11}$ | $3.5207 \cdot 10^{-8}$ | $1.2323 \cdot 10^{-4}$ | $4.3128 \cdot 10^{-1}$ | $1.5095 \cdot 10^3$ |
| 3500  | $8.7646 \cdot 10^{-12}$ | $3.0896 \cdot 10^{-8}$ | $1.0891 \cdot 10^{-4}$ | $3.8390 \cdot 10^{-1}$ | $1.3533 \cdot 10^3$ |
| 3525  | $7.6403 \cdot 10^{-12}$ | $2.7124 \cdot 10^{-8}$ | $9.6287 \cdot 10^{-5}$ | $3.4182 \cdot 10^{-1}$ | $1.2135 \cdot 10^3$ |
| 3550  | $6.6608 \cdot 10^{-12}$ | $2.3813 \cdot 10^{-8}$ | $8.5129 \cdot 10^{-5}$ | $3.0434 \cdot 10^{-1}$ | $1.0880 \cdot 10^3$ |
| 3575  | $5.8042 \cdot 10^{-12}$ | $2.0896 \cdot 10^{-8}$ | $7.5223 \cdot 10^{-5}$ | $2.7080 \cdot 10^{-1}$ | $9.7488 \cdot 10^2$ |
| 3600  | $5.0622 \cdot 10^{-12}$ | $1.8351 \cdot 10^{-8}$ | $6.6520 \cdot 10^{-5}$ | $2.4114 \cdot 10^{-1}$ | $8.7411 \cdot 10^2$ |
| 3625  | $4.4166 \cdot 10^{-12}$ | $1.6121 \cdot 10^{-8}$ | $5.8840 \cdot 10^{-5}$ | $2.1477 \cdot 10^{-1}$ | $7.8389 \cdot 10^2$ |
| 3650  | $3.8475 \cdot 10^{-12}$ | $1.4140 \cdot 10^{-8}$ | $5.1963 \cdot 10^{-5}$ | $1.9097 \cdot 10^{-1}$ | $7.0179 \cdot 10^2$ |
| 3675  | $3.3561 \cdot 10^{-12}$ | $1.2418 \cdot 10^{-8}$ | $4.5944 \cdot 10^{-5}$ | $1.7000 \cdot 10^{-1}$ | $6.2898 \cdot 10^2$ |
| 3700  | $2.9296 \cdot 10^{-12}$ | $1.0913 \cdot 10^{-8}$ | $4.0650 \cdot 10^{-5}$ | $1.5142 \cdot 10^{-1}$ | $5.6404 \cdot 10^2$ |
| 3725  | $2.5580 \cdot 10^{-12}$ | $9.5924 \cdot 10^{-9}$ | $3.5972 \cdot 10^{-5}$ | $1.3490 \cdot 10^{-1}$ | $5.0585 \cdot 10^2$ |
| 3750  | $2.2347 \cdot 10^{-12}$ | $8.4358 \cdot 10^{-9}$ | $3.1845 \cdot 10^{-5}$ | $1.2022 \cdot 10^{-1}$ | $4.5381 \cdot 10^2$ |
| 3775  | $1.9514 \cdot 10^{-12}$ | $7.4151 \cdot 10^{-9}$ | $2.8178 \cdot 10^{-5}$ | $1.0708 \cdot 10^{-1}$ | $4.0689 \cdot 10^2$ |
| 3800  | $1.7020 \cdot 10^{-12}$ | $6.5100 \cdot 10^{-9}$ | $2.4901 \cdot 10^{-5}$ | $9.5245 \cdot 10^{-2}$ | $3.6431 \cdot 10^2$ |
| 3825  | $1.4855 \cdot 10^{-12}$ | $5.7189 \cdot 10^{-9}$ | $2.2018 \cdot 10^{-5}$ | $8.4768 \cdot 10^{-2}$ | $3.2636 \cdot 10^2$ |
| 3850  | $1.2973 \cdot 10^{-12}$ | $5.0267 \cdot 10^{-9}$ | $1.9479 \cdot 10^{-5}$ | $7.5479 \cdot 10^{-2}$ | $2.9249 \cdot 10^2$ |
| 3875  | $1.1314 \cdot 10^{-12}$ | $4.4124 \cdot 10^{-9}$ | $1.7209 \cdot 10^{-5}$ | $6.7112 \cdot 10^{-2}$ | $2.6174 \cdot 10^2$ |
| 3900  | $9.8800 \cdot 10^{-13}$ | $3.8779 \cdot 10^{-9}$ | $1.5221 \cdot 10^{-5}$ | $5.9742 \cdot 10^{-2}$ | $2.3449 \cdot 10^2$ |
| 3925  | $8.6323 \cdot 10^{-13}$ | $3.4098 \cdot 10^{-9}$ | $1.3469 \cdot 10^{-5}$ | $5.3201 \cdot 10^{-2}$ | $2.1015 \cdot 10^2$ |
| 3950  | $7.5450 \cdot 10^{-13}$ | $2.9992 \cdot 10^{-9}$ | $1.1922 \cdot 10^{-5}$ | $4.7388 \cdot 10^{-2}$ | $1.8837 \cdot 10^2$ |
| 3975  | $6.5788 \cdot 10^{-13}$ | $2.6316 \cdot 10^{-9}$ | $1.0527 \cdot 10^{-5}$ | $4.2105 \cdot 10^{-2}$ | $1.6842 \cdot 10^2$ |
| 4000  | $5.7410 \cdot 10^{-13}$ | $2.3108 \cdot 10^{-9}$ | $9.3007 \cdot 10^{-6}$ | $3.7436 \cdot 10^{-2}$ | $1.5068 \cdot 10^2$ |
| 4025  | $5.0265 \cdot 10^{-13}$ | $2.0358 \cdot 10^{-9}$ | $8.2446 \cdot 10^{-6}$ | $3.3391 \cdot 10^{-2}$ | $1.3524 \cdot 10^2$ |
| 4050  | $4.3803 \cdot 10^{-13}$ | $1.7850 \cdot 10^{-9}$ | $7.2737 \cdot 10^{-6}$ | $2.9641 \cdot 10^{-2}$ | $1.2079 \cdot 10^2$ |
| 4075  | $3.8285 \cdot 10^{-13}$ | $1.5697 \cdot 10^{-9}$ | $6.4357 \cdot 10^{-6}$ | $2.6387 \cdot 10^{-2}$ | $1.0819 \cdot 10^2$ |
| 4100  | $3.3428 \cdot 10^{-13}$ | $1.3789 \cdot 10^{-9}$ | $5.6880 \cdot 10^{-6}$ | $2.3463 \cdot 10^{-2}$ | $9.6784 \cdot 10^1$ |
| 4125  | $2.9206 \cdot 10^{-13}$ | $1.2121 \cdot 10^{-9}$ | $5.0300 \cdot 10^{-6}$ | $2.0875 \cdot 10^{-2}$ | $8.6629 \cdot 10^1$ |
| 4150  | $2.5566 \cdot 10^{-13}$ | $1.0674 \cdot 10^{-9}$ | $4.4564 \cdot 10^{-6}$ | $1.8606 \cdot 10^{-2}$ | $7.7677 \cdot 10^1$ |

Continued on next page

Table 11 – continued from previous page

| $b_j$ | $\mathcal{B}_{j,1}$     | $\mathcal{B}_{j,2}$     | $\mathcal{B}_{j,3}$     | $\mathcal{B}_{j,4}$    | $\mathcal{B}_{j,5}$    |
|-------|-------------------------|-------------------------|-------------------------|------------------------|------------------------|
| 4175  | $2.2310 \cdot 10^{-13}$ | $9.3698 \cdot 10^{-10}$ | $3.9354 \cdot 10^{-6}$  | $1.6529 \cdot 10^{-2}$ | $6.9419 \cdot 10^1$    |
| 4200  | $1.9496 \cdot 10^{-13}$ | $8.2370 \cdot 10^{-10}$ | $3.4802 \cdot 10^{-6}$  | $1.4704 \cdot 10^{-2}$ | $6.2123 \cdot 10^1$    |
| 4225  | $1.7047 \cdot 10^{-13}$ | $7.2449 \cdot 10^{-10}$ | $3.0791 \cdot 10^{-6}$  | $1.3087 \cdot 10^{-2}$ | $5.5616 \cdot 10^1$    |
| 4250  | $1.4913 \cdot 10^{-13}$ | $6.3752 \cdot 10^{-10}$ | $2.7254 \cdot 10^{-6}$  | $1.1651 \cdot 10^{-2}$ | $4.9808 \cdot 10^1$    |
| 4275  | $1.3037 \cdot 10^{-13}$ | $5.6056 \cdot 10^{-10}$ | $2.4104 \cdot 10^{-6}$  | $1.0365 \cdot 10^{-2}$ | $4.4569 \cdot 10^1$    |
| 4300  | $1.1396 \cdot 10^{-13}$ | $4.9288 \cdot 10^{-10}$ | $2.1317 \cdot 10^{-6}$  | $9.2196 \cdot 10^{-3}$ | $3.9875 \cdot 10^1$    |
| 4325  | $9.9670 \cdot 10^{-14}$ | $4.3357 \cdot 10^{-10}$ | $1.8860 \cdot 10^{-6}$  | $8.2041 \cdot 10^{-3}$ | $3.5688 \cdot 10^1$    |
| 4350  | $8.7210 \cdot 10^{-14}$ | $3.8155 \cdot 10^{-10}$ | $1.6693 \cdot 10^{-6}$  | $7.3030 \cdot 10^{-3}$ | $3.1951 \cdot 10^1$    |
| 4375  | $7.6274 \cdot 10^{-14}$ | $3.3561 \cdot 10^{-10}$ | $1.4767 \cdot 10^{-6}$  | $6.4974 \cdot 10^{-3}$ | $2.8589 \cdot 10^1$    |
| 4400  | $6.6744 \cdot 10^{-14}$ | $2.9534 \cdot 10^{-10}$ | $1.3069 \cdot 10^{-6}$  | $5.7830 \cdot 10^{-3}$ | $2.5590 \cdot 10^1$    |
| 4425  | $5.8436 \cdot 10^{-14}$ | $2.6005 \cdot 10^{-10}$ | $1.1572 \cdot 10^{-6}$  | $5.1495 \cdot 10^{-3}$ | $2.2916 \cdot 10^1$    |
| 4450  | $5.1175 \cdot 10^{-14}$ | $2.2901 \cdot 10^{-10}$ | $1.0248 \cdot 10^{-6}$  | $4.5860 \cdot 10^{-3}$ | $2.0523 \cdot 10^1$    |
| 4475  | $4.4832 \cdot 10^{-14}$ | $2.0175 \cdot 10^{-10}$ | $9.0785 \cdot 10^{-7}$  | $4.0853 \cdot 10^{-3}$ | $1.8384 \cdot 10^1$    |
| 4500  | $3.9291 \cdot 10^{-14}$ | $1.7779 \cdot 10^{-10}$ | $8.0450 \cdot 10^{-7}$  | $3.6404 \cdot 10^{-3}$ | $1.6473 \cdot 10^1$    |
| 4525  | $3.4446 \cdot 10^{-14}$ | $1.5673 \cdot 10^{-10}$ | $7.1312 \cdot 10^{-7}$  | $3.2447 \cdot 10^{-3}$ | $1.4764 \cdot 10^1$    |
| 4550  | $3.0156 \cdot 10^{-14}$ | $1.3797 \cdot 10^{-10}$ | $6.3117 \cdot 10^{-7}$  | $2.8876 \cdot 10^{-3}$ | $1.3211 \cdot 10^1$    |
| 4575  | $2.6404 \cdot 10^{-14}$ | $1.2146 \cdot 10^{-10}$ | $5.5871 \cdot 10^{-7}$  | $2.5701 \cdot 10^{-3}$ | $1.1823 \cdot 10^1$    |
| 4600  | $2.3158 \cdot 10^{-14}$ | $1.0711 \cdot 10^{-10}$ | $4.9535 \cdot 10^{-7}$  | $2.2910 \cdot 10^{-3}$ | $1.0596 \cdot 10^1$    |
| 4625  | $2.0260 \cdot 10^{-14}$ | $9.4207 \cdot 10^{-11}$ | $4.3806 \cdot 10^{-7}$  | $2.0370 \cdot 10^{-3}$ | $9.4720 \cdot 10^0$    |
| 4650  | $1.7754 \cdot 10^{-14}$ | $8.2997 \cdot 10^{-11}$ | $3.8801 \cdot 10^{-7}$  | $1.8140 \cdot 10^{-3}$ | $8.4802 \cdot 10^0$    |
| 4675  | $1.5563 \cdot 10^{-14}$ | $7.3145 \cdot 10^{-11}$ | $3.4378 \cdot 10^{-7}$  | $1.6158 \cdot 10^{-3}$ | $7.5941 \cdot 10^0$    |
| 4700  | $1.3648 \cdot 10^{-14}$ | $6.4487 \cdot 10^{-11}$ | $3.0470 \cdot 10^{-7}$  | $1.4397 \cdot 10^{-3}$ | $6.8026 \cdot 10^0$    |
| 4725  | $1.1977 \cdot 10^{-14}$ | $5.6887 \cdot 10^{-11}$ | $2.7022 \cdot 10^{-7}$  | $1.2836 \cdot 10^{-3}$ | $6.0967 \cdot 10^0$    |
| 4750  | $1.0492 \cdot 10^{-14}$ | $5.0095 \cdot 10^{-11}$ | $2.3921 \cdot 10^{-7}$  | $1.1422 \cdot 10^{-3}$ | $5.4540 \cdot 10^0$    |
| 4775  | $9.1894 \cdot 10^{-15}$ | $4.4109 \cdot 10^{-11}$ | $2.1173 \cdot 10^{-7}$  | $1.0163 \cdot 10^{-3}$ | $4.8782 \cdot 10^0$    |
| 4800  | $8.0537 \cdot 10^{-15}$ | $3.8859 \cdot 10^{-11}$ | $1.8750 \cdot 10^{-7}$  | $9.0467 \cdot 10^{-4}$ | $4.3650 \cdot 10^0$    |
| 4825  | $7.0615 \cdot 10^{-15}$ | $3.4248 \cdot 10^{-11}$ | $1.6611 \cdot 10^{-7}$  | $8.0560 \cdot 10^{-4}$ | $3.9072 \cdot 10^0$    |
| 4850  | $6.1951 \cdot 10^{-15}$ | $3.0202 \cdot 10^{-11}$ | $1.4724 \cdot 10^{-7}$  | $7.1775 \cdot 10^{-4}$ | $3.4991 \cdot 10^0$    |
| 4875  | $5.4361 \cdot 10^{-15}$ | $2.6637 \cdot 10^{-11}$ | $1.3053 \cdot 10^{-7}$  | $6.3955 \cdot 10^{-4}$ | $3.1338 \cdot 10^0$    |
| 4900  | $4.7721 \cdot 10^{-15}$ | $2.3503 \cdot 10^{-11}$ | $1.1575 \cdot 10^{-7}$  | $5.7006 \cdot 10^{-4}$ | $2.8076 \cdot 10^0$    |
| 4925  | $4.1878 \cdot 10^{-15}$ | $2.0730 \cdot 10^{-11}$ | $1.0262 \cdot 10^{-7}$  | $5.0793 \cdot 10^{-4}$ | $2.5143 \cdot 10^0$    |
| 4950  | $3.6731 \cdot 10^{-15}$ | $1.8274 \cdot 10^{-11}$ | $9.0911 \cdot 10^{-8}$  | $4.5228 \cdot 10^{-4}$ | $2.2501 \cdot 10^0$    |
| 4975  | $3.2229 \cdot 10^{-15}$ | $1.6115 \cdot 10^{-11}$ | $8.0572 \cdot 10^{-8}$  | $4.0286 \cdot 10^{-4}$ | $2.0143 \cdot 10^0$    |
| 5000  | $2.8715 \cdot 10^{-15}$ | $1.4645 \cdot 10^{-11}$ | $7.4687 \cdot 10^{-8}$  | $3.8091 \cdot 10^{-4}$ | $1.9426 \cdot 10^0$    |
| 5100  | $1.7087 \cdot 10^{-15}$ | $8.8850 \cdot 10^{-12}$ | $4.6202 \cdot 10^{-8}$  | $2.4025 \cdot 10^{-4}$ | $1.2493 \cdot 10^0$    |
| 5200  | $1.0185 \cdot 10^{-15}$ | $5.3981 \cdot 10^{-12}$ | $2.8610 \cdot 10^{-8}$  | $1.5164 \cdot 10^{-4}$ | $8.0365 \cdot 10^{-1}$ |
| 5300  | $6.0977 \cdot 10^{-16}$ | $3.2928 \cdot 10^{-12}$ | $1.7781 \cdot 10^{-8}$  | $9.6016 \cdot 10^{-5}$ | $5.1849 \cdot 10^{-1}$ |
| 5400  | $3.6472 \cdot 10^{-16}$ | $2.0060 \cdot 10^{-12}$ | $1.1033 \cdot 10^{-8}$  | $6.0680 \cdot 10^{-5}$ | $3.3374 \cdot 10^{-1}$ |
| 5500  | $2.1916 \cdot 10^{-16}$ | $1.2273 \cdot 10^{-12}$ | $6.8727 \cdot 10^{-9}$  | $3.8488 \cdot 10^{-5}$ | $2.1553 \cdot 10^{-1}$ |
| 5600  | $1.3218 \cdot 10^{-16}$ | $7.5337 \cdot 10^{-13}$ | $4.2943 \cdot 10^{-9}$  | $2.4477 \cdot 10^{-5}$ | $1.3952 \cdot 10^{-1}$ |
| 5700  | $8.0079 \cdot 10^{-17}$ | $4.6446 \cdot 10^{-13}$ | $2.6939 \cdot 10^{-9}$  | $1.5625 \cdot 10^{-5}$ | $9.0621 \cdot 10^{-2}$ |
| 5800  | $4.8519 \cdot 10^{-17}$ | $2.8626 \cdot 10^{-13}$ | $1.6890 \cdot 10^{-9}$  | $9.9647 \cdot 10^{-6}$ | $5.8792 \cdot 10^{-2}$ |
| 5900  | $2.9483 \cdot 10^{-17}$ | $1.7690 \cdot 10^{-13}$ | $1.0614 \cdot 10^{-9}$  | $6.3682 \cdot 10^{-6}$ | $3.8209 \cdot 10^{-2}$ |
| 6000  | $1.7952 \cdot 10^{-17}$ | $1.0951 \cdot 10^{-13}$ | $6.6798 \cdot 10^{-10}$ | $4.0747 \cdot 10^{-6}$ | $2.4856 \cdot 10^{-2}$ |
| 6100  | $1.0988 \cdot 10^{-17}$ | $6.8120 \cdot 10^{-14}$ | $4.2235 \cdot 10^{-10}$ | $2.6186 \cdot 10^{-6}$ | $1.6235 \cdot 10^{-2}$ |
| 6200  | $6.7178 \cdot 10^{-18}$ | $4.2322 \cdot 10^{-14}$ | $2.6663 \cdot 10^{-10}$ | $1.6798 \cdot 10^{-6}$ | $1.0583 \cdot 10^{-2}$ |
| 6300  | $4.1268 \cdot 10^{-18}$ | $2.6412 \cdot 10^{-14}$ | $1.6904 \cdot 10^{-10}$ | $1.0818 \cdot 10^{-6}$ | $6.9236 \cdot 10^{-3}$ |
| 6400  | $2.5481 \cdot 10^{-18}$ | $1.6563 \cdot 10^{-14}$ | $1.0766 \cdot 10^{-10}$ | $6.9977 \cdot 10^{-7}$ | $4.5485 \cdot 10^{-3}$ |
| 6500  | $1.5741 \cdot 10^{-18}$ | $1.0389 \cdot 10^{-14}$ | $6.8566 \cdot 10^{-11}$ | $4.5254 \cdot 10^{-7}$ | $2.9868 \cdot 10^{-3}$ |
| 6600  | $9.7287 \cdot 10^{-19}$ | $6.5182 \cdot 10^{-15}$ | $4.3672 \cdot 10^{-11}$ | $2.9261 \cdot 10^{-7}$ | $1.9605 \cdot 10^{-3}$ |
| 6700  | $6.0447 \cdot 10^{-19}$ | $4.1104 \cdot 10^{-15}$ | $2.7951 \cdot 10^{-11}$ | $1.9007 \cdot 10^{-7}$ | $1.2925 \cdot 10^{-3}$ |
| 6800  | $3.7652 \cdot 10^{-19}$ | $2.5980 \cdot 10^{-15}$ | $1.7926 \cdot 10^{-11}$ | $1.2369 \cdot 10^{-7}$ | $8.5345 \cdot 10^{-4}$ |
| 6900  | $2.3555 \cdot 10^{-19}$ | $1.6488 \cdot 10^{-15}$ | $1.1542 \cdot 10^{-11}$ | $8.0791 \cdot 10^{-8}$ | $5.6554 \cdot 10^{-4}$ |
| 7000  | $1.4744 \cdot 10^{-19}$ | $1.0468 \cdot 10^{-15}$ | $7.4322 \cdot 10^{-12}$ | $5.2769 \cdot 10^{-8}$ | $3.7466 \cdot 10^{-4}$ |
| 7100  | $9.2826 \cdot 10^{-20}$ | $6.6835 \cdot 10^{-16}$ | $4.8121 \cdot 10^{-12}$ | $3.4647 \cdot 10^{-8}$ | $2.4946 \cdot 10^{-4}$ |

Continued on next page

Table 11 – continued from previous page

| $b_j$ | $\mathcal{B}_{j,1}$     | $\mathcal{B}_{j,2}$     | $\mathcal{B}_{j,3}$     | $\mathcal{B}_{j,4}$     | $\mathcal{B}_{j,5}$     |
|-------|-------------------------|-------------------------|-------------------------|-------------------------|-------------------------|
| 7200  | $5.8601 \cdot 10^{-20}$ | $4.2779 \cdot 10^{-16}$ | $3.1229 \cdot 10^{-12}$ | $2.2797 \cdot 10^{-8}$  | $1.6642 \cdot 10^{-4}$  |
| 7300  | $3.7014 \cdot 10^{-20}$ | $2.7391 \cdot 10^{-16}$ | $2.0269 \cdot 10^{-12}$ | $1.4999 \cdot 10^{-8}$  | $1.1100 \cdot 10^{-4}$  |
| 7400  | $2.3489 \cdot 10^{-20}$ | $1.7617 \cdot 10^{-16}$ | $1.3213 \cdot 10^{-12}$ | $9.9092 \cdot 10^{-9}$  | $7.4319 \cdot 10^{-5}$  |
| 7500  | $1.4908 \cdot 10^{-20}$ | $1.1330 \cdot 10^{-16}$ | $8.6105 \cdot 10^{-13}$ | $6.5440 \cdot 10^{-9}$  | $4.9735 \cdot 10^{-5}$  |
| 7600  | $9.4822 \cdot 10^{-21}$ | $7.3013 \cdot 10^{-17}$ | $5.6220 \cdot 10^{-13}$ | $4.3290 \cdot 10^{-9}$  | $3.3333 \cdot 10^{-5}$  |
| 7700  | $6.0570 \cdot 10^{-21}$ | $4.7245 \cdot 10^{-17}$ | $3.6851 \cdot 10^{-13}$ | $2.8744 \cdot 10^{-9}$  | $2.2420 \cdot 10^{-5}$  |
| 7800  | $3.8812 \cdot 10^{-21}$ | $3.0661 \cdot 10^{-17}$ | $2.4223 \cdot 10^{-13}$ | $1.9136 \cdot 10^{-9}$  | $1.5117 \cdot 10^{-5}$  |
| 7900  | $2.4928 \cdot 10^{-21}$ | $1.9943 \cdot 10^{-17}$ | $1.5954 \cdot 10^{-13}$ | $1.2764 \cdot 10^{-9}$  | $1.0211 \cdot 10^{-5}$  |
| 8000  | $1.6007 \cdot 10^{-21}$ | $1.2966 \cdot 10^{-17}$ | $1.0502 \cdot 10^{-13}$ | $8.5065 \cdot 10^{-10}$ | $6.8903 \cdot 10^{-6}$  |
| 8100  | $1.0327 \cdot 10^{-21}$ | $8.4675 \cdot 10^{-18}$ | $6.9433 \cdot 10^{-14}$ | $5.6935 \cdot 10^{-10}$ | $4.6687 \cdot 10^{-6}$  |
| 8200  | $6.6829 \cdot 10^{-22}$ | $5.5468 \cdot 10^{-18}$ | $4.6038 \cdot 10^{-14}$ | $3.8212 \cdot 10^{-10}$ | $3.1716 \cdot 10^{-6}$  |
| 8300  | $4.3257 \cdot 10^{-22}$ | $3.6336 \cdot 10^{-18}$ | $3.0523 \cdot 10^{-14}$ | $2.5639 \cdot 10^{-10}$ | $2.1537 \cdot 10^{-6}$  |
| 8400  | $2.8105 \cdot 10^{-22}$ | $2.3889 \cdot 10^{-18}$ | $2.0306 \cdot 10^{-14}$ | $1.7260 \cdot 10^{-10}$ | $1.4671 \cdot 10^{-6}$  |
| 8500  | $1.8316 \cdot 10^{-22}$ | $1.5752 \cdot 10^{-18}$ | $1.3547 \cdot 10^{-14}$ | $1.1650 \cdot 10^{-10}$ | $1.0019 \cdot 10^{-6}$  |
| 8600  | $1.1981 \cdot 10^{-22}$ | $1.0424 \cdot 10^{-18}$ | $9.0682 \cdot 10^{-15}$ | $7.8894 \cdot 10^{-11}$ | $6.8638 \cdot 10^{-7}$  |
| 8700  | $7.8221 \cdot 10^{-23}$ | $6.8834 \cdot 10^{-19}$ | $6.0574 \cdot 10^{-15}$ | $5.3305 \cdot 10^{-11}$ | $4.6909 \cdot 10^{-7}$  |
| 8800  | $5.1585 \cdot 10^{-23}$ | $4.5911 \cdot 10^{-19}$ | $4.0861 \cdot 10^{-15}$ | $3.6366 \cdot 10^{-11}$ | $3.2366 \cdot 10^{-7}$  |
| 8900  | $3.3883 \cdot 10^{-23}$ | $3.0495 \cdot 10^{-19}$ | $2.7445 \cdot 10^{-15}$ | $2.4701 \cdot 10^{-11}$ | $2.2231 \cdot 10^{-7}$  |
| 9000  | $2.2253 \cdot 10^{-23}$ | $2.0250 \cdot 10^{-19}$ | $1.8428 \cdot 10^{-15}$ | $1.6769 \cdot 10^{-11}$ | $1.5260 \cdot 10^{-7}$  |
| 9100  | $1.4642 \cdot 10^{-23}$ | $1.3470 \cdot 10^{-19}$ | $1.2393 \cdot 10^{-15}$ | $1.1401 \cdot 10^{-11}$ | $1.0489 \cdot 10^{-7}$  |
| 9200  | $9.6778 \cdot 10^{-24}$ | $9.0003 \cdot 10^{-20}$ | $8.3703 \cdot 10^{-16}$ | $7.7844 \cdot 10^{-12}$ | $7.2395 \cdot 10^{-8}$  |
| 9300  | $6.4195 \cdot 10^{-24}$ | $6.0344 \cdot 10^{-20}$ | $5.6723 \cdot 10^{-16}$ | $5.3320 \cdot 10^{-12}$ | $5.0121 \cdot 10^{-8}$  |
| 9400  | $4.2972 \cdot 10^{-24}$ | $4.0823 \cdot 10^{-20}$ | $3.8782 \cdot 10^{-16}$ | $3.6843 \cdot 10^{-12}$ | $3.5001 \cdot 10^{-8}$  |
| 9500  | $2.8513 \cdot 10^{-24}$ | $2.7372 \cdot 10^{-20}$ | $2.6277 \cdot 10^{-16}$ | $2.5226 \cdot 10^{-12}$ | $2.4217 \cdot 10^{-8}$  |
| 9600  | $1.9059 \cdot 10^{-24}$ | $1.8487 \cdot 10^{-20}$ | $1.7933 \cdot 10^{-16}$ | $1.7395 \cdot 10^{-12}$ | $1.6873 \cdot 10^{-8}$  |
| 9700  | $1.2689 \cdot 10^{-24}$ | $1.2436 \cdot 10^{-20}$ | $1.2187 \cdot 10^{-16}$ | $1.1943 \cdot 10^{-12}$ | $1.1704 \cdot 10^{-8}$  |
| 9800  | $8.4841 \cdot 10^{-25}$ | $8.3993 \cdot 10^{-21}$ | $8.3153 \cdot 10^{-17}$ | $8.2321 \cdot 10^{-13}$ | $8.1498 \cdot 10^{-9}$  |
| 9900  | $5.7396 \cdot 10^{-25}$ | $5.7396 \cdot 10^{-21}$ | $5.7396 \cdot 10^{-17}$ | $5.7396 \cdot 10^{-13}$ | $5.7396 \cdot 10^{-9}$  |
| 10000 | $3.8228 \cdot 10^{-25}$ | $3.8610 \cdot 10^{-21}$ | $3.8997 \cdot 10^{-17}$ | $3.9387 \cdot 10^{-13}$ | $3.9780 \cdot 10^{-9}$  |
| 10100 | $2.5746 \cdot 10^{-25}$ | $2.6260 \cdot 10^{-21}$ | $2.6786 \cdot 10^{-17}$ | $2.7321 \cdot 10^{-13}$ | $2.7868 \cdot 10^{-9}$  |
| 10200 | $1.7389 \cdot 10^{-25}$ | $1.7911 \cdot 10^{-21}$ | $1.8448 \cdot 10^{-17}$ | $1.9002 \cdot 10^{-13}$ | $1.9572 \cdot 10^{-9}$  |
| 10300 | $1.1734 \cdot 10^{-25}$ | $1.2204 \cdot 10^{-21}$ | $1.2692 \cdot 10^{-17}$ | $1.3199 \cdot 10^{-13}$ | $1.3727 \cdot 10^{-9}$  |
| 10400 | $7.9556 \cdot 10^{-26}$ | $8.3534 \cdot 10^{-22}$ | $8.7711 \cdot 10^{-18}$ | $9.2096 \cdot 10^{-14}$ | $9.6701 \cdot 10^{-10}$ |
| 10500 | $5.4077 \cdot 10^{-26}$ | $5.7321 \cdot 10^{-22}$ | $6.0761 \cdot 10^{-18}$ | $6.4406 \cdot 10^{-14}$ | $6.8270 \cdot 10^{-10}$ |
| 10600 | $3.6845 \cdot 10^{-26}$ | $3.9424 \cdot 10^{-22}$ | $4.2184 \cdot 10^{-18}$ | $4.5137 \cdot 10^{-14}$ | $4.8296 \cdot 10^{-10}$ |
| 10700 | $2.5150 \cdot 10^{-26}$ | $2.7162 \cdot 10^{-22}$ | $2.9335 \cdot 10^{-18}$ | $3.1682 \cdot 10^{-14}$ | $3.4217 \cdot 10^{-10}$ |
| 10800 | $1.7201 \cdot 10^{-26}$ | $1.8749 \cdot 10^{-22}$ | $2.0437 \cdot 10^{-18}$ | $2.2276 \cdot 10^{-14}$ | $2.4281 \cdot 10^{-10}$ |
| 10900 | $1.1640 \cdot 10^{-26}$ | $1.2803 \cdot 10^{-22}$ | $1.4084 \cdot 10^{-18}$ | $1.5492 \cdot 10^{-14}$ | $1.7041 \cdot 10^{-10}$ |
| 11000 | $7.9284 \cdot 10^{-27}$ | $8.8005 \cdot 10^{-23}$ | $9.7685 \cdot 10^{-19}$ | $1.0844 \cdot 10^{-14}$ | $1.2036 \cdot 10^{-10}$ |
| 11100 | $5.4156 \cdot 10^{-27}$ | $6.0655 \cdot 10^{-23}$ | $6.7933 \cdot 10^{-19}$ | $7.6085 \cdot 10^{-15}$ | $8.5215 \cdot 10^{-11}$ |
| 11200 | $3.7120 \cdot 10^{-27}$ | $4.1946 \cdot 10^{-23}$ | $4.7398 \cdot 10^{-19}$ | $5.3560 \cdot 10^{-15}$ | $6.0523 \cdot 10^{-11}$ |
| 11300 | $2.5509 \cdot 10^{-27}$ | $2.9080 \cdot 10^{-23}$ | $3.3152 \cdot 10^{-19}$ | $3.7793 \cdot 10^{-15}$ | $4.3084 \cdot 10^{-11}$ |
| 11400 | $1.7570 \cdot 10^{-27}$ | $2.0205 \cdot 10^{-23}$ | $2.3236 \cdot 10^{-19}$ | $2.6721 \cdot 10^{-15}$ | $3.0729 \cdot 10^{-11}$ |
| 11500 | $1.2103 \cdot 10^{-27}$ | $1.4039 \cdot 10^{-23}$ | $1.6285 \cdot 10^{-19}$ | $1.8891 \cdot 10^{-15}$ | $2.1913 \cdot 10^{-11}$ |
| 11600 | $8.3445 \cdot 10^{-28}$ | $9.7630 \cdot 10^{-24}$ | $1.1423 \cdot 10^{-19}$ | $1.3365 \cdot 10^{-15}$ | $1.5637 \cdot 10^{-11}$ |
| 11700 | $5.7692 \cdot 10^{-28}$ | $6.8076 \cdot 10^{-24}$ | $8.0330 \cdot 10^{-20}$ | $9.4789 \cdot 10^{-16}$ | $1.1186 \cdot 10^{-11}$ |
| 11800 | $3.9987 \cdot 10^{-28}$ | $4.7584 \cdot 10^{-24}$ | $5.6625 \cdot 10^{-20}$ | $6.7384 \cdot 10^{-16}$ | $8.0187 \cdot 10^{-12}$ |
| 11900 | $2.7776 \cdot 10^{-28}$ | $3.3331 \cdot 10^{-24}$ | $3.9997 \cdot 10^{-20}$ | $4.7996 \cdot 10^{-16}$ | $5.7596 \cdot 10^{-12}$ |
| 12000 | $1.9331 \cdot 10^{-28}$ | $2.3390 \cdot 10^{-24}$ | $2.8302 \cdot 10^{-20}$ | $3.4245 \cdot 10^{-16}$ | $4.1437 \cdot 10^{-12}$ |
| 12100 | $1.3478 \cdot 10^{-28}$ | $1.6443 \cdot 10^{-24}$ | $2.0060 \cdot 10^{-20}$ | $2.4473 \cdot 10^{-16}$ | $2.9857 \cdot 10^{-12}$ |
| 12200 | $9.3147 \cdot 10^{-29}$ | $1.1457 \cdot 10^{-24}$ | $1.4093 \cdot 10^{-20}$ | $1.7334 \cdot 10^{-16}$ | $2.1320 \cdot 10^{-12}$ |
| 12300 | $6.5069 \cdot 10^{-29}$ | $8.0686 \cdot 10^{-25}$ | $1.0005 \cdot 10^{-20}$ | $1.2407 \cdot 10^{-16}$ | $1.5384 \cdot 10^{-12}$ |
| 12400 | $4.5540 \cdot 10^{-29}$ | $5.6924 \cdot 10^{-25}$ | $7.1155 \cdot 10^{-21}$ | $8.8944 \cdot 10^{-17}$ | $1.1118 \cdot 10^{-12}$ |
| 12500 | $3.1924 \cdot 10^{-29}$ | $4.0224 \cdot 10^{-25}$ | $5.0682 \cdot 10^{-21}$ | $6.3860 \cdot 10^{-17}$ | $8.0463 \cdot 10^{-13}$ |
| 12600 | $2.2307 \cdot 10^{-29}$ | $2.8330 \cdot 10^{-25}$ | $3.5979 \cdot 10^{-21}$ | $4.5694 \cdot 10^{-17}$ | $5.8031 \cdot 10^{-13}$ |

Continued on next page

Table 11 – continued from previous page

| $b_j$ | $\mathcal{B}_{j,1}$     | $\mathcal{B}_{j,2}$     | $\mathcal{B}_{j,3}$     | $\mathcal{B}_{j,4}$     | $\mathcal{B}_{j,5}$     |
|-------|-------------------------|-------------------------|-------------------------|-------------------------|-------------------------|
| 12700 | $1.5600 \cdot 10^{-29}$ | $1.9967 \cdot 10^{-25}$ | $2.5558 \cdot 10^{-21}$ | $3.2714 \cdot 10^{-17}$ | $4.1874 \cdot 10^{-13}$ |
| 12800 | $1.0940 \cdot 10^{-29}$ | $1.4112 \cdot 10^{-25}$ | $1.8205 \cdot 10^{-21}$ | $2.3484 \cdot 10^{-17}$ | $3.0294 \cdot 10^{-13}$ |
| 12900 | $7.6900 \cdot 10^{-30}$ | $9.9970 \cdot 10^{-26}$ | $1.2996 \cdot 10^{-21}$ | $1.6895 \cdot 10^{-17}$ | $2.1964 \cdot 10^{-13}$ |
| 13000 | $5.5830 \cdot 10^{-30}$ | $7.5371 \cdot 10^{-26}$ | $1.0175 \cdot 10^{-21}$ | $1.3737 \cdot 10^{-17}$ | $1.8544 \cdot 10^{-13}$ |
| 13500 | $9.9578 \cdot 10^{-31}$ | $1.3743 \cdot 10^{-26}$ | $1.8966 \cdot 10^{-22}$ | $2.6174 \cdot 10^{-18}$ | $3.6123 \cdot 10^{-14}$ |
| 13800 | $3.5593 \cdot 10^{-31}$ | $4.9830 \cdot 10^{-27}$ | $6.9761 \cdot 10^{-23}$ | $9.7665 \cdot 10^{-19}$ | $1.3674 \cdot 10^{-14}$ |
| 14000 | $1.8399 \cdot 10^{-31}$ | $2.7598 \cdot 10^{-27}$ | $4.1396 \cdot 10^{-23}$ | $6.2094 \cdot 10^{-19}$ | $9.3141 \cdot 10^{-15}$ |
| 15000 | $6.5712 \cdot 10^{-33}$ | $1.0514 \cdot 10^{-28}$ | $1.6823 \cdot 10^{-24}$ | $2.6916 \cdot 10^{-20}$ | $4.3065 \cdot 10^{-16}$ |
| 16000 | $2.5739 \cdot 10^{-34}$ | $4.3756 \cdot 10^{-30}$ | $7.4384 \cdot 10^{-26}$ | $1.2646 \cdot 10^{-21}$ | $2.1497 \cdot 10^{-17}$ |
| 17000 | $1.1168 \cdot 10^{-35}$ | $2.0101 \cdot 10^{-31}$ | $3.6182 \cdot 10^{-27}$ | $6.5127 \cdot 10^{-23}$ | $1.1723 \cdot 10^{-18}$ |
| 18000 | $5.3739 \cdot 10^{-37}$ | $1.0211 \cdot 10^{-32}$ | $1.9400 \cdot 10^{-28}$ | $3.6860 \cdot 10^{-24}$ | $7.0033 \cdot 10^{-20}$ |
| 19000 | $2.7357 \cdot 10^{-38}$ | $5.4714 \cdot 10^{-34}$ | $1.0943 \cdot 10^{-29}$ | $2.1886 \cdot 10^{-25}$ | $4.3772 \cdot 10^{-21}$ |
| 20000 | $1.5041 \cdot 10^{-39}$ | $3.1585 \cdot 10^{-35}$ | $6.6329 \cdot 10^{-31}$ | $1.3929 \cdot 10^{-26}$ | $2.9251 \cdot 10^{-22}$ |
| 21000 | $9.0606 \cdot 10^{-41}$ | $1.9934 \cdot 10^{-36}$ | $4.3853 \cdot 10^{-32}$ | $9.6477 \cdot 10^{-28}$ | $2.1225 \cdot 10^{-23}$ |
| 22000 | $5.6101 \cdot 10^{-42}$ | $1.2904 \cdot 10^{-37}$ | $2.9678 \cdot 10^{-33}$ | $6.8258 \cdot 10^{-29}$ | $1.5700 \cdot 10^{-24}$ |
| 23000 | $3.7554 \cdot 10^{-43}$ | $9.0129 \cdot 10^{-39}$ | $2.1631 \cdot 10^{-34}$ | $5.1915 \cdot 10^{-30}$ | $1.2460 \cdot 10^{-25}$ |
| 24000 | $1.3804 \cdot 10^{-43}$ | $3.4508 \cdot 10^{-39}$ | $8.6269 \cdot 10^{-35}$ | $2.1568 \cdot 10^{-30}$ | $5.3919 \cdot 10^{-26}$ |
| 25000 | $1.3804 \cdot 10^{-43}$ | $3.4508 \cdot 10^{-39}$ | $8.6269 \cdot 10^{-35}$ | $2.1568 \cdot 10^{-30}$ | $5.3919 \cdot 10^{-26}$ |



5. TABLE 12: LOWER BOUND FOR FIRST VALUES OF  $x \in [e^{J_0}, 10^{19}]$

TABLE 12. Values of  $\mathcal{C}_{b,k}$  in  $\theta(x) > x - \frac{\mathcal{C}_{b,k}x}{(\log x)^k}$  calculated using the method described in Corollary 9.1, Section 3.4 of [1]. Each  $\mathcal{C}_{b,k}$  is valid for  $e^b \leq x \leq 10^{19} \simeq e^{43.749}$ .

| $b$                                                                                                       | $\mathcal{C}_{b,1}$    | $\mathcal{C}_{b,2}$    | $\mathcal{C}_{b,3}$    | $\mathcal{C}_{b,4}$    | $\mathcal{C}_{b,5}$    |
|-----------------------------------------------------------------------------------------------------------|------------------------|------------------------|------------------------|------------------------|------------------------|
| Calculated using $c = -0.8$ , $C = 0.81$ , each value valid up to $5 \cdot 10^{10} \simeq e^{24.635}$ .   |                        |                        |                        |                        |                        |
| 20                                                                                                        | $1.6844 \cdot 10^{-3}$ | $3.3688 \cdot 10^{-2}$ | $6.7375 \cdot 10^{-1}$ | $1.3475 \cdot 10^1$    | $2.6950 \cdot 10^2$    |
| 21                                                                                                        | $1.0684 \cdot 10^{-3}$ | $2.2435 \cdot 10^{-2}$ | $4.7114 \cdot 10^{-1}$ | $9.8939 \cdot 10^0$    | $2.0778 \cdot 10^2$    |
| 22                                                                                                        | $6.7654 \cdot 10^{-4}$ | $1.4884 \cdot 10^{-2}$ | $3.2745 \cdot 10^{-1}$ | $7.2038 \cdot 10^0$    | $1.5849 \cdot 10^2$    |
| 23                                                                                                        | $4.2780 \cdot 10^{-4}$ | $9.8392 \cdot 10^{-3}$ | $2.2631 \cdot 10^{-1}$ | $5.2050 \cdot 10^0$    | $1.1972 \cdot 10^2$    |
| 24                                                                                                        | $2.7012 \cdot 10^{-4}$ | $6.4829 \cdot 10^{-3}$ | $1.5559 \cdot 10^{-1}$ | $3.7341 \cdot 10^0$    | $8.9619 \cdot 10^1$    |
| Calculated using $c = -0.88$ , $C = 0.86$ , each value valid up to $32 \cdot 10^{12} \simeq e^{31.097}$ . |                        |                        |                        |                        |                        |
| $\log(5 \cdot 10^{10})$                                                                                   | $2.0156 \cdot 10^{-4}$ | $4.9654 \cdot 10^{-3}$ | $1.2233 \cdot 10^{-1}$ | $3.0135 \cdot 10^0$    | $7.4238 \cdot 10^1$    |
| 25                                                                                                        | $1.7033 \cdot 10^{-4}$ | $4.2583 \cdot 10^{-3}$ | $1.0646 \cdot 10^{-1}$ | $2.6614 \cdot 10^0$    | $6.6535 \cdot 10^1$    |
| 26                                                                                                        | $1.1022 \cdot 10^{-4}$ | $2.8656 \cdot 10^{-3}$ | $7.4505 \cdot 10^{-2}$ | $1.9372 \cdot 10^0$    | $5.0365 \cdot 10^1$    |
| 27                                                                                                        | $6.9327 \cdot 10^{-5}$ | $1.8719 \cdot 10^{-3}$ | $5.0540 \cdot 10^{-2}$ | $1.3646 \cdot 10^0$    | $3.6843 \cdot 10^1$    |
| 28                                                                                                        | $4.3558 \cdot 10^{-5}$ | $1.2197 \cdot 10^{-3}$ | $3.4150 \cdot 10^{-2}$ | $9.5618 \cdot 10^{-1}$ | $2.6773 \cdot 10^1$    |
| 29                                                                                                        | $2.7338 \cdot 10^{-5}$ | $7.9278 \cdot 10^{-4}$ | $2.2991 \cdot 10^{-2}$ | $6.6673 \cdot 10^{-1}$ | $1.9336 \cdot 10^1$    |
| 30                                                                                                        | $1.7140 \cdot 10^{-5}$ | $5.1418 \cdot 10^{-4}$ | $1.5426 \cdot 10^{-2}$ | $4.6276 \cdot 10^{-1}$ | $1.3883 \cdot 10^1$    |
| 31                                                                                                        | $1.0735 \cdot 10^{-5}$ | $3.3279 \cdot 10^{-4}$ | $1.0317 \cdot 10^{-2}$ | $3.1981 \cdot 10^{-1}$ | $9.9140 \cdot 10^0$    |
| Calculated using $-c = C = 0.94$ , each value valid up to $10^{19} \simeq e^{43.749}$ .                   |                        |                        |                        |                        |                        |
| $\log(3.2 \cdot 10^{13})$                                                                                 | $1.0260 \cdot 10^{-5}$ | $3.1904 \cdot 10^{-4}$ | $9.9209 \cdot 10^{-3}$ | $3.0851 \cdot 10^{-1}$ | $9.5936 \cdot 10^0$    |
| 32                                                                                                        | $6.7175 \cdot 10^{-6}$ | $2.1496 \cdot 10^{-4}$ | $6.8787 \cdot 10^{-3}$ | $2.2012 \cdot 10^{-1}$ | $7.0438 \cdot 10^0$    |
| 33                                                                                                        | $4.3800 \cdot 10^{-6}$ | $1.4454 \cdot 10^{-4}$ | $4.7699 \cdot 10^{-3}$ | $1.5741 \cdot 10^{-1}$ | $5.1944 \cdot 10^0$    |
| 34                                                                                                        | $2.7361 \cdot 10^{-6}$ | $9.3027 \cdot 10^{-5}$ | $3.1630 \cdot 10^{-3}$ | $1.0754 \cdot 10^{-1}$ | $3.6564 \cdot 10^0$    |
| 35                                                                                                        | $1.7078 \cdot 10^{-6}$ | $5.9773 \cdot 10^{-5}$ | $2.0921 \cdot 10^{-3}$ | $7.3222 \cdot 10^{-2}$ | $2.5628 \cdot 10^0$    |
| 36                                                                                                        | $1.0652 \cdot 10^{-6}$ | $3.8346 \cdot 10^{-5}$ | $1.3805 \cdot 10^{-3}$ | $4.9696 \cdot 10^{-2}$ | $1.7891 \cdot 10^0$    |
| 37                                                                                                        | $6.6385 \cdot 10^{-7}$ | $2.4563 \cdot 10^{-5}$ | $9.0881 \cdot 10^{-4}$ | $3.3626 \cdot 10^{-2}$ | $1.2442 \cdot 10^0$    |
| 38                                                                                                        | $4.1345 \cdot 10^{-7}$ | $1.5712 \cdot 10^{-5}$ | $5.9702 \cdot 10^{-4}$ | $2.2687 \cdot 10^{-2}$ | $8.6210 \cdot 10^{-1}$ |
| 39                                                                                                        | $2.5733 \cdot 10^{-7}$ | $1.0036 \cdot 10^{-5}$ | $3.9140 \cdot 10^{-4}$ | $1.5265 \cdot 10^{-2}$ | $5.9532 \cdot 10^{-1}$ |
| 40                                                                                                        | $1.6006 \cdot 10^{-7}$ | $6.4024 \cdot 10^{-6}$ | $2.5610 \cdot 10^{-4}$ | $1.0244 \cdot 10^{-2}$ | $4.0975 \cdot 10^{-1}$ |
| 41                                                                                                        | $9.9497 \cdot 10^{-8}$ | $4.0794 \cdot 10^{-6}$ | $1.6726 \cdot 10^{-4}$ | $6.8574 \cdot 10^{-3}$ | $2.8116 \cdot 10^{-1}$ |
| 42                                                                                                        | $6.1814 \cdot 10^{-8}$ | $2.5962 \cdot 10^{-6}$ | $1.0904 \cdot 10^{-4}$ | $4.5797 \cdot 10^{-3}$ | $1.9235 \cdot 10^{-1}$ |
| 43                                                                                                        | $3.8382 \cdot 10^{-8}$ | $1.6505 \cdot 10^{-6}$ | $7.0968 \cdot 10^{-5}$ | $3.0517 \cdot 10^{-3}$ | $1.3122 \cdot 10^{-1}$ |
| $19 \cdot \log 10$                                                                                        | $2.6851 \cdot 10^{-8}$ | $1.1748 \cdot 10^{-6}$ | $5.1390 \cdot 10^{-5}$ | $2.2484 \cdot 10^{-3}$ | $9.8359 \cdot 10^{-2}$ |

6. TABLE 13: LOWER BOUND FOR  $x \leq 10^{19}$  (NUMERICAL VERIFICATION)

TABLE 13. Values for  $\mathcal{D}_k(a, b)$  in  $\mathcal{D}_k(a, b) = \max_{n_0 \leq n \leq n_1} \left( \frac{(\log p_n)^k \cdot (p_n - \theta(p_{n-1}))}{p_n} \right)$  calculated using the method described in Lemma 10, Section 3.5 of [1]. We give values for selected ranges between 1 and  $7.0 \cdot 10^{11}$ .

| $a$                | $b$                | $\mathcal{D}_0(a, b)$   | $\mathcal{D}_1(a, b)$   | $\mathcal{D}_2(a, b)$   | $\mathcal{D}_3(a, b)$   | $\mathcal{D}_4(a, b)$ | $\mathcal{D}_5(a, b)$ |
|--------------------|--------------------|-------------------------|-------------------------|-------------------------|-------------------------|-----------------------|-----------------------|
| 1                  | $1 \cdot 10^5$     | $1.00000 \cdot 10^0$    | $1.23228 \cdot 10^0$    | $3.96481 \cdot 10^0$    | $2.08282 \cdot 10^1$    | $1.51224 \cdot 10^2$  | $1.30475 \cdot 10^3$  |
| $1 \cdot 10^5$     | $5 \cdot 10^5$     | $4.73131 \cdot 10^{-3}$ | $5.53160 \cdot 10^{-2}$ | $6.46725 \cdot 10^{-1}$ | $7.56118 \cdot 10^0$    | $8.93458 \cdot 10^1$  | $1.07895 \cdot 10^3$  |
| $5 \cdot 10^5$     | $1 \cdot 10^6$     | $1.99799 \cdot 10^{-3}$ | $2.67236 \cdot 10^{-2}$ | $3.57434 \cdot 10^{-1}$ | $4.78076 \cdot 10^0$    | $6.39437 \cdot 10^1$  | $8.55260 \cdot 10^2$  |
| $1 \cdot 10^6$     | $5 \cdot 10^6$     | $1.67162 \cdot 10^{-3}$ | $2.32393 \cdot 10^{-2}$ | $3.23081 \cdot 10^{-1}$ | $4.49158 \cdot 10^0$    | $6.24434 \cdot 10^1$  | $8.68209 \cdot 10^2$  |
| $5 \cdot 10^6$     | $1 \cdot 10^7$     | $6.56794 \cdot 10^{-4}$ | $1.02357 \cdot 10^{-2}$ | $1.59515 \cdot 10^{-1}$ | $2.48592 \cdot 10^0$    | $3.87413 \cdot 10^1$  | $6.03754 \cdot 10^2$  |
| $1 \cdot 10^7$     | $5 \cdot 10^7$     | $5.24943 \cdot 10^{-4}$ | $8.47248 \cdot 10^{-3}$ | $1.36744 \cdot 10^{-1}$ | $2.20703 \cdot 10^0$    | $3.56210 \cdot 10^1$  | $5.74917 \cdot 10^2$  |
| $5 \cdot 10^7$     | $1 \cdot 10^8$     | $2.16306 \cdot 10^{-4}$ | $3.85492 \cdot 10^{-3}$ | $6.87010 \cdot 10^{-2}$ | $1.22436 \cdot 10^0$    | $2.18201 \cdot 10^1$  | $3.88870 \cdot 10^2$  |
| $1 \cdot 10^8$     | $1 \cdot 10^9$     | $1.48989 \cdot 10^{-4}$ | $2.74568 \cdot 10^{-3}$ | $5.06111 \cdot 10^{-2}$ | $9.4259 \cdot 10^{-1}$  | $1.74450 \cdot 10^1$  | $1.74450 \cdot 10^1$  |
| $1 \cdot 10^9$     | $1 \cdot 10^{10}$  | $4.57993 \cdot 10^{-5}$ | $9.59129 \cdot 10^{-4}$ | $2.00861 \cdot 10^{-2}$ | $4.20644 \cdot 10^{-1}$ | $8.80913 \cdot 10^0$  | $1.84481 \cdot 10^2$  |
| $1 \cdot 10^{10}$  | $2 \cdot 10^{10}$  | $1.63137 \cdot 10^{-5}$ | $3.77870 \cdot 10^{-4}$ | $8.75253 \cdot 10^{-3}$ | $2.02733 \cdot 10^{-1}$ | $4.69587 \cdot 10^0$  | $1.08770 \cdot 10^2$  |
| 19 035 709 163     | $2 \cdot 10^{10}$  | $1.13110 \cdot 10^{-5}$ | $2.67726 \cdot 10^{-4}$ | $6.33697 \cdot 10^{-3}$ | $1.49993 \cdot 10^{-1}$ | $3.55028 \cdot 10^0$  | $8.40336 \cdot 10^1$  |
| $2 \cdot 10^{10}$  | $3 \cdot 10^{10}$  | $1.03687 \cdot 10^{-5}$ | $2.46002 \cdot 10^{-4}$ | $5.83648 \cdot 10^{-3}$ | $1.38472 \cdot 10^{-1}$ | $3.28531 \cdot 10^0$  | $7.79452 \cdot 10^1$  |
| $3 \cdot 10^{10}$  | $4 \cdot 10^{10}$  | $8.08543 \cdot 10^{-6}$ | $1.95082 \cdot 10^{-4}$ | $4.72265 \cdot 10^{-3}$ | $1.14540 \cdot 10^{-1}$ | $2.77796 \cdot 10^0$  | $6.73747 \cdot 10^1$  |
| $4 \cdot 10^{10}$  | $5 \cdot 10^{10}$  | $7.11201 \cdot 10^{-6}$ | $1.75016 \cdot 10^{-4}$ | $4.30688 \cdot 10^{-3}$ | $1.05986 \cdot 10^{-1}$ | $2.60815 \cdot 10^0$  | $6.41826 \cdot 10^1$  |
| $5 \cdot 10^{10}$  | $6 \cdot 10^{10}$  | $7.53086 \cdot 10^{-6}$ | $1.85559 \cdot 10^{-4}$ | $4.57216 \cdot 10^{-3}$ | $1.12657 \cdot 10^{-1}$ | $2.77586 \cdot 10^0$  | $6.83969 \cdot 10^1$  |
| $6 \cdot 10^{10}$  | $7 \cdot 10^{10}$  | $5.71466 \cdot 10^{-6}$ | $1.42491 \cdot 10^{-4}$ | $3.55293 \cdot 10^{-3}$ | $8.85900 \cdot 10^{-2}$ | $2.20893 \cdot 10^0$  | $5.50783 \cdot 10^1$  |
| $7 \cdot 10^{10}$  | $8 \cdot 10^{10}$  | $5.39050 \cdot 10^{-6}$ | $1.34922 \cdot 10^{-4}$ | $3.37702 \cdot 10^{-3}$ | $8.45253 \cdot 10^{-2}$ | $2.11563 \cdot 10^0$  | $5.29532 \cdot 10^1$  |
| $8 \cdot 10^{10}$  | $9 \cdot 10^{10}$  | $4.35507 \cdot 10^{-6}$ | $1.09446 \cdot 10^{-4}$ | $2.75045 \cdot 10^{-3}$ | $6.91859 \cdot 10^{-2}$ | $1.74250 \cdot 10^0$  | $4.38862 \cdot 10^1$  |
| $9 \cdot 10^{10}$  | $10 \cdot 10^{10}$ | $4.10662 \cdot 10^{-6}$ | $1.03589 \cdot 10^{-4}$ | $2.61301 \cdot 10^{-3}$ | $6.59129 \cdot 10^{-2}$ | $1.66264 \cdot 10^0$  | $4.19399 \cdot 10^1$  |
| $10 \cdot 10^{10}$ | $11 \cdot 10^{10}$ | $5.26105 \cdot 10^{-6}$ | $1.33752 \cdot 10^{-4}$ | $3.40037 \cdot 10^{-3}$ | $8.64475 \cdot 10^{-2}$ | $2.19775 \cdot 10^0$  | $5.58735 \cdot 10^1$  |
| $11 \cdot 10^{10}$ | $12 \cdot 10^{10}$ | $5.26640 \cdot 10^{-6}$ | $1.33915 \cdot 10^{-4}$ | $3.40521 \cdot 10^{-3}$ | $8.65882 \cdot 10^{-2}$ | $2.20178 \cdot 10^0$  | $5.59872 \cdot 10^1$  |
| $12 \cdot 10^{10}$ | $13 \cdot 10^{10}$ | $4.44681 \cdot 10^{-6}$ | $1.13461 \cdot 10^{-4}$ | $2.89497 \cdot 10^{-3}$ | $7.38655 \cdot 10^{-2}$ | $1.88469 \cdot 10^0$  | $4.80880 \cdot 10^1$  |
| $13 \cdot 10^{10}$ | $14 \cdot 10^{10}$ | $3.41846 \cdot 10^{-6}$ | $8.76906 \cdot 10^{-5}$ | $2.24945 \cdot 10^{-3}$ | $5.77030 \cdot 10^{-2}$ | $1.48020 \cdot 10^0$  | $3.79703 \cdot 10^1$  |
| $14 \cdot 10^{10}$ | $15 \cdot 10^{10}$ | $3.29978 \cdot 10^{-6}$ | $8.47568 \cdot 10^{-5}$ | $2.17703 \cdot 10^{-3}$ | $5.59181 \cdot 10^{-2}$ | $1.43629 \cdot 10^0$  | $3.68919 \cdot 10^1$  |
| $15 \cdot 10^{10}$ | $16 \cdot 10^{10}$ | $4.01405 \cdot 10^{-6}$ | $1.03396 \cdot 10^{-4}$ | $2.66335 \cdot 10^{-3}$ | $6.86042 \cdot 10^{-2}$ | $1.76715 \cdot 10^0$  | $4.55193 \cdot 10^1$  |
| $16 \cdot 10^{10}$ | $17 \cdot 10^{10}$ | $3.63233 \cdot 10^{-6}$ | $9.38449 \cdot 10^{-5}$ | $2.42458 \cdot 10^{-3}$ | $6.26413 \cdot 10^{-2}$ | $1.61840 \cdot 10^0$  | $4.18129 \cdot 10^1$  |
| $17 \cdot 10^{10}$ | $18 \cdot 10^{10}$ | $3.14570 \cdot 10^{-6}$ | $8.13474 \cdot 10^{-5}$ | $2.10363 \cdot 10^{-3}$ | $5.43995 \cdot 10^{-2}$ | $1.40676 \cdot 10^0$  | $3.63786 \cdot 10^1$  |
| $18 \cdot 10^{10}$ | $19 \cdot 10^{10}$ | $3.18303 \cdot 10^{-6}$ | $8.25980 \cdot 10^{-5}$ | $2.14337 \cdot 10^{-3}$ | $5.56193 \cdot 10^{-2}$ | $1.44329 \cdot 10^0$  | $3.74526 \cdot 10^1$  |
| $19 \cdot 10^{10}$ | $20 \cdot 10^{10}$ | $3.28073 \cdot 10^{-6}$ | $8.52255 \cdot 10^{-5}$ | $2.21396 \cdot 10^{-3}$ | $5.75133 \cdot 10^{-2}$ | $1.49406 \cdot 10^0$  | $3.88120 \cdot 10^1$  |
| $20 \cdot 10^{10}$ | $21 \cdot 10^{10}$ | $2.73340 \cdot 10^{-6}$ | $7.11770 \cdot 10^{-5}$ | $1.85343 \cdot 10^{-3}$ | $4.82627 \cdot 10^{-2}$ | $1.25675 \cdot 10^0$  | $3.27253 \cdot 10^1$  |
| $21 \cdot 10^{10}$ | $22 \cdot 10^{10}$ | $2.53668 \cdot 10^{-6}$ | $6.61874 \cdot 10^{-5}$ | $1.72697 \cdot 10^{-3}$ | $4.50604 \cdot 10^{-2}$ | $1.17572 \cdot 10^0$  | $3.06771 \cdot 10^1$  |

Continued on next page

Table 13 – continued from previous page

| $a$                | $b$                | $\mathcal{D}_0(a, b)$   | $\mathcal{D}_1(a, b)$   | $\mathcal{D}_2(a, b)$   | $\mathcal{D}_3(a, b)$   | $\mathcal{D}_4(a, b)$   | $\mathcal{D}_5(a, b)$ |
|--------------------|--------------------|-------------------------|-------------------------|-------------------------|-------------------------|-------------------------|-----------------------|
| $22 \cdot 10^{10}$ | $23 \cdot 10^{10}$ | $2.52342 \cdot 10^{-6}$ | $6.60155 \cdot 10^{-5}$ | $1.72704 \cdot 10^{-3}$ | $4.51814 \cdot 10^{-2}$ | $1.18200 \cdot 10^0$    | $3.09224 \cdot 10^1$  |
| $23 \cdot 10^{10}$ | $24 \cdot 10^{10}$ | $3.00664 \cdot 10^{-6}$ | $7.86826 \cdot 10^{-5}$ | $2.05910 \cdot 10^{-3}$ | $5.38859 \cdot 10^{-2}$ | $1.41018 \cdot 10^0$    | $3.69038 \cdot 10^1$  |
| $24 \cdot 10^{10}$ | $25 \cdot 10^{10}$ | $2.52843 \cdot 10^{-6}$ | $6.63579 \cdot 10^{-5}$ | $1.74154 \cdot 10^{-3}$ | $4.57060 \cdot 10^{-2}$ | $1.19954 \cdot 10^0$    | $3.14814 \cdot 10^1$  |
| $25 \cdot 10^{10}$ | $26 \cdot 10^{10}$ | $2.70299 \cdot 10^{-6}$ | $7.10356 \cdot 10^{-5}$ | $1.86684 \cdot 10^{-3}$ | $4.90612 \cdot 10^{-2}$ | $1.28934 \cdot 10^0$    | $3.38844 \cdot 10^1$  |
| $26 \cdot 10^{10}$ | $27 \cdot 10^{10}$ | $2.86910 \cdot 10^{-6}$ | $7.55027 \cdot 10^{-5}$ | $1.98691 \cdot 10^{-3}$ | $5.22873 \cdot 10^{-2}$ | $1.37598 \cdot 10^0$    | $3.62101 \cdot 10^1$  |
| $27 \cdot 10^{10}$ | $28 \cdot 10^{10}$ | $2.43132 \cdot 10^{-6}$ | $6.40002 \cdot 10^{-5}$ | $1.68469 \cdot 10^{-3}$ | $4.43466 \cdot 10^{-2}$ | $1.16735 \cdot 10^0$    | $3.07283 \cdot 10^1$  |
| $28 \cdot 10^{10}$ | $29 \cdot 10^{10}$ | $2.73706 \cdot 10^{-6}$ | $7.22351 \cdot 10^{-5}$ | $1.90640 \cdot 10^{-3}$ | $5.03127 \cdot 10^{-2}$ | $1.32783 \cdot 10^0$    | $3.50434 \cdot 10^1$  |
| $29 \cdot 10^{10}$ | $30 \cdot 10^{10}$ | $2.59106 \cdot 10^{-6}$ | $6.84089 \cdot 10^{-5}$ | $1.80613 \cdot 10^{-3}$ | $4.76853 \cdot 10^{-2}$ | $1.25898 \cdot 10^0$    | $3.32396 \cdot 10^1$  |
| $30 \cdot 10^{10}$ | $31 \cdot 10^{10}$ | $2.41963 \cdot 10^{-6}$ | $6.39936 \cdot 10^{-5}$ | $1.69249 \cdot 10^{-3}$ | $4.47624 \cdot 10^{-2}$ | $1.18386 \cdot 10^0$    | $3.13105 \cdot 10^1$  |
| $31 \cdot 10^{10}$ | $32 \cdot 10^{10}$ | $2.21245 \cdot 10^{-6}$ | $5.85673 \cdot 10^{-5}$ | $1.55038 \cdot 10^{-3}$ | $4.10412 \cdot 10^{-2}$ | $1.08643 \cdot 10^0$    | $2.87598 \cdot 10^1$  |
| $32 \cdot 10^{10}$ | $33 \cdot 10^{10}$ | $1.72269 \cdot 10^{-6}$ | $4.56367 \cdot 10^{-5}$ | $1.20899 \cdot 10^{-3}$ | $3.20280 \cdot 10^{-2}$ | $8.48474 \cdot 10^{-1}$ | $2.24774 \cdot 10^1$  |
| $33 \cdot 10^{10}$ | $34 \cdot 10^{10}$ | $1.46360 \cdot 10^{-6}$ | $3.88604 \cdot 10^{-5}$ | $1.03180 \cdot 10^{-3}$ | $2.73956 \cdot 10^{-2}$ | $7.27389 \cdot 10^{-1}$ | $1.93132 \cdot 10^1$  |
| $34 \cdot 10^{10}$ | $35 \cdot 10^{10}$ | $1.91975 \cdot 10^{-6}$ | $5.10043 \cdot 10^{-5}$ | $1.35510 \cdot 10^{-3}$ | $3.60025 \cdot 10^{-2}$ | $9.56524 \cdot 10^{-1}$ | $2.54132 \cdot 10^1$  |
| $35 \cdot 10^{10}$ | $36 \cdot 10^{10}$ | $1.91465 \cdot 10^{-6}$ | $5.09395 \cdot 10^{-5}$ | $1.35525 \cdot 10^{-3}$ | $3.60567 \cdot 10^{-2}$ | $9.59293 \cdot 10^{-1}$ | $2.55221 \cdot 10^1$  |
| $36 \cdot 10^{10}$ | $37 \cdot 10^{10}$ | $2.19313 \cdot 10^{-6}$ | $5.83927 \cdot 10^{-5}$ | $1.55472 \cdot 10^{-3}$ | $4.13951 \cdot 10^{-2}$ | $1.10216 \cdot 10^0$    | $2.93453 \cdot 10^1$  |
| $37 \cdot 10^{10}$ | $38 \cdot 10^{10}$ | $2.05932 \cdot 10^{-6}$ | $5.48858 \cdot 10^{-5}$ | $1.46284 \cdot 10^{-3}$ | $3.89883 \cdot 10^{-2}$ | $1.03913 \cdot 10^0$    | $2.76954 \cdot 10^1$  |
| $38 \cdot 10^{10}$ | $39 \cdot 10^{10}$ | $2.29636 \cdot 10^{-6}$ | $6.12815 \cdot 10^{-5}$ | $1.63538 \cdot 10^{-3}$ | $4.36424 \cdot 10^{-2}$ | $1.16466 \cdot 10^0$    | $3.10805 \cdot 10^1$  |
| $39 \cdot 10^{10}$ | $40 \cdot 10^{10}$ | $2.32437 \cdot 10^{-6}$ | $6.20941 \cdot 10^{-5}$ | $1.65880 \cdot 10^{-3}$ | $4.43139 \cdot 10^{-2}$ | $1.18382 \cdot 10^0$    | $3.16250 \cdot 10^1$  |
| $40 \cdot 10^{10}$ | $41 \cdot 10^{10}$ | $2.62662 \cdot 10^{-6}$ | $7.01926 \cdot 10^{-5}$ | $1.87579 \cdot 10^{-3}$ | $5.01279 \cdot 10^{-2}$ | $1.33959 \cdot 10^0$    | $3.57987 \cdot 10^1$  |
| $41 \cdot 10^{10}$ | $42 \cdot 10^{10}$ | $2.18274 \cdot 10^{-6}$ | $5.83701 \cdot 10^{-5}$ | $1.56091 \cdot 10^{-3}$ | $4.17413 \cdot 10^{-2}$ | $1.11623 \cdot 10^0$    | $2.98498 \cdot 10^1$  |
| $42 \cdot 10^{10}$ | $43 \cdot 10^{10}$ | $2.11475 \cdot 10^{-6}$ | $5.66141 \cdot 10^{-5}$ | $1.51562 \cdot 10^{-3}$ | $4.05749 \cdot 10^{-2}$ | $1.08624 \cdot 10^0$    | $2.90798 \cdot 10^1$  |
| $43 \cdot 10^{10}$ | $44 \cdot 10^{10}$ | $1.83951 \cdot 10^{-6}$ | $4.92751 \cdot 10^{-5}$ | $1.31993 \cdot 10^{-3}$ | $3.53572 \cdot 10^{-2}$ | $9.47114 \cdot 10^{-1}$ | $2.53704 \cdot 10^1$  |
| $44 \cdot 10^{10}$ | $45 \cdot 10^{10}$ | $1.66382 \cdot 10^{-6}$ | $4.46343 \cdot 10^{-5}$ | $1.19737 \cdot 10^{-3}$ | $3.21211 \cdot 10^{-2}$ | $8.61691 \cdot 10^{-1}$ | $2.31160 \cdot 10^1$  |
| $45 \cdot 10^{10}$ | $46 \cdot 10^{10}$ | $1.64139 \cdot 10^{-6}$ | $4.40693 \cdot 10^{-5}$ | $1.18320 \cdot 10^{-3}$ | $3.17676 \cdot 10^{-2}$ | $8.52919 \cdot 10^{-1}$ | $2.28998 \cdot 10^1$  |
| $46 \cdot 10^{10}$ | $47 \cdot 10^{10}$ | $1.71266 \cdot 10^{-6}$ | $4.60159 \cdot 10^{-5}$ | $1.23636 \cdot 10^{-3}$ | $3.32186 \cdot 10^{-2}$ | $8.92519 \cdot 10^{-1}$ | $2.39803 \cdot 10^1$  |
| $47 \cdot 10^{10}$ | $48 \cdot 10^{10}$ | $1.87687 \cdot 10^{-6}$ | $5.04822 \cdot 10^{-5}$ | $1.35782 \cdot 10^{-3}$ | $3.65213 \cdot 10^{-2}$ | $9.82313 \cdot 10^{-1}$ | $2.64213 \cdot 10^1$  |
| $48 \cdot 10^{10}$ | $49 \cdot 10^{10}$ | $1.87852 \cdot 10^{-6}$ | $5.05266 \cdot 10^{-5}$ | $1.35902 \cdot 10^{-3}$ | $3.65535 \cdot 10^{-2}$ | $9.83182 \cdot 10^{-1}$ | $2.64447 \cdot 10^1$  |
| $49 \cdot 10^{10}$ | $50 \cdot 10^{10}$ | $1.88896 \cdot 10^{-6}$ | $5.08825 \cdot 10^{-5}$ | $1.37061 \cdot 10^{-3}$ | $3.69198 \cdot 10^{-2}$ | $9.94501 \cdot 10^{-1}$ | $2.67886 \cdot 10^1$  |
| $50 \cdot 10^{10}$ | $51 \cdot 10^{10}$ | $1.89356 \cdot 10^{-6}$ | $5.10206 \cdot 10^{-5}$ | $1.37472 \cdot 10^{-3}$ | $3.70409 \cdot 10^{-2}$ | $9.98044 \cdot 10^{-1}$ | $2.68917 \cdot 10^1$  |
| $51 \cdot 10^{10}$ | $52 \cdot 10^{10}$ | $1.80664 \cdot 10^{-6}$ | $4.87131 \cdot 10^{-5}$ | $1.31347 \cdot 10^{-3}$ | $3.54157 \cdot 10^{-2}$ | $9.54927 \cdot 10^{-1}$ | $2.57481 \cdot 10^1$  |
| $52 \cdot 10^{10}$ | $53 \cdot 10^{10}$ | $1.74704 \cdot 10^{-6}$ | $4.71470 \cdot 10^{-5}$ | $1.27235 \cdot 10^{-3}$ | $3.43367 \cdot 10^{-2}$ | $9.26639 \cdot 10^{-1}$ | $2.50071 \cdot 10^1$  |
| $53 \cdot 10^{10}$ | $54 \cdot 10^{10}$ | $1.39274 \cdot 10^{-6}$ | $3.75997 \cdot 10^{-5}$ | $1.01507 \cdot 10^{-3}$ | $2.74038 \cdot 10^{-2}$ | $7.39818 \cdot 10^{-1}$ | $1.99728 \cdot 10^1$  |
| $54 \cdot 10^{10}$ | $55 \cdot 10^{10}$ | $1.25296 \cdot 10^{-6}$ | $3.38714 \cdot 10^{-5}$ | $9.15650 \cdot 10^{-4}$ | $2.47529 \cdot 10^{-2}$ | $6.69150 \cdot 10^{-1}$ | $1.80892 \cdot 10^1$  |
| $55 \cdot 10^{10}$ | $56 \cdot 10^{10}$ | $1.30633 \cdot 10^{-6}$ | $3.53272 \cdot 10^{-5}$ | $9.55357 \cdot 10^{-4}$ | $2.58358 \cdot 10^{-2}$ | $6.98680 \cdot 10^{-1}$ | $1.88944 \cdot 10^1$  |
| $56 \cdot 10^{10}$ | $57 \cdot 10^{10}$ | $1.22171 \cdot 10^{-6}$ | $3.30680 \cdot 10^{-5}$ | $8.95046 \cdot 10^{-4}$ | $2.42261 \cdot 10^{-2}$ | $6.55724 \cdot 10^{-1}$ | $1.77484 \cdot 10^1$  |
| $57 \cdot 10^{10}$ | $58 \cdot 10^{10}$ | $1.40190 \cdot 10^{-6}$ | $3.79535 \cdot 10^{-5}$ | $1.02751 \cdot 10^{-3}$ | $2.78179 \cdot 10^{-2}$ | $7.53112 \cdot 10^{-1}$ | $2.03890 \cdot 10^1$  |
| $58 \cdot 10^{10}$ | $59 \cdot 10^{10}$ | $1.69730 \cdot 10^{-6}$ | $4.59964 \cdot 10^{-5}$ | $1.24649 \cdot 10^{-3}$ | $3.37795 \cdot 10^{-2}$ | $9.15416 \cdot 10^{-1}$ | $2.48075 \cdot 10^1$  |

Continued on next page

Table 13 – continued from previous page

| $a$                | $b$                | $\mathcal{D}_0(a, b)$   | $\mathcal{D}_1(a, b)$   | $\mathcal{D}_2(a, b)$   | $\mathcal{D}_3(a, b)$   | $\mathcal{D}_4(a, b)$   | $\mathcal{D}_5(a, b)$ |
|--------------------|--------------------|-------------------------|-------------------------|-------------------------|-------------------------|-------------------------|-----------------------|
| $59 \cdot 10^{10}$ | $60 \cdot 10^{10}$ | $1.62157 \cdot 10^{-6}$ | $4.39642 \cdot 10^{-5}$ | $1.19197 \cdot 10^{-3}$ | $3.23168 \cdot 10^{-2}$ | $8.76180 \cdot 10^{-1}$ | $2.37551 \cdot 10^1$  |
| $60 \cdot 10^{10}$ | $61 \cdot 10^{10}$ | $1.52488 \cdot 10^{-6}$ | $4.13767 \cdot 10^{-5}$ | $1.12274 \cdot 10^{-3}$ | $3.04648 \cdot 10^{-2}$ | $8.26646 \cdot 10^{-1}$ | $2.24306 \cdot 10^1$  |
| $61 \cdot 10^{10}$ | $62 \cdot 10^{10}$ | $1.60364 \cdot 10^{-6}$ | $4.35194 \cdot 10^{-5}$ | $1.18102 \cdot 10^{-3}$ | $3.20503 \cdot 10^{-2}$ | $8.69773 \cdot 10^{-1}$ | $2.36037 \cdot 10^1$  |
| $62 \cdot 10^{10}$ | $63 \cdot 10^{10}$ | $1.71497 \cdot 10^{-6}$ | $4.65765 \cdot 10^{-5}$ | $1.26496 \cdot 10^{-3}$ | $3.43547 \cdot 10^{-2}$ | $9.33031 \cdot 10^{-1}$ | $2.53400 \cdot 10^1$  |
| $63 \cdot 10^{10}$ | $64 \cdot 10^{10}$ | $1.69670 \cdot 10^{-6}$ | $4.61014 \cdot 10^{-5}$ | $1.25263 \cdot 10^{-3}$ | $3.40354 \cdot 10^{-2}$ | $9.24780 \cdot 10^{-1}$ | $2.51274 \cdot 10^1$  |
| $64 \cdot 10^{10}$ | $65 \cdot 10^{10}$ | $1.59469 \cdot 10^{-6}$ | $4.33521 \cdot 10^{-5}$ | $1.17854 \cdot 10^{-3}$ | $3.20389 \cdot 10^{-2}$ | $8.70987 \cdot 10^{-1}$ | $2.36780 \cdot 10^1$  |
| $65 \cdot 10^{10}$ | $66 \cdot 10^{10}$ | $1.65110 \cdot 10^{-6}$ | $4.49346 \cdot 10^{-5}$ | $1.22289 \cdot 10^{-3}$ | $3.32810 \cdot 10^{-2}$ | $9.05741 \cdot 10^{-1}$ | $2.46497 \cdot 10^1$  |
| $66 \cdot 10^{10}$ | $67 \cdot 10^{10}$ | $1.66910 \cdot 10^{-6}$ | $4.54282 \cdot 10^{-5}$ | $1.23643 \cdot 10^{-3}$ | $3.36521 \cdot 10^{-2}$ | $9.15915 \cdot 10^{-1}$ | $2.49286 \cdot 10^1$  |
| $67 \cdot 10^{10}$ | $68 \cdot 10^{10}$ | $1.57358 \cdot 10^{-6}$ | $4.28513 \cdot 10^{-5}$ | $1.16692 \cdot 10^{-3}$ | $3.17773 \cdot 10^{-2}$ | $8.65354 \cdot 10^{-1}$ | $2.35652 \cdot 10^1$  |
| $68 \cdot 10^{10}$ | $69 \cdot 10^{10}$ | $1.75478 \cdot 10^{-6}$ | $4.78305 \cdot 10^{-5}$ | $1.30373 \cdot 10^{-3}$ | $3.55359 \cdot 10^{-2}$ | $9.68610 \cdot 10^{-1}$ | $2.64016 \cdot 10^1$  |
| $69 \cdot 10^{10}$ | $70 \cdot 10^{10}$ | $1.57476 \cdot 10^{-6}$ | $4.29284 \cdot 10^{-5}$ | $1.17024 \cdot 10^{-3}$ | $3.19011 \cdot 10^{-2}$ | $8.69631 \cdot 10^{-1}$ | $2.37064 \cdot 10^1$  |

7. TABLE 14: VALUES FOR THEOREM 2 FOR  $k = 0$ .

TABLE 14. Values of  $m_0$  in  $\theta(x) \geq x(1 - m_0)$  and values of  $M_0$  in  $\theta(x) \leq x(1 + M_0)$  from Theorem 1 of [1], using the methods shown in Section 3.6 of [1]. Each value is valid for  $x \geq \log X_0 = \log X_1$ .

| $\log X_0 = \log X_1$ | $M_0$                       | $m_0$                       |
|-----------------------|-----------------------------|-----------------------------|
| 20                    | $4.26760000 \cdot 10^{-5}$  | $9.16390000 \cdot 10^{-5}$  |
| 21                    | $2.58843000 \cdot 10^{-5}$  | $5.54070000 \cdot 10^{-5}$  |
| 22                    | $1.56996000 \cdot 10^{-5}$  | $3.35170000 \cdot 10^{-5}$  |
| 23                    | $9.52229000 \cdot 10^{-6}$  | $2.02850000 \cdot 10^{-5}$  |
| 24                    | $5.77556000 \cdot 10^{-6}$  | $1.22810000 \cdot 10^{-5}$  |
| 25                    | $3.50306000 \cdot 10^{-6}$  | $7.43660000 \cdot 10^{-6}$  |
| 26                    | $2.12471000 \cdot 10^{-6}$  | $4.50460000 \cdot 10^{-6}$  |
| 27                    | $1.28871000 \cdot 10^{-6}$  | $2.72920000 \cdot 10^{-6}$  |
| 28                    | $7.81637000 \cdot 10^{-7}$  | $1.65380000 \cdot 10^{-6}$  |
| 29                    | $4.74087000 \cdot 10^{-7}$  | $1.00230000 \cdot 10^{-6}$  |
| 30                    | $2.87549000 \cdot 10^{-7}$  | $6.07510000 \cdot 10^{-7}$  |
| 31                    | $1.74407000 \cdot 10^{-7}$  | $3.68270000 \cdot 10^{-7}$  |
| 32                    | $1.05784000 \cdot 10^{-7}$  | $2.23270000 \cdot 10^{-7}$  |
| 33                    | $6.41607000 \cdot 10^{-8}$  | $1.35370000 \cdot 10^{-7}$  |
| 34                    | $3.89155000 \cdot 10^{-8}$  | $8.20730000 \cdot 10^{-8}$  |
| 35                    | $2.36034000 \cdot 10^{-8}$  | $4.97660000 \cdot 10^{-8}$  |
| 36                    | $1.93378000 \cdot 10^{-8}$  | $3.51990000 \cdot 10^{-8}$  |
| 37                    | $1.93378000 \cdot 10^{-8}$  | $2.89550000 \cdot 10^{-8}$  |
| 38                    | $1.93378000 \cdot 10^{-8}$  | $2.51690000 \cdot 10^{-8}$  |
| 39                    | $1.93378000 \cdot 10^{-8}$  | $2.28740000 \cdot 10^{-8}$  |
| 40                    | $1.93378000 \cdot 10^{-8}$  | $2.14820000 \cdot 10^{-8}$  |
| 41                    | $1.93378000 \cdot 10^{-8}$  | $2.06380000 \cdot 10^{-8}$  |
| 42                    | $1.93378000 \cdot 10^{-8}$  | $2.01270000 \cdot 10^{-8}$  |
| 43                    | $1.93378000 \cdot 10^{-8}$  | $1.98160000 \cdot 10^{-8}$  |
| 19 log 10             | $1.93378000 \cdot 10^{-8}$  | $1.96670000 \cdot 10^{-8}$  |
| 44                    | $1.72001000 \cdot 10^{-8}$  | $1.74910000 \cdot 10^{-8}$  |
| 45                    | $1.09073000 \cdot 10^{-8}$  | $1.10840000 \cdot 10^{-8}$  |
| 46                    | $6.94507000 \cdot 10^{-9}$  | $7.05180000 \cdot 10^{-9}$  |
| 47                    | $4.40123000 \cdot 10^{-9}$  | $4.46600000 \cdot 10^{-9}$  |
| 48                    | $2.79143000 \cdot 10^{-9}$  | $2.83070000 \cdot 10^{-9}$  |
| 49                    | $1.76889000 \cdot 10^{-9}$  | $1.79270000 \cdot 10^{-9}$  |
| 50                    | $1.11990000 \cdot 10^{-9}$  | $1.13440000 \cdot 10^{-9}$  |
| 51                    | $7.09243000 \cdot 10^{-10}$ | $7.18000000 \cdot 10^{-10}$ |
| 52                    | $4.47806000 \cdot 10^{-10}$ | $4.53120000 \cdot 10^{-10}$ |
| 53                    | $2.82796000 \cdot 10^{-10}$ | $2.86020000 \cdot 10^{-10}$ |
| 54                    | $1.78455000 \cdot 10^{-10}$ | $1.80410000 \cdot 10^{-10}$ |
| 55                    | $1.12553000 \cdot 10^{-10}$ | $1.13740000 \cdot 10^{-10}$ |
| 56                    | $7.09282000 \cdot 10^{-11}$ | $7.16470000 \cdot 10^{-11}$ |
| 57                    | $4.46546000 \cdot 10^{-11}$ | $4.50910000 \cdot 10^{-11}$ |
| 58                    | $2.83279000 \cdot 10^{-11}$ | $2.85930000 \cdot 10^{-11}$ |
| 59                    | $1.84401000 \cdot 10^{-11}$ | $1.86010000 \cdot 10^{-11}$ |
| 60                    | $1.22147000 \cdot 10^{-11}$ | $1.23120000 \cdot 10^{-11}$ |
| 65                    | $3.57125000 \cdot 10^{-12}$ | $3.57930000 \cdot 10^{-12}$ |
| 70                    | $2.79233000 \cdot 10^{-12}$ | $2.79300000 \cdot 10^{-12}$ |
| 75                    | $2.70358000 \cdot 10^{-12}$ | $2.70370000 \cdot 10^{-12}$ |
| 80                    | $2.61079000 \cdot 10^{-12}$ | $2.61080000 \cdot 10^{-12}$ |
| 85                    | $2.56924000 \cdot 10^{-12}$ | $2.56930000 \cdot 10^{-12}$ |

Continued on next page

Table 14 – continued from previous page

| $\log X_0 = \log X_1$ | $M_0$                       | $m_0$                       |
|-----------------------|-----------------------------|-----------------------------|
| 90                    | $2.52129000 \cdot 10^{-12}$ | $2.52130000 \cdot 10^{-12}$ |
| 95                    | $2.49192000 \cdot 10^{-12}$ | $2.49200000 \cdot 10^{-12}$ |
| 100                   | $2.45299000 \cdot 10^{-12}$ | $2.45300000 \cdot 10^{-12}$ |
| 200                   | $2.18154000 \cdot 10^{-12}$ | $2.18160000 \cdot 10^{-12}$ |
| 300                   | $2.09022000 \cdot 10^{-12}$ | $2.09030000 \cdot 10^{-12}$ |
| 400                   | $2.03981000 \cdot 10^{-12}$ | $2.03990000 \cdot 10^{-12}$ |
| 500                   | $1.99986000 \cdot 10^{-12}$ | $1.99990000 \cdot 10^{-12}$ |
| 600                   | $1.98894000 \cdot 10^{-12}$ | $1.98900000 \cdot 10^{-12}$ |
| 700                   | $1.97643000 \cdot 10^{-12}$ | $1.97650000 \cdot 10^{-12}$ |
| 800                   | $1.96710000 \cdot 10^{-12}$ | $1.96710000 \cdot 10^{-12}$ |
| 900                   | $1.95987000 \cdot 10^{-12}$ | $1.95990000 \cdot 10^{-12}$ |
| 1000                  | $1.94751000 \cdot 10^{-12}$ | $1.94760000 \cdot 10^{-12}$ |
| 1500                  | $1.93677000 \cdot 10^{-12}$ | $1.93680000 \cdot 10^{-12}$ |
| 1600                  | $1.92922000 \cdot 10^{-12}$ | $1.92930000 \cdot 10^{-12}$ |
| 1700                  | $1.92733000 \cdot 10^{-12}$ | $1.92740000 \cdot 10^{-12}$ |
| 1725                  | $1.92689000 \cdot 10^{-12}$ | $1.92690000 \cdot 10^{-12}$ |
| 1750                  | $1.92646000 \cdot 10^{-12}$ | $1.92650000 \cdot 10^{-12}$ |
| 1775                  | $1.92604000 \cdot 10^{-12}$ | $1.92610000 \cdot 10^{-12}$ |
| 1800                  | $1.92564000 \cdot 10^{-12}$ | $1.92570000 \cdot 10^{-12}$ |
| 1825                  | $1.92525000 \cdot 10^{-12}$ | $1.92530000 \cdot 10^{-12}$ |
| 1850                  | $1.92487000 \cdot 10^{-12}$ | $1.92490000 \cdot 10^{-12}$ |
| 1875                  | $1.92450000 \cdot 10^{-12}$ | $1.92450000 \cdot 10^{-12}$ |
| 1900                  | $1.92414000 \cdot 10^{-12}$ | $1.92420000 \cdot 10^{-12}$ |
| 1925                  | $1.92379000 \cdot 10^{-12}$ | $1.92380000 \cdot 10^{-12}$ |
| 1950                  | $1.92344000 \cdot 10^{-12}$ | $1.92350000 \cdot 10^{-12}$ |
| 1975                  | $1.92311000 \cdot 10^{-12}$ | $1.92320000 \cdot 10^{-12}$ |
| 2000                  | $1.92279000 \cdot 10^{-12}$ | $1.92280000 \cdot 10^{-12}$ |
| 2025                  | $1.92247000 \cdot 10^{-12}$ | $1.92250000 \cdot 10^{-12}$ |
| 2050                  | $1.92216000 \cdot 10^{-12}$ | $1.92220000 \cdot 10^{-12}$ |
| 2075                  | $1.92186000 \cdot 10^{-12}$ | $1.92190000 \cdot 10^{-12}$ |
| 2100                  | $1.92156000 \cdot 10^{-12}$ | $1.92160000 \cdot 10^{-12}$ |
| 2125                  | $1.92128000 \cdot 10^{-12}$ | $1.92130000 \cdot 10^{-12}$ |
| 2150                  | $1.92100000 \cdot 10^{-12}$ | $1.92100000 \cdot 10^{-12}$ |
| 2175                  | $1.92072000 \cdot 10^{-12}$ | $1.92080000 \cdot 10^{-12}$ |
| 2200                  | $1.92046000 \cdot 10^{-12}$ | $1.92050000 \cdot 10^{-12}$ |
| 2225                  | $1.92019000 \cdot 10^{-12}$ | $1.92020000 \cdot 10^{-12}$ |
| 2250                  | $1.91994000 \cdot 10^{-12}$ | $1.92000000 \cdot 10^{-12}$ |
| 2275                  | $1.91969000 \cdot 10^{-12}$ | $1.91970000 \cdot 10^{-12}$ |
| 2300                  | $1.91944000 \cdot 10^{-12}$ | $1.91950000 \cdot 10^{-12}$ |
| 2325                  | $1.87499000 \cdot 10^{-12}$ | $1.87500000 \cdot 10^{-12}$ |
| 2350                  | $1.77873000 \cdot 10^{-12}$ | $1.77880000 \cdot 10^{-12}$ |
| 2375                  | $1.68743000 \cdot 10^{-12}$ | $1.68750000 \cdot 10^{-12}$ |
| 2400                  | $1.60083000 \cdot 10^{-12}$ | $1.60090000 \cdot 10^{-12}$ |
| 2425                  | $1.42172300 \cdot 10^{-12}$ | $1.42180000 \cdot 10^{-12}$ |
| 2450                  | $1.22132480 \cdot 10^{-12}$ | $1.22140000 \cdot 10^{-12}$ |
| 2475                  | $1.05112910 \cdot 10^{-12}$ | $1.05120000 \cdot 10^{-12}$ |
| 2500                  | $9.06303550 \cdot 10^{-13}$ | $9.06310000 \cdot 10^{-13}$ |
| 2525                  | $7.79324680 \cdot 10^{-13}$ | $7.79330000 \cdot 10^{-13}$ |
| 2550                  | $6.70678560 \cdot 10^{-13}$ | $6.70680000 \cdot 10^{-13}$ |
| 2575                  | $5.76611200 \cdot 10^{-13}$ | $5.76620000 \cdot 10^{-13}$ |
| 2600                  | $4.96086610 \cdot 10^{-13}$ | $4.96090000 \cdot 10^{-13}$ |
| 2625                  | $4.26925890 \cdot 10^{-13}$ | $4.26930000 \cdot 10^{-13}$ |
| 2650                  | $3.67459760 \cdot 10^{-13}$ | $3.67460000 \cdot 10^{-13}$ |
| 2675                  | $3.16411610 \cdot 10^{-13}$ | $3.16420000 \cdot 10^{-13}$ |
| 2700                  | $2.72417160 \cdot 10^{-13}$ | $2.72420000 \cdot 10^{-13}$ |

Continued on next page

Table 14 – continued from previous page

| $\log X_0 = \log X_1$ | $M_0$                       | $m_0$                       |
|-----------------------|-----------------------------|-----------------------------|
| 2725                  | $2.34537640 \cdot 10^{-13}$ | $2.34540000 \cdot 10^{-13}$ |
| 2750                  | $2.02057750 \cdot 10^{-13}$ | $2.02060000 \cdot 10^{-13}$ |
| 2775                  | $1.74034120 \cdot 10^{-13}$ | $1.74040000 \cdot 10^{-13}$ |
| 2800                  | $1.50046680 \cdot 10^{-13}$ | $1.50050000 \cdot 10^{-13}$ |
| 2825                  | $1.29513280 \cdot 10^{-13}$ | $1.29520000 \cdot 10^{-13}$ |
| 2850                  | $1.11886580 \cdot 10^{-13}$ | $1.11890000 \cdot 10^{-13}$ |
| 2875                  | $9.63879480 \cdot 10^{-14}$ | $9.63880000 \cdot 10^{-14}$ |
| 2900                  | $8.31661760 \cdot 10^{-14}$ | $8.31670000 \cdot 10^{-14}$ |
| 2925                  | $7.16612100 \cdot 10^{-14}$ | $7.16620000 \cdot 10^{-14}$ |
| 2950                  | $6.18165850 \cdot 10^{-14}$ | $6.18170000 \cdot 10^{-14}$ |
| 2975                  | $5.33821180 \cdot 10^{-14}$ | $5.33830000 \cdot 10^{-14}$ |
| 3000                  | $4.59971650 \cdot 10^{-14}$ | $4.59980000 \cdot 10^{-14}$ |
| 3025                  | $3.97197520 \cdot 10^{-14}$ | $3.97200000 \cdot 10^{-14}$ |
| 3050                  | $3.42456560 \cdot 10^{-14}$ | $3.42460000 \cdot 10^{-14}$ |
| 3075                  | $2.95754100 \cdot 10^{-14}$ | $2.95760000 \cdot 10^{-14}$ |
| 3100                  | $2.55336000 \cdot 10^{-14}$ | $2.55340000 \cdot 10^{-14}$ |
| 3125                  | $2.20304500 \cdot 10^{-14}$ | $2.20310000 \cdot 10^{-14}$ |
| 3150                  | $1.90265910 \cdot 10^{-14}$ | $1.90270000 \cdot 10^{-14}$ |
| 3175                  | $1.64287280 \cdot 10^{-14}$ | $1.64290000 \cdot 10^{-14}$ |
| 3200                  | $1.41958670 \cdot 10^{-14}$ | $1.41960000 \cdot 10^{-14}$ |
| 3225                  | $1.22772600 \cdot 10^{-14}$ | $1.22780000 \cdot 10^{-14}$ |
| 3250                  | $1.06260230 \cdot 10^{-14}$ | $1.06270000 \cdot 10^{-14}$ |
| 3275                  | $9.19135030 \cdot 10^{-15}$ | $9.19140000 \cdot 10^{-15}$ |
| 3300                  | $7.94342550 \cdot 10^{-15}$ | $7.94350000 \cdot 10^{-15}$ |
| 3325                  | $6.87011930 \cdot 10^{-15}$ | $6.87020000 \cdot 10^{-15}$ |
| 3350                  | $5.93855920 \cdot 10^{-15}$ | $5.93860000 \cdot 10^{-15}$ |
| 3375                  | $5.13318710 \cdot 10^{-15}$ | $5.13320000 \cdot 10^{-15}$ |
| 3400                  | $4.44128700 \cdot 10^{-15}$ | $4.44130000 \cdot 10^{-15}$ |
| 3425                  | $3.84526310 \cdot 10^{-15}$ | $3.84530000 \cdot 10^{-15}$ |
| 3450                  | $3.32496110 \cdot 10^{-15}$ | $3.32500000 \cdot 10^{-15}$ |
| 3475                  | $2.87396010 \cdot 10^{-15}$ | $2.87400000 \cdot 10^{-15}$ |
| 3500                  | $2.48640360 \cdot 10^{-15}$ | $2.48650000 \cdot 10^{-15}$ |
| 3525                  | $2.15219300 \cdot 10^{-15}$ | $2.15220000 \cdot 10^{-15}$ |
| 3550                  | $1.86315230 \cdot 10^{-15}$ | $1.86320000 \cdot 10^{-15}$ |
| 3575                  | $1.61226920 \cdot 10^{-15}$ | $1.61230000 \cdot 10^{-15}$ |
| 3600                  | $1.39645160 \cdot 10^{-15}$ | $1.39650000 \cdot 10^{-15}$ |
| 3625                  | $1.21000520 \cdot 10^{-15}$ | $1.21010000 \cdot 10^{-15}$ |
| 3650                  | $1.04693670 \cdot 10^{-15}$ | $1.04700000 \cdot 10^{-15}$ |
| 3675                  | $9.07031130 \cdot 10^{-16}$ | $9.07040000 \cdot 10^{-16}$ |
| 3700                  | $7.86455750 \cdot 10^{-16}$ | $7.86460000 \cdot 10^{-16}$ |
| 3725                  | $6.82123910 \cdot 10^{-16}$ | $6.82130000 \cdot 10^{-16}$ |
| 3750                  | $5.91953430 \cdot 10^{-16}$ | $5.91960000 \cdot 10^{-16}$ |
| 3775                  | $5.13510070 \cdot 10^{-16}$ | $5.13520000 \cdot 10^{-16}$ |
| 3800                  | $4.44952080 \cdot 10^{-16}$ | $4.44960000 \cdot 10^{-16}$ |
| 3825                  | $3.85823120 \cdot 10^{-16}$ | $3.85830000 \cdot 10^{-16}$ |
| 3850                  | $3.34763150 \cdot 10^{-16}$ | $3.34770000 \cdot 10^{-16}$ |
| 3875                  | $2.90095130 \cdot 10^{-16}$ | $2.90100000 \cdot 10^{-16}$ |
| 3900                  | $2.51719120 \cdot 10^{-16}$ | $2.51720000 \cdot 10^{-16}$ |
| 3925                  | $2.18538700 \cdot 10^{-16}$ | $2.18540000 \cdot 10^{-16}$ |
| 3950                  | $1.89809110 \cdot 10^{-16}$ | $1.89810000 \cdot 10^{-16}$ |
| 3975                  | $1.64469440 \cdot 10^{-16}$ | $1.64470000 \cdot 10^{-16}$ |
| 4000                  | $1.42632000 \cdot 10^{-16}$ | $1.42640000 \cdot 10^{-16}$ |
| 4025                  | $1.24109310 \cdot 10^{-16}$ | $1.24110000 \cdot 10^{-16}$ |
| 4050                  | $1.07490780 \cdot 10^{-16}$ | $1.07500000 \cdot 10^{-16}$ |
| 4075                  | $9.33770160 \cdot 10^{-17}$ | $9.33780000 \cdot 10^{-17}$ |

Continued on next page

Table 14 – continued from previous page

| $\log X_0 = \log X_1$ | $M_0$                       | $m_0$                       |
|-----------------------|-----------------------------|-----------------------------|
| 4100                  | $8.10365290 \cdot 10^{-17}$ | $8.10370000 \cdot 10^{-17}$ |
| 4125                  | $7.03750160 \cdot 10^{-17}$ | $7.03760000 \cdot 10^{-17}$ |
| 4150                  | $6.12357670 \cdot 10^{-17}$ | $6.12360000 \cdot 10^{-17}$ |
| 4175                  | $5.31166970 \cdot 10^{-17}$ | $5.31170000 \cdot 10^{-17}$ |
| 4200                  | $4.61437750 \cdot 10^{-17}$ | $4.61440000 \cdot 10^{-17}$ |
| 4225                  | $4.01100610 \cdot 10^{-17}$ | $4.01110000 \cdot 10^{-17}$ |
| 4250                  | $3.48831260 \cdot 10^{-17}$ | $3.48840000 \cdot 10^{-17}$ |
| 4275                  | $3.03166350 \cdot 10^{-17}$ | $3.03170000 \cdot 10^{-17}$ |
| 4300                  | $2.63489850 \cdot 10^{-17}$ | $2.63490000 \cdot 10^{-17}$ |
| 4325                  | $2.29125190 \cdot 10^{-17}$ | $2.29130000 \cdot 10^{-17}$ |
| 4350                  | $1.99336840 \cdot 10^{-17}$ | $1.99340000 \cdot 10^{-17}$ |
| 4375                  | $1.73349970 \cdot 10^{-17}$ | $1.73350000 \cdot 10^{-17}$ |
| 4400                  | $1.50832610 \cdot 10^{-17}$ | $1.50840000 \cdot 10^{-17}$ |
| 4425                  | $1.31316780 \cdot 10^{-17}$ | $1.31320000 \cdot 10^{-17}$ |
| 4450                  | $1.14355970 \cdot 10^{-17}$ | $1.14360000 \cdot 10^{-17}$ |
| 4475                  | $9.96262310 \cdot 10^{-18}$ | $9.96270000 \cdot 10^{-18}$ |
| 4500                  | $8.68294660 \cdot 10^{-18}$ | $8.68300000 \cdot 10^{-18}$ |
| 4525                  | $7.57051470 \cdot 10^{-18}$ | $7.57060000 \cdot 10^{-18}$ |
| 4550                  | $6.59130160 \cdot 10^{-18}$ | $6.59140000 \cdot 10^{-18}$ |
| 4575                  | $5.73993010 \cdot 10^{-18}$ | $5.74000000 \cdot 10^{-18}$ |
| 4600                  | $5.00696180 \cdot 10^{-18}$ | $5.00700000 \cdot 10^{-18}$ |
| 4625                  | $4.35685140 \cdot 10^{-18}$ | $4.35690000 \cdot 10^{-18}$ |
| 4650                  | $3.79748990 \cdot 10^{-18}$ | $3.79750000 \cdot 10^{-18}$ |
| 4675                  | $3.31118720 \cdot 10^{-18}$ | $3.31120000 \cdot 10^{-18}$ |
| 4700                  | $2.88844300 \cdot 10^{-18}$ | $2.88850000 \cdot 10^{-18}$ |
| 4725                  | $2.52130700 \cdot 10^{-18}$ | $2.52140000 \cdot 10^{-18}$ |
| 4750                  | $2.19708580 \cdot 10^{-18}$ | $2.19710000 \cdot 10^{-18}$ |
| 4775                  | $1.91445270 \cdot 10^{-18}$ | $1.91450000 \cdot 10^{-18}$ |
| 4800                  | $1.66915450 \cdot 10^{-18}$ | $1.66920000 \cdot 10^{-18}$ |
| 4825                  | $1.45596610 \cdot 10^{-18}$ | $1.45600000 \cdot 10^{-18}$ |
| 4850                  | $1.27078940 \cdot 10^{-18}$ | $1.27080000 \cdot 10^{-18}$ |
| 4875                  | $1.10940340 \cdot 10^{-18}$ | $1.10950000 \cdot 10^{-18}$ |
| 4900                  | $9.68935730 \cdot 10^{-19}$ | $9.68940000 \cdot 10^{-19}$ |
| 4925                  | $8.46009520 \cdot 10^{-19}$ | $8.46010000 \cdot 10^{-19}$ |
| 4950                  | $7.38303130 \cdot 10^{-19}$ | $7.38310000 \cdot 10^{-19}$ |
| 4975                  | $6.44570570 \cdot 10^{-19}$ | $6.44580000 \cdot 10^{-19}$ |
| 5000                  | $5.63029630 \cdot 10^{-19}$ | $5.63030000 \cdot 10^{-19}$ |
| 5100                  | $3.28585970 \cdot 10^{-19}$ | $3.28590000 \cdot 10^{-19}$ |
| 5200                  | $1.92169390 \cdot 10^{-19}$ | $1.92170000 \cdot 10^{-19}$ |
| 5300                  | $1.12919400 \cdot 10^{-19}$ | $1.12920000 \cdot 10^{-19}$ |
| 5400                  | $6.63116500 \cdot 10^{-20}$ | $6.63120000 \cdot 10^{-20}$ |
| 5500                  | $3.91347680 \cdot 10^{-20}$ | $3.91350000 \cdot 10^{-20}$ |
| 5600                  | $2.31877400 \cdot 10^{-20}$ | $2.31880000 \cdot 10^{-20}$ |
| 5700                  | $1.38066280 \cdot 10^{-20}$ | $1.38070000 \cdot 10^{-20}$ |
| 5800                  | $8.22343310 \cdot 10^{-21}$ | $8.22350000 \cdot 10^{-21}$ |
| 5900                  | $4.91369400 \cdot 10^{-21}$ | $4.91370000 \cdot 10^{-21}$ |
| 6000                  | $2.94287010 \cdot 10^{-21}$ | $2.94290000 \cdot 10^{-21}$ |
| 6100                  | $1.77211030 \cdot 10^{-21}$ | $1.77220000 \cdot 10^{-21}$ |
| 6200                  | $1.06631120 \cdot 10^{-21}$ | $1.06640000 \cdot 10^{-21}$ |
| 6300                  | $6.44801210 \cdot 10^{-22}$ | $6.44810000 \cdot 10^{-22}$ |
| 6400                  | $3.92011870 \cdot 10^{-22}$ | $3.92020000 \cdot 10^{-22}$ |
| 6500                  | $2.38492250 \cdot 10^{-22}$ | $2.38500000 \cdot 10^{-22}$ |
| 6600                  | $1.45203620 \cdot 10^{-22}$ | $1.45210000 \cdot 10^{-22}$ |
| 6700                  | $8.88925300 \cdot 10^{-23}$ | $8.88930000 \cdot 10^{-23}$ |
| 6800                  | $5.45667580 \cdot 10^{-23}$ | $5.45670000 \cdot 10^{-23}$ |

Continued on next page



Table 14 – continued from previous page

| $\log X_0 = \log X_1$ | $M_0$                       | $m_0$                       |
|-----------------------|-----------------------------|-----------------------------|
| 6900                  | $3.36487440 \cdot 10^{-23}$ | $3.36490000 \cdot 10^{-23}$ |
| 7000                  | $2.07654310 \cdot 10^{-23}$ | $2.07660000 \cdot 10^{-23}$ |
| 7100                  | $1.28924250 \cdot 10^{-23}$ | $1.28930000 \cdot 10^{-23}$ |
| 7200                  | $8.02753400 \cdot 10^{-24}$ | $8.02760000 \cdot 10^{-24}$ |
| 7300                  | $5.00185720 \cdot 10^{-24}$ | $5.00190000 \cdot 10^{-24}$ |
| 7400                  | $3.13176600 \cdot 10^{-24}$ | $3.13180000 \cdot 10^{-24}$ |
| 7500                  | $1.96149510 \cdot 10^{-24}$ | $1.96150000 \cdot 10^{-24}$ |
| 7600                  | $1.23144850 \cdot 10^{-24}$ | $1.23150000 \cdot 10^{-24}$ |
| 7700                  | $7.76528970 \cdot 10^{-25}$ | $7.76530000 \cdot 10^{-25}$ |
| 7800                  | $4.91280560 \cdot 10^{-25}$ | $4.91290000 \cdot 10^{-25}$ |
| 7900                  | $3.11597790 \cdot 10^{-25}$ | $3.11600000 \cdot 10^{-25}$ |
| 8000                  | $1.97610170 \cdot 10^{-25}$ | $1.97620000 \cdot 10^{-25}$ |
| 8100                  | $1.25928340 \cdot 10^{-25}$ | $1.25930000 \cdot 10^{-25}$ |
| 8200                  | $8.05157250 \cdot 10^{-26}$ | $8.05160000 \cdot 10^{-26}$ |
| 8300                  | $5.14962470 \cdot 10^{-26}$ | $5.14970000 \cdot 10^{-26}$ |
| 8400                  | $3.30640070 \cdot 10^{-26}$ | $3.30650000 \cdot 10^{-26}$ |
| 8500                  | $2.12969510 \cdot 10^{-26}$ | $2.12970000 \cdot 10^{-26}$ |
| 8600                  | $1.37708930 \cdot 10^{-26}$ | $1.37710000 \cdot 10^{-26}$ |
| 8700                  | $8.88865920 \cdot 10^{-27}$ | $8.88870000 \cdot 10^{-27}$ |
| 8800                  | $5.79602940 \cdot 10^{-27}$ | $5.79610000 \cdot 10^{-27}$ |
| 8900                  | $3.76469220 \cdot 10^{-27}$ | $3.76470000 \cdot 10^{-27}$ |
| 9000                  | $2.44531000 \cdot 10^{-27}$ | $2.44540000 \cdot 10^{-27}$ |
| 9100                  | $1.59142170 \cdot 10^{-27}$ | $1.59150000 \cdot 10^{-27}$ |
| 9200                  | $1.04061600 \cdot 10^{-27}$ | $1.04070000 \cdot 10^{-27}$ |
| 9300                  | $6.82923950 \cdot 10^{-28}$ | $6.82930000 \cdot 10^{-28}$ |
| 9400                  | $4.52330570 \cdot 10^{-28}$ | $4.52340000 \cdot 10^{-28}$ |
| 9500                  | $2.97000660 \cdot 10^{-28}$ | $2.97010000 \cdot 10^{-28}$ |
| 9600                  | $1.96481940 \cdot 10^{-28}$ | $1.96490000 \cdot 10^{-28}$ |
| 9700                  | $1.29478450 \cdot 10^{-28}$ | $1.29480000 \cdot 10^{-28}$ |
| 9800                  | $8.56974260 \cdot 10^{-29}$ | $8.56980000 \cdot 10^{-29}$ |
| 9900                  | $5.73952730 \cdot 10^{-29}$ | $5.73960000 \cdot 10^{-29}$ |
| 10000                 | $3.78492020 \cdot 10^{-29}$ | $3.78500000 \cdot 10^{-29}$ |
| 10100                 | $2.52402540 \cdot 10^{-29}$ | $2.52410000 \cdot 10^{-29}$ |
| 10200                 | $1.68824150 \cdot 10^{-29}$ | $1.68830000 \cdot 10^{-29}$ |
| 10300                 | $1.12823880 \cdot 10^{-29}$ | $1.12830000 \cdot 10^{-29}$ |
| 10400                 | $7.57674890 \cdot 10^{-30}$ | $7.57680000 \cdot 10^{-30}$ |
| 10500                 | $5.10152880 \cdot 10^{-30}$ | $5.10160000 \cdot 10^{-30}$ |
| 10600                 | $3.44342720 \cdot 10^{-30}$ | $3.44350000 \cdot 10^{-30}$ |
| 10700                 | $2.32868900 \cdot 10^{-30}$ | $2.32870000 \cdot 10^{-30}$ |
| 10800                 | $1.57805180 \cdot 10^{-30}$ | $1.57810000 \cdot 10^{-30}$ |
| 10900                 | $1.05809280 \cdot 10^{-30}$ | $1.05810000 \cdot 10^{-30}$ |
| 11000                 | $7.14263470 \cdot 10^{-31}$ | $7.14270000 \cdot 10^{-31}$ |
| 11100                 | $4.83532160 \cdot 10^{-31}$ | $4.83540000 \cdot 10^{-31}$ |
| 11200                 | $3.28491050 \cdot 10^{-31}$ | $3.28500000 \cdot 10^{-31}$ |
| 11300                 | $2.23761050 \cdot 10^{-31}$ | $2.23770000 \cdot 10^{-31}$ |
| 11400                 | $1.52776500 \cdot 10^{-31}$ | $1.52780000 \cdot 10^{-31}$ |
| 11500                 | $1.04328360 \cdot 10^{-31}$ | $1.04330000 \cdot 10^{-31}$ |
| 11600                 | $7.13199660 \cdot 10^{-32}$ | $7.13200000 \cdot 10^{-32}$ |
| 11700                 | $4.88910860 \cdot 10^{-32}$ | $4.88920000 \cdot 10^{-32}$ |
| 11800                 | $3.36020650 \cdot 10^{-32}$ | $3.36030000 \cdot 10^{-32}$ |
| 11900                 | $2.31462190 \cdot 10^{-32}$ | $2.31470000 \cdot 10^{-32}$ |
| 12000                 | $1.59754600 \cdot 10^{-32}$ | $1.59760000 \cdot 10^{-32}$ |
| 12100                 | $1.10470040 \cdot 10^{-32}$ | $1.10480000 \cdot 10^{-32}$ |
| 12200                 | $7.57285640 \cdot 10^{-33}$ | $7.57290000 \cdot 10^{-33}$ |
| 12300                 | $5.24747240 \cdot 10^{-33}$ | $5.24750000 \cdot 10^{-33}$ |

Continued on next page

Table 14 – continued from previous page

| $\log X_0 = \log X_1$ | $M_0$                       | $m_0$                       |
|-----------------------|-----------------------------|-----------------------------|
| 12400                 | $3.64313520 \cdot 10^{-33}$ | $3.64320000 \cdot 10^{-33}$ |
| 12500                 | $2.53361130 \cdot 10^{-33}$ | $2.53370000 \cdot 10^{-33}$ |
| 12600                 | $1.75644830 \cdot 10^{-33}$ | $1.75650000 \cdot 10^{-33}$ |
| 12700                 | $1.21867480 \cdot 10^{-33}$ | $1.21870000 \cdot 10^{-33}$ |
| 12800                 | $8.48023480 \cdot 10^{-34}$ | $8.48030000 \cdot 10^{-34}$ |
| 12900                 | $5.91533320 \cdot 10^{-34}$ | $5.91540000 \cdot 10^{-34}$ |
| 13000                 | $4.13553930 \cdot 10^{-34}$ | $4.13560000 \cdot 10^{-34}$ |
| 13500                 | $7.21538000 \cdot 10^{-35}$ | $7.21540000 \cdot 10^{-35}$ |
| 13800.7464            | $2.54230000 \cdot 10^{-35}$ | $2.54240000 \cdot 10^{-35}$ |
| 14000                 | $1.22654420 \cdot 10^{-35}$ | $1.22660000 \cdot 10^{-35}$ |
| 15000                 | $4.10695780 \cdot 10^{-37}$ | $4.10700000 \cdot 10^{-37}$ |
| 16000                 | $1.51401400 \cdot 10^{-38}$ | $1.51410000 \cdot 10^{-38}$ |
| 17000                 | $6.20396540 \cdot 10^{-40}$ | $6.20400000 \cdot 10^{-40}$ |
| 18000                 | $2.82832570 \cdot 10^{-41}$ | $2.82840000 \cdot 10^{-41}$ |
| 19000                 | $1.36784760 \cdot 10^{-42}$ | $1.36790000 \cdot 10^{-42}$ |
| 20000                 | $7.16208580 \cdot 10^{-44}$ | $7.16210000 \cdot 10^{-44}$ |
| 21000                 | $4.11841260 \cdot 10^{-45}$ | $4.11850000 \cdot 10^{-45}$ |
| 22000                 | $2.43915550 \cdot 10^{-46}$ | $2.43920000 \cdot 10^{-46}$ |
| 23000                 | $1.56473610 \cdot 10^{-47}$ | $1.56480000 \cdot 10^{-47}$ |
| 24000                 | $1.07021370 \cdot 10^{-48}$ | $1.07030000 \cdot 10^{-48}$ |
| 25000                 | $7.57239210 \cdot 10^{-50}$ | $7.57240000 \cdot 10^{-50}$ |

8. TABLE 15: VALUES FOR THEOREM 2 FOR  $k \in \{1, 2, 3, 4, 5\}$ .

TABLE 15. Values of  $m_k = M_k$  in  $|\theta(x) - x| < \frac{m_k x}{(\log x)^k}$  as in Theorem 1 of [1]. Combined theoretical results from Table 8, 11, and 12. Each value is valid for  $x \geq X_0 = X_1$ . Note that for  $x \leq 10^{19}$ , we have  $M_k = 0$ , and for  $x \leq e^{27}$ , we have numerical results in Table 13. Computed using  $J_0 = \log(7 \cdot 10^{11})$ ,  $J = 43$ .

| $\log X_0 = \log X_1$   | $m_1 = M_1$            | $m_2 = M_2$            | $m_3 = M_3$            | $m_4 = M_4$         | $m_5 = M_5$         |
|-------------------------|------------------------|------------------------|------------------------|---------------------|---------------------|
| 0                       | $1.2323 \cdot 10^0$    | $3.9649 \cdot 10^0$    | $2.0829 \cdot 10^1$    | $1.5123 \cdot 10^2$ | $1.3441 \cdot 10^5$ |
| $\log(10^5)$            | $5.5316 \cdot 10^{-2}$ | $6.4673 \cdot 10^{-1}$ | $7.5612 \cdot 10^0$    | $8.9346 \cdot 10^1$ | $1.3441 \cdot 10^5$ |
| $\log(5 \cdot 10^5)$    | $2.6724 \cdot 10^{-2}$ | $3.5744 \cdot 10^{-1}$ | $4.7808 \cdot 10^0$    | $6.3944 \cdot 10^1$ | $1.3441 \cdot 10^5$ |
| $\log(10^6)$            | $2.3240 \cdot 10^{-2}$ | $3.2309 \cdot 10^{-1}$ | $4.4916 \cdot 10^0$    | $6.2444 \cdot 10^1$ | $1.3441 \cdot 10^5$ |
| $\log(5 \cdot 10^6)$    | $1.0236 \cdot 10^{-2}$ | $1.5952 \cdot 10^{-1}$ | $2.4860 \cdot 10^0$    | $5.7184 \cdot 10^1$ | $1.3441 \cdot 10^5$ |
| $\log(10^7)$            | $8.4725 \cdot 10^{-3}$ | $1.3675 \cdot 10^{-1}$ | $2.2071 \cdot 10^0$    | $5.7184 \cdot 10^1$ | $1.3441 \cdot 10^5$ |
| $\log(5 \cdot 10^7)$    | $3.8550 \cdot 10^{-3}$ | $6.8701 \cdot 10^{-2}$ | $1.2244 \cdot 10^0$    | $5.7184 \cdot 10^1$ | $1.3441 \cdot 10^5$ |
| $\log(10^8)$            | $2.7457 \cdot 10^{-3}$ | $5.0612 \cdot 10^{-2}$ | $9.4259 \cdot 10^{-1}$ | $5.7184 \cdot 10^1$ | $1.3441 \cdot 10^5$ |
| $\log(10^9)$            | $9.5913 \cdot 10^{-4}$ | $2.0087 \cdot 10^{-2}$ | $4.2065 \cdot 10^{-1}$ | $5.7184 \cdot 10^1$ | $1.3441 \cdot 10^5$ |
| $\log(10^{10})$         | $3.7787 \cdot 10^{-4}$ | $8.7526 \cdot 10^{-3}$ | $2.0274 \cdot 10^{-1}$ | $5.7184 \cdot 10^1$ | $1.3441 \cdot 10^5$ |
| $\log(19035709163)$     | $2.6773 \cdot 10^{-4}$ | $6.3370 \cdot 10^{-3}$ | $1.5000 \cdot 10^{-1}$ | $5.7184 \cdot 10^1$ | $1.3441 \cdot 10^5$ |
| $\log(2 \cdot 10^{10})$ | $2.4601 \cdot 10^{-4}$ | $5.8365 \cdot 10^{-3}$ | $1.3848 \cdot 10^{-1}$ | $5.7184 \cdot 10^1$ | $1.3441 \cdot 10^5$ |
| $\log(5 \cdot 10^{10})$ | $1.8556 \cdot 10^{-4}$ | $4.5722 \cdot 10^{-3}$ | $1.1266 \cdot 10^{-1}$ | $5.7184 \cdot 10^1$ | $1.3441 \cdot 10^5$ |
| $\log(10^{11})$         | $1.3392 \cdot 10^{-4}$ | $3.4053 \cdot 10^{-3}$ | $8.6589 \cdot 10^{-2}$ | $5.7184 \cdot 10^1$ | $1.3441 \cdot 10^5$ |
| $\log(2 \cdot 10^{11})$ | $7.8683 \cdot 10^{-5}$ | $2.0591 \cdot 10^{-3}$ | $5.3886 \cdot 10^{-2}$ | $5.7184 \cdot 10^1$ | $1.3441 \cdot 10^5$ |
| $\log(3 \cdot 10^{11})$ | $7.0193 \cdot 10^{-5}$ | $1.8758 \cdot 10^{-3}$ | $5.0536 \cdot 10^{-2}$ | $5.7184 \cdot 10^1$ | $1.3441 \cdot 10^5$ |
| $\log(4 \cdot 10^{11})$ | $7.0193 \cdot 10^{-5}$ | $1.8758 \cdot 10^{-3}$ | $5.0536 \cdot 10^{-2}$ | $5.7184 \cdot 10^1$ | $1.3441 \cdot 10^5$ |
| $\log(5 \cdot 10^{11})$ | $6.9322 \cdot 10^{-5}$ | $1.8717 \cdot 10^{-3}$ | $5.0536 \cdot 10^{-2}$ | $5.7184 \cdot 10^1$ | $1.3441 \cdot 10^5$ |
| $\log(6 \cdot 10^{11})$ | $6.9322 \cdot 10^{-5}$ | $1.8717 \cdot 10^{-3}$ | $5.0536 \cdot 10^{-2}$ | $5.7184 \cdot 10^1$ | $1.3441 \cdot 10^5$ |
| 28                      | $4.3555 \cdot 10^{-5}$ | $1.2196 \cdot 10^{-3}$ | $3.4148 \cdot 10^{-2}$ | $5.7184 \cdot 10^1$ | $1.3441 \cdot 10^5$ |
| 29                      | $2.7336 \cdot 10^{-5}$ | $7.9272 \cdot 10^{-4}$ | $2.4334 \cdot 10^{-2}$ | $5.7184 \cdot 10^1$ | $1.3441 \cdot 10^5$ |
| 30                      | $1.7139 \cdot 10^{-5}$ | $5.1415 \cdot 10^{-4}$ | $2.4334 \cdot 10^{-2}$ | $5.7184 \cdot 10^1$ | $1.3441 \cdot 10^5$ |
| 31                      | $1.0735 \cdot 10^{-5}$ | $3.3277 \cdot 10^{-4}$ | $2.4334 \cdot 10^{-2}$ | $5.7184 \cdot 10^1$ | $1.3441 \cdot 10^5$ |
| 32                      | $7.0053 \cdot 10^{-6}$ | $2.2417 \cdot 10^{-4}$ | $2.4334 \cdot 10^{-2}$ | $5.7184 \cdot 10^1$ | $1.3441 \cdot 10^5$ |
| 33                      | $4.3798 \cdot 10^{-6}$ | $1.4454 \cdot 10^{-4}$ | $2.4334 \cdot 10^{-2}$ | $5.7184 \cdot 10^1$ | $1.3441 \cdot 10^5$ |
| 34                      | $2.7360 \cdot 10^{-6}$ | $9.3023 \cdot 10^{-5}$ | $2.4334 \cdot 10^{-2}$ | $5.7184 \cdot 10^1$ | $1.3441 \cdot 10^5$ |
| 35                      | $1.7078 \cdot 10^{-6}$ | $5.9771 \cdot 10^{-5}$ | $2.4334 \cdot 10^{-2}$ | $5.7184 \cdot 10^1$ | $1.3441 \cdot 10^5$ |
| 36                      | $1.0652 \cdot 10^{-6}$ | $3.8345 \cdot 10^{-5}$ | $2.4334 \cdot 10^{-2}$ | $5.7184 \cdot 10^1$ | $1.3441 \cdot 10^5$ |
| 37                      | $8.6315 \cdot 10^{-7}$ | $3.7979 \cdot 10^{-5}$ | $2.4334 \cdot 10^{-2}$ | $5.7184 \cdot 10^1$ | $1.3441 \cdot 10^5$ |
| 38                      | $8.6315 \cdot 10^{-7}$ | $3.7979 \cdot 10^{-5}$ | $2.4334 \cdot 10^{-2}$ | $5.7184 \cdot 10^1$ | $1.3441 \cdot 10^5$ |
| 39                      | $8.6315 \cdot 10^{-7}$ | $3.7979 \cdot 10^{-5}$ | $2.4334 \cdot 10^{-2}$ | $5.7184 \cdot 10^1$ | $1.3441 \cdot 10^5$ |
| 40                      | $8.6315 \cdot 10^{-7}$ | $3.7979 \cdot 10^{-5}$ | $2.4334 \cdot 10^{-2}$ | $5.7184 \cdot 10^1$ | $1.3441 \cdot 10^5$ |
| 41                      | $8.6315 \cdot 10^{-7}$ | $3.7979 \cdot 10^{-5}$ | $2.4334 \cdot 10^{-2}$ | $5.7184 \cdot 10^1$ | $1.3441 \cdot 10^5$ |
| 42                      | $8.6315 \cdot 10^{-7}$ | $3.7979 \cdot 10^{-5}$ | $2.4334 \cdot 10^{-2}$ | $5.7184 \cdot 10^1$ | $1.3441 \cdot 10^5$ |
| 43                      | $8.6315 \cdot 10^{-7}$ | $3.7979 \cdot 10^{-5}$ | $2.4334 \cdot 10^{-2}$ | $5.7184 \cdot 10^1$ | $1.3441 \cdot 10^5$ |
| $19 \log(10)$           | $8.6315 \cdot 10^{-7}$ | $3.7979 \cdot 10^{-5}$ | $2.4334 \cdot 10^{-2}$ | $5.7184 \cdot 10^1$ | $1.3441 \cdot 10^5$ |
| 44                      | $7.8163 \cdot 10^{-7}$ | $3.5174 \cdot 10^{-5}$ | $2.4334 \cdot 10^{-2}$ | $5.7184 \cdot 10^1$ | $1.3441 \cdot 10^5$ |
| 45                      | $5.0646 \cdot 10^{-7}$ | $2.3298 \cdot 10^{-5}$ | $2.4334 \cdot 10^{-2}$ | $5.7184 \cdot 10^1$ | $1.3441 \cdot 10^5$ |
| 46                      | $3.2935 \cdot 10^{-7}$ | $1.5480 \cdot 10^{-5}$ | $2.4334 \cdot 10^{-2}$ | $5.7184 \cdot 10^1$ | $1.3441 \cdot 10^5$ |
| 47                      | $2.1308 \cdot 10^{-7}$ | $1.0376 \cdot 10^{-5}$ | $2.4334 \cdot 10^{-2}$ | $5.7184 \cdot 10^1$ | $1.3441 \cdot 10^5$ |
| 48                      | $1.3791 \cdot 10^{-7}$ | $1.0376 \cdot 10^{-5}$ | $2.4334 \cdot 10^{-2}$ | $5.7184 \cdot 10^1$ | $1.3441 \cdot 10^5$ |
| 49                      | $8.9140 \cdot 10^{-8}$ | $1.0376 \cdot 10^{-5}$ | $2.4334 \cdot 10^{-2}$ | $5.7184 \cdot 10^1$ | $1.3441 \cdot 10^5$ |
| 50                      | $5.7545 \cdot 10^{-8}$ | $1.0376 \cdot 10^{-5}$ | $2.4334 \cdot 10^{-2}$ | $5.7184 \cdot 10^1$ | $1.3441 \cdot 10^5$ |
| 51                      | $3.7147 \cdot 10^{-8}$ | $1.0376 \cdot 10^{-5}$ | $2.4334 \cdot 10^{-2}$ | $5.7184 \cdot 10^1$ | $1.3441 \cdot 10^5$ |
| 52                      | $2.3898 \cdot 10^{-8}$ | $1.0376 \cdot 10^{-5}$ | $2.4334 \cdot 10^{-2}$ | $5.7184 \cdot 10^1$ | $1.3441 \cdot 10^5$ |
| 53                      | $1.5373 \cdot 10^{-8}$ | $1.0376 \cdot 10^{-5}$ | $2.4334 \cdot 10^{-2}$ | $5.7184 \cdot 10^1$ | $1.3441 \cdot 10^5$ |
| 54                      | $9.8778 \cdot 10^{-9}$ | $1.0376 \cdot 10^{-5}$ | $2.4334 \cdot 10^{-2}$ | $5.7184 \cdot 10^1$ | $1.3441 \cdot 10^5$ |

Continued on next page



Table 15 – continued from previous page

| $\log X_0 = \log X_1$ | $m_1 = M_1$             | $m_2 = M_2$            | $m_3 = M_3$            | $m_4 = M_4$            | $m_5 = M_5$         |
|-----------------------|-------------------------|------------------------|------------------------|------------------------|---------------------|
| 2450                  | $3.0228 \cdot 10^{-9}$  | $7.4814 \cdot 10^{-6}$ | $1.8517 \cdot 10^{-2}$ | $4.5829 \cdot 10^1$    | $1.1343 \cdot 10^5$ |
| 2475                  | $2.6279 \cdot 10^{-9}$  | $6.5696 \cdot 10^{-6}$ | $1.6424 \cdot 10^{-2}$ | $4.1060 \cdot 10^1$    | $1.0265 \cdot 10^5$ |
| 2500                  | $2.2885 \cdot 10^{-9}$  | $5.7783 \cdot 10^{-6}$ | $1.4591 \cdot 10^{-2}$ | $3.6840 \cdot 10^1$    | $9.3021 \cdot 10^4$ |
| 2525                  | $1.9873 \cdot 10^{-9}$  | $5.0676 \cdot 10^{-6}$ | $1.2923 \cdot 10^{-2}$ | $3.2952 \cdot 10^1$    | $8.4028 \cdot 10^4$ |
| 2550                  | $1.7270 \cdot 10^{-9}$  | $4.4471 \cdot 10^{-6}$ | $1.1452 \cdot 10^{-2}$ | $2.9487 \cdot 10^1$    | $7.5928 \cdot 10^4$ |
| 2575                  | $1.4992 \cdot 10^{-9}$  | $3.8979 \cdot 10^{-6}$ | $1.0135 \cdot 10^{-2}$ | $2.6350 \cdot 10^1$    | $6.8510 \cdot 10^4$ |
| 2600                  | $1.3023 \cdot 10^{-9}$  | $3.4184 \cdot 10^{-6}$ | $8.9732 \cdot 10^{-3}$ | $2.3555 \cdot 10^1$    | $6.1831 \cdot 10^4$ |
| 2625                  | $1.1314 \cdot 10^{-9}$  | $2.9981 \cdot 10^{-6}$ | $7.9450 \cdot 10^{-3}$ | $2.1055 \cdot 10^1$    | $5.5794 \cdot 10^4$ |
| 2650                  | $9.8296 \cdot 10^{-10}$ | $2.6295 \cdot 10^{-6}$ | $7.0337 \cdot 10^{-3}$ | $1.8816 \cdot 10^1$    | $5.0331 \cdot 10^4$ |
| 2675                  | $8.5432 \cdot 10^{-10}$ | $2.3067 \cdot 10^{-6}$ | $6.2280 \cdot 10^{-3}$ | $1.6816 \cdot 10^1$    | $4.5402 \cdot 10^4$ |
| 2700                  | $7.4234 \cdot 10^{-10}$ | $2.0229 \cdot 10^{-6}$ | $5.5124 \cdot 10^{-3}$ | $1.5022 \cdot 10^1$    | $4.0933 \cdot 10^4$ |
| 2725                  | $6.4498 \cdot 10^{-10}$ | $1.7737 \cdot 10^{-6}$ | $4.8777 \cdot 10^{-3}$ | $1.3414 \cdot 10^1$    | $3.6888 \cdot 10^4$ |
| 2750                  | $5.6072 \cdot 10^{-10}$ | $1.5560 \cdot 10^{-6}$ | $4.3179 \cdot 10^{-3}$ | $1.1982 \cdot 10^1$    | $3.3250 \cdot 10^4$ |
| 2775                  | $4.8730 \cdot 10^{-10}$ | $1.3645 \cdot 10^{-6}$ | $3.8204 \cdot 10^{-3}$ | $1.0698 \cdot 10^1$    | $2.9952 \cdot 10^4$ |
| 2800                  | $4.2389 \cdot 10^{-10}$ | $1.1975 \cdot 10^{-6}$ | $3.3829 \cdot 10^{-3}$ | $9.5566 \cdot 10^0$    | $2.6998 \cdot 10^4$ |
| 2825                  | $3.6912 \cdot 10^{-10}$ | $1.0520 \cdot 10^{-6}$ | $2.9982 \cdot 10^{-3}$ | $8.5447 \cdot 10^0$    | $2.4353 \cdot 10^4$ |
| 2850                  | $3.2168 \cdot 10^{-10}$ | $9.2482 \cdot 10^{-7}$ | $2.6589 \cdot 10^{-3}$ | $7.6442 \cdot 10^0$    | $2.1977 \cdot 10^4$ |
| 2875                  | $2.7953 \cdot 10^{-10}$ | $8.1063 \cdot 10^{-7}$ | $2.3509 \cdot 10^{-3}$ | $6.8174 \cdot 10^0$    | $1.9771 \cdot 10^4$ |
| 2900                  | $2.4327 \cdot 10^{-10}$ | $7.1154 \cdot 10^{-7}$ | $2.0813 \cdot 10^{-3}$ | $6.0877 \cdot 10^0$    | $1.7807 \cdot 10^4$ |
| 2925                  | $2.1141 \cdot 10^{-10}$ | $6.2364 \cdot 10^{-7}$ | $1.8398 \cdot 10^{-3}$ | $5.4272 \cdot 10^0$    | $1.6011 \cdot 10^4$ |
| 2950                  | $1.8391 \cdot 10^{-10}$ | $5.4712 \cdot 10^{-7}$ | $1.6277 \cdot 10^{-3}$ | $4.8424 \cdot 10^0$    | $1.4406 \cdot 10^4$ |
| 2975                  | $1.6015 \cdot 10^{-10}$ | $4.8044 \cdot 10^{-7}$ | $1.4414 \cdot 10^{-3}$ | $4.3240 \cdot 10^0$    | $1.2972 \cdot 10^4$ |
| 3000                  | $1.3915 \cdot 10^{-10}$ | $4.2091 \cdot 10^{-7}$ | $1.2733 \cdot 10^{-3}$ | $3.8516 \cdot 10^0$    | $1.1651 \cdot 10^4$ |
| 3025                  | $1.2115 \cdot 10^{-10}$ | $3.6950 \cdot 10^{-7}$ | $1.1270 \cdot 10^{-3}$ | $3.4373 \cdot 10^0$    | $1.0484 \cdot 10^4$ |
| 3050                  | $1.0531 \cdot 10^{-10}$ | $3.2382 \cdot 10^{-7}$ | $9.9573 \cdot 10^{-4}$ | $3.0619 \cdot 10^0$    | $9.4153 \cdot 10^3$ |
| 3075                  | $9.1684 \cdot 10^{-11}$ | $2.8422 \cdot 10^{-7}$ | $8.8109 \cdot 10^{-4}$ | $2.7314 \cdot 10^0$    | $8.4672 \cdot 10^3$ |
| 3100                  | $7.9793 \cdot 10^{-11}$ | $2.4936 \cdot 10^{-7}$ | $7.7923 \cdot 10^{-4}$ | $2.4351 \cdot 10^0$    | $7.6097 \cdot 10^3$ |
| 3125                  | $6.9396 \cdot 10^{-11}$ | $2.1860 \cdot 10^{-7}$ | $6.8859 \cdot 10^{-4}$ | $2.1691 \cdot 10^0$    | $6.8325 \cdot 10^3$ |
| 3150                  | $6.0410 \cdot 10^{-11}$ | $1.9180 \cdot 10^{-7}$ | $6.0897 \cdot 10^{-4}$ | $1.9335 \cdot 10^0$    | $6.1388 \cdot 10^3$ |
| 3175                  | $5.2572 \cdot 10^{-11}$ | $1.6824 \cdot 10^{-7}$ | $5.3834 \cdot 10^{-4}$ | $1.7227 \cdot 10^0$    | $5.5126 \cdot 10^3$ |
| 3200                  | $4.5782 \cdot 10^{-11}$ | $1.4765 \cdot 10^{-7}$ | $4.7616 \cdot 10^{-4}$ | $1.5357 \cdot 10^0$    | $4.9524 \cdot 10^3$ |
| 3225                  | $3.9902 \cdot 10^{-11}$ | $1.2968 \cdot 10^{-7}$ | $4.2146 \cdot 10^{-4}$ | $1.3698 \cdot 10^0$    | $4.4517 \cdot 10^3$ |
| 3250                  | $3.4801 \cdot 10^{-11}$ | $1.1398 \cdot 10^{-7}$ | $3.7326 \cdot 10^{-4}$ | $1.2225 \cdot 10^0$    | $4.0034 \cdot 10^3$ |
| 3275                  | $3.0332 \cdot 10^{-11}$ | $1.0010 \cdot 10^{-7}$ | $3.3031 \cdot 10^{-4}$ | $1.0901 \cdot 10^0$    | $3.5971 \cdot 10^3$ |
| 3300                  | $2.6412 \cdot 10^{-11}$ | $8.7820 \cdot 10^{-8}$ | $2.9200 \cdot 10^{-4}$ | $9.7090 \cdot 10^{-1}$ | $3.2283 \cdot 10^3$ |
| 3325                  | $2.3015 \cdot 10^{-11}$ | $7.7100 \cdot 10^{-8}$ | $2.5829 \cdot 10^{-4}$ | $8.6526 \cdot 10^{-1}$ | $2.8987 \cdot 10^3$ |
| 3350                  | $2.0043 \cdot 10^{-11}$ | $6.7644 \cdot 10^{-8}$ | $2.2830 \cdot 10^{-4}$ | $7.7051 \cdot 10^{-1}$ | $2.6005 \cdot 10^3$ |
| 3375                  | $1.7453 \cdot 10^{-11}$ | $5.9340 \cdot 10^{-8}$ | $2.0176 \cdot 10^{-4}$ | $6.8597 \cdot 10^{-1}$ | $2.3323 \cdot 10^3$ |
| 3400                  | $1.5212 \cdot 10^{-11}$ | $5.2100 \cdot 10^{-8}$ | $1.7844 \cdot 10^{-4}$ | $6.1116 \cdot 10^{-1}$ | $2.0933 \cdot 10^3$ |
| 3425                  | $1.3267 \cdot 10^{-11}$ | $4.5769 \cdot 10^{-8}$ | $1.5791 \cdot 10^{-4}$ | $5.4476 \cdot 10^{-1}$ | $1.8795 \cdot 10^3$ |
| 3450                  | $1.1555 \cdot 10^{-11}$ | $4.0151 \cdot 10^{-8}$ | $1.3953 \cdot 10^{-4}$ | $4.8485 \cdot 10^{-1}$ | $1.6849 \cdot 10^3$ |
| 3475                  | $1.0059 \cdot 10^{-11}$ | $3.5207 \cdot 10^{-8}$ | $1.2323 \cdot 10^{-4}$ | $4.3128 \cdot 10^{-1}$ | $1.5095 \cdot 10^3$ |
| 3500                  | $8.7646 \cdot 10^{-12}$ | $3.0896 \cdot 10^{-8}$ | $1.0891 \cdot 10^{-4}$ | $3.8390 \cdot 10^{-1}$ | $1.3533 \cdot 10^3$ |
| 3525                  | $7.6403 \cdot 10^{-12}$ | $2.7124 \cdot 10^{-8}$ | $9.6287 \cdot 10^{-5}$ | $3.4182 \cdot 10^{-1}$ | $1.2135 \cdot 10^3$ |
| 3550                  | $6.6608 \cdot 10^{-12}$ | $2.3813 \cdot 10^{-8}$ | $8.5129 \cdot 10^{-5}$ | $3.0434 \cdot 10^{-1}$ | $1.0880 \cdot 10^3$ |
| 3575                  | $5.8042 \cdot 10^{-12}$ | $2.0896 \cdot 10^{-8}$ | $7.5223 \cdot 10^{-5}$ | $2.7080 \cdot 10^{-1}$ | $9.7488 \cdot 10^2$ |
| 3600                  | $5.0622 \cdot 10^{-12}$ | $1.8351 \cdot 10^{-8}$ | $6.6520 \cdot 10^{-5}$ | $2.4114 \cdot 10^{-1}$ | $8.7411 \cdot 10^2$ |
| 3625                  | $4.4166 \cdot 10^{-12}$ | $1.6121 \cdot 10^{-8}$ | $5.8840 \cdot 10^{-5}$ | $2.1477 \cdot 10^{-1}$ | $7.8389 \cdot 10^2$ |
| 3650                  | $3.8475 \cdot 10^{-12}$ | $1.4140 \cdot 10^{-8}$ | $5.1963 \cdot 10^{-5}$ | $1.9097 \cdot 10^{-1}$ | $7.0179 \cdot 10^2$ |
| 3675                  | $3.3561 \cdot 10^{-12}$ | $1.2418 \cdot 10^{-8}$ | $4.5944 \cdot 10^{-5}$ | $1.7000 \cdot 10^{-1}$ | $6.2898 \cdot 10^2$ |
| 3700                  | $2.9296 \cdot 10^{-12}$ | $1.0913 \cdot 10^{-8}$ | $4.0650 \cdot 10^{-5}$ | $1.5142 \cdot 10^{-1}$ | $5.6404 \cdot 10^2$ |
| 3725                  | $2.5580 \cdot 10^{-12}$ | $9.5924 \cdot 10^{-9}$ | $3.5972 \cdot 10^{-5}$ | $1.3490 \cdot 10^{-1}$ | $5.0585 \cdot 10^2$ |
| 3750                  | $2.2347 \cdot 10^{-12}$ | $8.4358 \cdot 10^{-9}$ | $3.1845 \cdot 10^{-5}$ | $1.2022 \cdot 10^{-1}$ | $4.5381 \cdot 10^2$ |
| 3775                  | $1.9514 \cdot 10^{-12}$ | $7.4151 \cdot 10^{-9}$ | $2.8178 \cdot 10^{-5}$ | $1.0708 \cdot 10^{-1}$ | $4.0689 \cdot 10^2$ |
| 3800                  | $1.7020 \cdot 10^{-12}$ | $6.5100 \cdot 10^{-9}$ | $2.4901 \cdot 10^{-5}$ | $9.5245 \cdot 10^{-2}$ | $3.6431 \cdot 10^2$ |

Continued on next page

Table 15 – continued from previous page

| $\log X_0 = \log X_1$ | $m_1 = M_1$             | $m_2 = M_2$             | $m_3 = M_3$            | $m_4 = M_4$            | $m_5 = M_5$            |
|-----------------------|-------------------------|-------------------------|------------------------|------------------------|------------------------|
| 3825                  | $1.4855 \cdot 10^{-12}$ | $5.7189 \cdot 10^{-9}$  | $2.2018 \cdot 10^{-5}$ | $8.4768 \cdot 10^{-2}$ | $3.2636 \cdot 10^2$    |
| 3850                  | $1.2973 \cdot 10^{-12}$ | $5.0267 \cdot 10^{-9}$  | $1.9479 \cdot 10^{-5}$ | $7.5479 \cdot 10^{-2}$ | $2.9249 \cdot 10^2$    |
| 3875                  | $1.1314 \cdot 10^{-12}$ | $4.4124 \cdot 10^{-9}$  | $1.7209 \cdot 10^{-5}$ | $6.7112 \cdot 10^{-2}$ | $2.6174 \cdot 10^2$    |
| 3900                  | $9.8800 \cdot 10^{-13}$ | $3.8779 \cdot 10^{-9}$  | $1.5221 \cdot 10^{-5}$ | $5.9742 \cdot 10^{-2}$ | $2.3449 \cdot 10^2$    |
| 3925                  | $8.6323 \cdot 10^{-13}$ | $3.4098 \cdot 10^{-9}$  | $1.3469 \cdot 10^{-5}$ | $5.3201 \cdot 10^{-2}$ | $2.1015 \cdot 10^2$    |
| 3950                  | $7.5450 \cdot 10^{-13}$ | $2.9992 \cdot 10^{-9}$  | $1.1922 \cdot 10^{-5}$ | $4.7388 \cdot 10^{-2}$ | $1.8837 \cdot 10^2$    |
| 3975                  | $6.5788 \cdot 10^{-13}$ | $2.6316 \cdot 10^{-9}$  | $1.0527 \cdot 10^{-5}$ | $4.2105 \cdot 10^{-2}$ | $1.6842 \cdot 10^2$    |
| 4000                  | $5.7410 \cdot 10^{-13}$ | $2.3108 \cdot 10^{-9}$  | $9.3007 \cdot 10^{-6}$ | $3.7436 \cdot 10^{-2}$ | $1.5068 \cdot 10^2$    |
| 4025                  | $5.0265 \cdot 10^{-13}$ | $2.0358 \cdot 10^{-9}$  | $8.2446 \cdot 10^{-6}$ | $3.3391 \cdot 10^{-2}$ | $1.3524 \cdot 10^2$    |
| 4050                  | $4.3803 \cdot 10^{-13}$ | $1.7850 \cdot 10^{-9}$  | $7.2737 \cdot 10^{-6}$ | $2.9641 \cdot 10^{-2}$ | $1.2079 \cdot 10^2$    |
| 4075                  | $3.8285 \cdot 10^{-13}$ | $1.5697 \cdot 10^{-9}$  | $6.4357 \cdot 10^{-6}$ | $2.6387 \cdot 10^{-2}$ | $1.0819 \cdot 10^2$    |
| 4100                  | $3.3428 \cdot 10^{-13}$ | $1.3789 \cdot 10^{-9}$  | $5.6880 \cdot 10^{-6}$ | $2.3463 \cdot 10^{-2}$ | $9.6784 \cdot 10^1$    |
| 4125                  | $2.9206 \cdot 10^{-13}$ | $1.2121 \cdot 10^{-9}$  | $5.0300 \cdot 10^{-6}$ | $2.0875 \cdot 10^{-2}$ | $8.6629 \cdot 10^1$    |
| 4150                  | $2.5566 \cdot 10^{-13}$ | $1.0674 \cdot 10^{-9}$  | $4.4564 \cdot 10^{-6}$ | $1.8606 \cdot 10^{-2}$ | $7.7677 \cdot 10^1$    |
| 4175                  | $2.2310 \cdot 10^{-13}$ | $9.3698 \cdot 10^{-10}$ | $3.9354 \cdot 10^{-6}$ | $1.6529 \cdot 10^{-2}$ | $6.9419 \cdot 10^1$    |
| 4200                  | $1.9496 \cdot 10^{-13}$ | $8.2370 \cdot 10^{-10}$ | $3.4802 \cdot 10^{-6}$ | $1.4704 \cdot 10^{-2}$ | $6.2123 \cdot 10^1$    |
| 4225                  | $1.7047 \cdot 10^{-13}$ | $7.2449 \cdot 10^{-10}$ | $3.0791 \cdot 10^{-6}$ | $1.3087 \cdot 10^{-2}$ | $5.5616 \cdot 10^1$    |
| 4250                  | $1.4913 \cdot 10^{-13}$ | $6.3752 \cdot 10^{-10}$ | $2.7254 \cdot 10^{-6}$ | $1.1651 \cdot 10^{-2}$ | $4.9808 \cdot 10^1$    |
| 4275                  | $1.3037 \cdot 10^{-13}$ | $5.6056 \cdot 10^{-10}$ | $2.4104 \cdot 10^{-6}$ | $1.0365 \cdot 10^{-2}$ | $4.4569 \cdot 10^1$    |
| 4300                  | $1.1396 \cdot 10^{-13}$ | $4.9288 \cdot 10^{-10}$ | $2.1317 \cdot 10^{-6}$ | $9.2196 \cdot 10^{-3}$ | $3.9875 \cdot 10^1$    |
| 4325                  | $9.9670 \cdot 10^{-14}$ | $4.3357 \cdot 10^{-10}$ | $1.8860 \cdot 10^{-6}$ | $8.2041 \cdot 10^{-3}$ | $3.5688 \cdot 10^1$    |
| 4350                  | $8.7210 \cdot 10^{-14}$ | $3.8155 \cdot 10^{-10}$ | $1.6693 \cdot 10^{-6}$ | $7.3030 \cdot 10^{-3}$ | $3.1951 \cdot 10^1$    |
| 4375                  | $7.6274 \cdot 10^{-14}$ | $3.3561 \cdot 10^{-10}$ | $1.4767 \cdot 10^{-6}$ | $6.4974 \cdot 10^{-3}$ | $2.8589 \cdot 10^1$    |
| 4400                  | $6.6744 \cdot 10^{-14}$ | $2.9534 \cdot 10^{-10}$ | $1.3069 \cdot 10^{-6}$ | $5.7830 \cdot 10^{-3}$ | $2.5590 \cdot 10^1$    |
| 4425                  | $5.8436 \cdot 10^{-14}$ | $2.6005 \cdot 10^{-10}$ | $1.1572 \cdot 10^{-6}$ | $5.1495 \cdot 10^{-3}$ | $2.2916 \cdot 10^1$    |
| 4450                  | $5.1175 \cdot 10^{-14}$ | $2.2901 \cdot 10^{-10}$ | $1.0248 \cdot 10^{-6}$ | $4.5860 \cdot 10^{-3}$ | $2.0523 \cdot 10^1$    |
| 4475                  | $4.4832 \cdot 10^{-14}$ | $2.0175 \cdot 10^{-10}$ | $9.0785 \cdot 10^{-7}$ | $4.0853 \cdot 10^{-3}$ | $1.8384 \cdot 10^1$    |
| 4500                  | $3.9291 \cdot 10^{-14}$ | $1.7779 \cdot 10^{-10}$ | $8.0450 \cdot 10^{-7}$ | $3.6404 \cdot 10^{-3}$ | $1.6473 \cdot 10^1$    |
| 4525                  | $3.4446 \cdot 10^{-14}$ | $1.5673 \cdot 10^{-10}$ | $7.1312 \cdot 10^{-7}$ | $3.2447 \cdot 10^{-3}$ | $1.4764 \cdot 10^1$    |
| 4550                  | $3.0156 \cdot 10^{-14}$ | $1.3797 \cdot 10^{-10}$ | $6.3117 \cdot 10^{-7}$ | $2.8876 \cdot 10^{-3}$ | $1.3211 \cdot 10^1$    |
| 4575                  | $2.6404 \cdot 10^{-14}$ | $1.2146 \cdot 10^{-10}$ | $5.5871 \cdot 10^{-7}$ | $2.5701 \cdot 10^{-3}$ | $1.1823 \cdot 10^1$    |
| 4600                  | $2.3158 \cdot 10^{-14}$ | $1.0711 \cdot 10^{-10}$ | $4.9535 \cdot 10^{-7}$ | $2.2910 \cdot 10^{-3}$ | $1.0596 \cdot 10^1$    |
| 4625                  | $2.0260 \cdot 10^{-14}$ | $9.4207 \cdot 10^{-11}$ | $4.3806 \cdot 10^{-7}$ | $2.0370 \cdot 10^{-3}$ | $9.4720 \cdot 10^0$    |
| 4650                  | $1.7754 \cdot 10^{-14}$ | $8.2997 \cdot 10^{-11}$ | $3.8801 \cdot 10^{-7}$ | $1.8140 \cdot 10^{-3}$ | $8.4802 \cdot 10^0$    |
| 4675                  | $1.5563 \cdot 10^{-14}$ | $7.3145 \cdot 10^{-11}$ | $3.4378 \cdot 10^{-7}$ | $1.6158 \cdot 10^{-3}$ | $7.5941 \cdot 10^0$    |
| 4700                  | $1.3648 \cdot 10^{-14}$ | $6.4487 \cdot 10^{-11}$ | $3.0470 \cdot 10^{-7}$ | $1.4397 \cdot 10^{-3}$ | $6.8026 \cdot 10^0$    |
| 4725                  | $1.1977 \cdot 10^{-14}$ | $5.6887 \cdot 10^{-11}$ | $2.7022 \cdot 10^{-7}$ | $1.2836 \cdot 10^{-3}$ | $6.0967 \cdot 10^0$    |
| 4750                  | $1.0492 \cdot 10^{-14}$ | $5.0095 \cdot 10^{-11}$ | $2.3921 \cdot 10^{-7}$ | $1.1422 \cdot 10^{-3}$ | $5.4540 \cdot 10^0$    |
| 4775                  | $9.1894 \cdot 10^{-15}$ | $4.4109 \cdot 10^{-11}$ | $2.1173 \cdot 10^{-7}$ | $1.0163 \cdot 10^{-3}$ | $4.8782 \cdot 10^0$    |
| 4800                  | $8.0537 \cdot 10^{-15}$ | $3.8859 \cdot 10^{-11}$ | $1.8750 \cdot 10^{-7}$ | $9.0467 \cdot 10^{-4}$ | $4.3650 \cdot 10^0$    |
| 4825                  | $7.0615 \cdot 10^{-15}$ | $3.4248 \cdot 10^{-11}$ | $1.6611 \cdot 10^{-7}$ | $8.0560 \cdot 10^{-4}$ | $3.9072 \cdot 10^0$    |
| 4850                  | $6.1951 \cdot 10^{-15}$ | $3.0202 \cdot 10^{-11}$ | $1.4724 \cdot 10^{-7}$ | $7.1775 \cdot 10^{-4}$ | $3.4991 \cdot 10^0$    |
| 4875                  | $5.4361 \cdot 10^{-15}$ | $2.6637 \cdot 10^{-11}$ | $1.3053 \cdot 10^{-7}$ | $6.3955 \cdot 10^{-4}$ | $3.1338 \cdot 10^0$    |
| 4900                  | $4.7721 \cdot 10^{-15}$ | $2.3503 \cdot 10^{-11}$ | $1.1575 \cdot 10^{-7}$ | $5.7006 \cdot 10^{-4}$ | $2.8076 \cdot 10^0$    |
| 4925                  | $4.1878 \cdot 10^{-15}$ | $2.0730 \cdot 10^{-11}$ | $1.0262 \cdot 10^{-7}$ | $5.0793 \cdot 10^{-4}$ | $2.5143 \cdot 10^0$    |
| 4950                  | $3.6731 \cdot 10^{-15}$ | $1.8274 \cdot 10^{-11}$ | $9.0911 \cdot 10^{-8}$ | $4.5228 \cdot 10^{-4}$ | $2.2501 \cdot 10^0$    |
| 4975                  | $3.2229 \cdot 10^{-15}$ | $1.6115 \cdot 10^{-11}$ | $8.0572 \cdot 10^{-8}$ | $4.0286 \cdot 10^{-4}$ | $2.0143 \cdot 10^0$    |
| 5000                  | $2.8715 \cdot 10^{-15}$ | $1.4645 \cdot 10^{-11}$ | $7.4687 \cdot 10^{-8}$ | $3.8091 \cdot 10^{-4}$ | $1.9426 \cdot 10^0$    |
| 5100                  | $1.7087 \cdot 10^{-15}$ | $8.8850 \cdot 10^{-12}$ | $4.6202 \cdot 10^{-8}$ | $2.4025 \cdot 10^{-4}$ | $1.2493 \cdot 10^0$    |
| 5200                  | $1.0185 \cdot 10^{-15}$ | $5.3981 \cdot 10^{-12}$ | $2.8610 \cdot 10^{-8}$ | $1.5164 \cdot 10^{-4}$ | $8.0365 \cdot 10^{-1}$ |
| 5300                  | $6.0977 \cdot 10^{-16}$ | $3.2928 \cdot 10^{-12}$ | $1.7781 \cdot 10^{-8}$ | $9.6016 \cdot 10^{-5}$ | $5.1849 \cdot 10^{-1}$ |
| 5400                  | $3.6472 \cdot 10^{-16}$ | $2.0060 \cdot 10^{-12}$ | $1.1033 \cdot 10^{-8}$ | $6.0680 \cdot 10^{-5}$ | $3.3374 \cdot 10^{-1}$ |
| 5500                  | $2.1916 \cdot 10^{-16}$ | $1.2273 \cdot 10^{-12}$ | $6.8727 \cdot 10^{-9}$ | $3.8488 \cdot 10^{-5}$ | $2.1553 \cdot 10^{-1}$ |
| 5600                  | $1.3218 \cdot 10^{-16}$ | $7.5337 \cdot 10^{-13}$ | $4.2943 \cdot 10^{-9}$ | $2.4477 \cdot 10^{-5}$ | $1.3952 \cdot 10^{-1}$ |
| 5700                  | $8.0079 \cdot 10^{-17}$ | $4.6446 \cdot 10^{-13}$ | $2.6939 \cdot 10^{-9}$ | $1.5625 \cdot 10^{-5}$ | $9.0621 \cdot 10^{-2}$ |

Continued on next page

Table 15 – continued from previous page

| $\log X_0 = \log X_1$ | $m_1 = M_1$             | $m_2 = M_2$             | $m_3 = M_3$             | $m_4 = M_4$             | $m_5 = M_5$             |
|-----------------------|-------------------------|-------------------------|-------------------------|-------------------------|-------------------------|
| 5800                  | $4.8519 \cdot 10^{-17}$ | $2.8626 \cdot 10^{-13}$ | $1.6890 \cdot 10^{-9}$  | $9.9647 \cdot 10^{-6}$  | $5.8792 \cdot 10^{-2}$  |
| 5900                  | $2.9483 \cdot 10^{-17}$ | $1.7690 \cdot 10^{-13}$ | $1.0614 \cdot 10^{-9}$  | $6.3682 \cdot 10^{-6}$  | $3.8209 \cdot 10^{-2}$  |
| 6000                  | $1.7952 \cdot 10^{-17}$ | $1.0951 \cdot 10^{-13}$ | $6.6798 \cdot 10^{-10}$ | $4.0747 \cdot 10^{-6}$  | $2.4856 \cdot 10^{-2}$  |
| 6100                  | $1.0988 \cdot 10^{-17}$ | $6.8120 \cdot 10^{-14}$ | $4.2235 \cdot 10^{-10}$ | $2.6186 \cdot 10^{-6}$  | $1.6235 \cdot 10^{-2}$  |
| 6200                  | $6.7178 \cdot 10^{-18}$ | $4.2322 \cdot 10^{-14}$ | $2.6663 \cdot 10^{-10}$ | $1.6798 \cdot 10^{-6}$  | $1.0583 \cdot 10^{-2}$  |
| 6300                  | $4.1268 \cdot 10^{-18}$ | $2.6412 \cdot 10^{-14}$ | $1.6904 \cdot 10^{-10}$ | $1.0818 \cdot 10^{-6}$  | $6.9236 \cdot 10^{-3}$  |
| 6400                  | $2.5481 \cdot 10^{-18}$ | $1.6563 \cdot 10^{-14}$ | $1.0766 \cdot 10^{-10}$ | $6.9977 \cdot 10^{-7}$  | $4.5485 \cdot 10^{-3}$  |
| 6500                  | $1.5741 \cdot 10^{-18}$ | $1.0389 \cdot 10^{-14}$ | $6.8566 \cdot 10^{-11}$ | $4.5254 \cdot 10^{-7}$  | $2.9868 \cdot 10^{-3}$  |
| 6600                  | $9.7287 \cdot 10^{-19}$ | $6.5182 \cdot 10^{-15}$ | $4.3672 \cdot 10^{-11}$ | $2.9261 \cdot 10^{-7}$  | $1.9605 \cdot 10^{-3}$  |
| 6700                  | $6.0447 \cdot 10^{-19}$ | $4.1104 \cdot 10^{-15}$ | $2.7951 \cdot 10^{-11}$ | $1.9007 \cdot 10^{-7}$  | $1.2925 \cdot 10^{-3}$  |
| 6800                  | $3.7652 \cdot 10^{-19}$ | $2.5980 \cdot 10^{-15}$ | $1.7926 \cdot 10^{-11}$ | $1.2369 \cdot 10^{-7}$  | $8.5345 \cdot 10^{-4}$  |
| 6900                  | $2.3555 \cdot 10^{-19}$ | $1.6488 \cdot 10^{-15}$ | $1.1542 \cdot 10^{-11}$ | $8.0791 \cdot 10^{-8}$  | $5.6554 \cdot 10^{-4}$  |
| 7000                  | $1.4744 \cdot 10^{-19}$ | $1.0468 \cdot 10^{-15}$ | $7.4322 \cdot 10^{-12}$ | $5.2769 \cdot 10^{-8}$  | $3.7466 \cdot 10^{-4}$  |
| 7100                  | $9.2826 \cdot 10^{-20}$ | $6.6835 \cdot 10^{-16}$ | $4.8121 \cdot 10^{-12}$ | $3.4647 \cdot 10^{-8}$  | $2.4946 \cdot 10^{-4}$  |
| 7200                  | $5.8601 \cdot 10^{-20}$ | $4.2779 \cdot 10^{-16}$ | $3.1229 \cdot 10^{-12}$ | $2.2797 \cdot 10^{-8}$  | $1.6642 \cdot 10^{-4}$  |
| 7300                  | $3.7014 \cdot 10^{-20}$ | $2.7391 \cdot 10^{-16}$ | $2.0269 \cdot 10^{-12}$ | $1.4999 \cdot 10^{-8}$  | $1.1100 \cdot 10^{-4}$  |
| 7400                  | $2.3489 \cdot 10^{-20}$ | $1.7617 \cdot 10^{-16}$ | $1.3213 \cdot 10^{-12}$ | $9.9092 \cdot 10^{-9}$  | $7.4319 \cdot 10^{-5}$  |
| 7500                  | $1.4908 \cdot 10^{-20}$ | $1.1330 \cdot 10^{-16}$ | $8.6105 \cdot 10^{-13}$ | $6.5440 \cdot 10^{-9}$  | $4.9735 \cdot 10^{-5}$  |
| 7600                  | $9.4822 \cdot 10^{-21}$ | $7.3013 \cdot 10^{-17}$ | $5.6220 \cdot 10^{-13}$ | $4.3290 \cdot 10^{-9}$  | $3.3333 \cdot 10^{-5}$  |
| 7700                  | $6.0570 \cdot 10^{-21}$ | $4.7245 \cdot 10^{-17}$ | $3.6851 \cdot 10^{-13}$ | $2.8744 \cdot 10^{-9}$  | $2.2420 \cdot 10^{-5}$  |
| 7800                  | $3.8812 \cdot 10^{-21}$ | $3.0661 \cdot 10^{-17}$ | $2.4223 \cdot 10^{-13}$ | $1.9136 \cdot 10^{-9}$  | $1.5117 \cdot 10^{-5}$  |
| 7900                  | $2.4928 \cdot 10^{-21}$ | $1.9943 \cdot 10^{-17}$ | $1.5954 \cdot 10^{-13}$ | $1.2764 \cdot 10^{-9}$  | $1.0211 \cdot 10^{-5}$  |
| 8000                  | $1.6007 \cdot 10^{-21}$ | $1.2966 \cdot 10^{-17}$ | $1.0502 \cdot 10^{-13}$ | $8.5065 \cdot 10^{-10}$ | $6.8903 \cdot 10^{-6}$  |
| 8100                  | $1.0327 \cdot 10^{-21}$ | $8.4675 \cdot 10^{-18}$ | $6.9433 \cdot 10^{-14}$ | $5.6935 \cdot 10^{-10}$ | $4.6687 \cdot 10^{-6}$  |
| 8200                  | $6.6829 \cdot 10^{-22}$ | $5.5468 \cdot 10^{-18}$ | $4.6038 \cdot 10^{-14}$ | $3.8212 \cdot 10^{-10}$ | $3.1716 \cdot 10^{-6}$  |
| 8300                  | $4.3257 \cdot 10^{-22}$ | $3.6336 \cdot 10^{-18}$ | $3.0523 \cdot 10^{-14}$ | $2.5639 \cdot 10^{-10}$ | $2.1537 \cdot 10^{-6}$  |
| 8400                  | $2.8105 \cdot 10^{-22}$ | $2.3889 \cdot 10^{-18}$ | $2.0306 \cdot 10^{-14}$ | $1.7260 \cdot 10^{-10}$ | $1.4671 \cdot 10^{-6}$  |
| 8500                  | $1.8316 \cdot 10^{-22}$ | $1.5752 \cdot 10^{-18}$ | $1.3547 \cdot 10^{-14}$ | $1.1650 \cdot 10^{-10}$ | $1.0019 \cdot 10^{-6}$  |
| 8600                  | $1.1981 \cdot 10^{-22}$ | $1.0424 \cdot 10^{-18}$ | $9.0682 \cdot 10^{-15}$ | $7.8894 \cdot 10^{-11}$ | $6.8638 \cdot 10^{-7}$  |
| 8700                  | $7.8221 \cdot 10^{-23}$ | $6.8834 \cdot 10^{-19}$ | $6.0574 \cdot 10^{-15}$ | $5.3305 \cdot 10^{-11}$ | $4.6909 \cdot 10^{-7}$  |
| 8800                  | $5.1585 \cdot 10^{-23}$ | $4.5911 \cdot 10^{-19}$ | $4.0861 \cdot 10^{-15}$ | $3.6366 \cdot 10^{-11}$ | $3.6366 \cdot 10^{-7}$  |
| 8900                  | $3.3883 \cdot 10^{-23}$ | $3.0495 \cdot 10^{-19}$ | $2.7445 \cdot 10^{-15}$ | $2.4701 \cdot 10^{-11}$ | $2.2231 \cdot 10^{-7}$  |
| 9000                  | $2.2253 \cdot 10^{-23}$ | $2.0250 \cdot 10^{-19}$ | $1.8428 \cdot 10^{-15}$ | $1.6769 \cdot 10^{-11}$ | $1.5260 \cdot 10^{-7}$  |
| 9100                  | $1.4642 \cdot 10^{-23}$ | $1.3470 \cdot 10^{-19}$ | $1.2393 \cdot 10^{-15}$ | $1.1401 \cdot 10^{-11}$ | $1.0489 \cdot 10^{-7}$  |
| 9200                  | $9.6778 \cdot 10^{-24}$ | $9.0003 \cdot 10^{-20}$ | $8.3703 \cdot 10^{-16}$ | $7.7844 \cdot 10^{-12}$ | $7.2395 \cdot 10^{-8}$  |
| 9300                  | $6.4195 \cdot 10^{-24}$ | $6.0344 \cdot 10^{-20}$ | $5.6723 \cdot 10^{-16}$ | $5.3320 \cdot 10^{-12}$ | $5.0121 \cdot 10^{-8}$  |
| 9400                  | $4.2972 \cdot 10^{-24}$ | $4.0823 \cdot 10^{-20}$ | $3.8782 \cdot 10^{-16}$ | $3.6843 \cdot 10^{-12}$ | $3.5001 \cdot 10^{-8}$  |
| 9500                  | $2.8513 \cdot 10^{-24}$ | $2.7372 \cdot 10^{-20}$ | $2.6277 \cdot 10^{-16}$ | $2.5226 \cdot 10^{-12}$ | $2.4217 \cdot 10^{-8}$  |
| 9600                  | $1.9059 \cdot 10^{-24}$ | $1.8487 \cdot 10^{-20}$ | $1.7933 \cdot 10^{-16}$ | $1.7395 \cdot 10^{-12}$ | $1.6873 \cdot 10^{-8}$  |
| 9700                  | $1.2689 \cdot 10^{-24}$ | $1.2436 \cdot 10^{-20}$ | $1.2187 \cdot 10^{-16}$ | $1.1943 \cdot 10^{-12}$ | $1.1704 \cdot 10^{-8}$  |
| 9800                  | $8.4841 \cdot 10^{-25}$ | $8.3993 \cdot 10^{-21}$ | $8.3153 \cdot 10^{-17}$ | $8.2321 \cdot 10^{-13}$ | $8.1498 \cdot 10^{-9}$  |
| 9900                  | $5.7396 \cdot 10^{-25}$ | $5.7396 \cdot 10^{-21}$ | $5.7396 \cdot 10^{-17}$ | $5.7396 \cdot 10^{-13}$ | $5.7396 \cdot 10^{-9}$  |
| 10000                 | $3.8228 \cdot 10^{-25}$ | $3.8610 \cdot 10^{-21}$ | $3.8997 \cdot 10^{-17}$ | $3.9387 \cdot 10^{-13}$ | $3.9780 \cdot 10^{-9}$  |
| 10100                 | $2.5746 \cdot 10^{-25}$ | $2.6260 \cdot 10^{-21}$ | $2.6786 \cdot 10^{-17}$ | $2.7321 \cdot 10^{-13}$ | $2.7868 \cdot 10^{-9}$  |
| 10200                 | $1.7389 \cdot 10^{-25}$ | $1.7911 \cdot 10^{-21}$ | $1.8448 \cdot 10^{-17}$ | $1.9002 \cdot 10^{-13}$ | $1.9572 \cdot 10^{-9}$  |
| 10300                 | $1.1734 \cdot 10^{-25}$ | $1.2204 \cdot 10^{-21}$ | $1.2692 \cdot 10^{-17}$ | $1.3199 \cdot 10^{-13}$ | $1.3727 \cdot 10^{-9}$  |
| 10400                 | $7.9556 \cdot 10^{-26}$ | $8.3534 \cdot 10^{-22}$ | $8.7711 \cdot 10^{-18}$ | $9.2096 \cdot 10^{-14}$ | $9.6701 \cdot 10^{-10}$ |
| 10500                 | $5.4077 \cdot 10^{-26}$ | $5.7321 \cdot 10^{-22}$ | $6.0761 \cdot 10^{-18}$ | $6.4406 \cdot 10^{-14}$ | $6.8270 \cdot 10^{-10}$ |
| 10600                 | $3.6845 \cdot 10^{-26}$ | $3.9424 \cdot 10^{-22}$ | $4.2184 \cdot 10^{-18}$ | $4.5137 \cdot 10^{-14}$ | $4.8296 \cdot 10^{-10}$ |
| 10700                 | $2.5150 \cdot 10^{-26}$ | $2.7162 \cdot 10^{-22}$ | $2.9335 \cdot 10^{-18}$ | $3.1682 \cdot 10^{-14}$ | $3.4217 \cdot 10^{-10}$ |
| 10800                 | $1.7201 \cdot 10^{-26}$ | $1.8749 \cdot 10^{-22}$ | $2.0437 \cdot 10^{-18}$ | $2.2276 \cdot 10^{-14}$ | $2.4281 \cdot 10^{-10}$ |
| 10900                 | $1.1640 \cdot 10^{-26}$ | $1.2803 \cdot 10^{-22}$ | $1.4084 \cdot 10^{-18}$ | $1.5492 \cdot 10^{-14}$ | $1.7041 \cdot 10^{-10}$ |
| 11000                 | $7.9284 \cdot 10^{-27}$ | $8.8005 \cdot 10^{-23}$ | $9.7685 \cdot 10^{-19}$ | $1.0844 \cdot 10^{-14}$ | $1.2036 \cdot 10^{-10}$ |
| 11100                 | $5.4156 \cdot 10^{-27}$ | $6.0655 \cdot 10^{-23}$ | $6.7933 \cdot 10^{-19}$ | $7.6085 \cdot 10^{-15}$ | $8.5215 \cdot 10^{-11}$ |
| 11200                 | $3.7120 \cdot 10^{-27}$ | $4.1946 \cdot 10^{-23}$ | $4.7398 \cdot 10^{-19}$ | $5.3560 \cdot 10^{-15}$ | $6.0523 \cdot 10^{-11}$ |

Continued on next page

Table 15 – continued from previous page

| $\log X_0 = \log X_1$ | $m_1 = M_1$             | $m_2 = M_2$             | $m_3 = M_3$             | $m_4 = M_4$             | $m_5 = M_5$             |
|-----------------------|-------------------------|-------------------------|-------------------------|-------------------------|-------------------------|
| 11300                 | $2.5509 \cdot 10^{-27}$ | $2.9080 \cdot 10^{-23}$ | $3.3152 \cdot 10^{-19}$ | $3.7793 \cdot 10^{-15}$ | $4.3084 \cdot 10^{-11}$ |
| 11400                 | $1.7570 \cdot 10^{-27}$ | $2.0205 \cdot 10^{-23}$ | $2.3236 \cdot 10^{-19}$ | $2.6721 \cdot 10^{-15}$ | $3.0729 \cdot 10^{-11}$ |
| 11500                 | $1.2103 \cdot 10^{-27}$ | $1.4039 \cdot 10^{-23}$ | $1.6285 \cdot 10^{-19}$ | $1.8891 \cdot 10^{-15}$ | $2.1913 \cdot 10^{-11}$ |
| 11600                 | $8.3445 \cdot 10^{-28}$ | $9.7630 \cdot 10^{-24}$ | $1.1423 \cdot 10^{-19}$ | $1.3365 \cdot 10^{-15}$ | $1.5637 \cdot 10^{-11}$ |
| 11700                 | $5.7692 \cdot 10^{-28}$ | $6.8076 \cdot 10^{-24}$ | $8.0330 \cdot 10^{-20}$ | $9.4789 \cdot 10^{-16}$ | $1.1186 \cdot 10^{-11}$ |
| 11800                 | $3.9987 \cdot 10^{-28}$ | $4.7584 \cdot 10^{-24}$ | $5.6625 \cdot 10^{-20}$ | $6.7384 \cdot 10^{-16}$ | $8.0187 \cdot 10^{-12}$ |
| 11900                 | $2.7776 \cdot 10^{-28}$ | $3.3331 \cdot 10^{-24}$ | $3.9997 \cdot 10^{-20}$ | $4.7996 \cdot 10^{-16}$ | $5.7596 \cdot 10^{-12}$ |
| 12000                 | $1.9331 \cdot 10^{-28}$ | $2.3390 \cdot 10^{-24}$ | $2.8302 \cdot 10^{-20}$ | $3.4245 \cdot 10^{-16}$ | $4.1437 \cdot 10^{-12}$ |
| 12100                 | $1.3478 \cdot 10^{-28}$ | $1.6443 \cdot 10^{-24}$ | $2.0060 \cdot 10^{-20}$ | $2.4473 \cdot 10^{-16}$ | $2.9857 \cdot 10^{-12}$ |
| 12200                 | $9.3147 \cdot 10^{-29}$ | $1.1457 \cdot 10^{-24}$ | $1.4093 \cdot 10^{-20}$ | $1.7334 \cdot 10^{-16}$ | $2.1320 \cdot 10^{-12}$ |
| 12300                 | $6.5069 \cdot 10^{-29}$ | $8.0686 \cdot 10^{-25}$ | $1.0005 \cdot 10^{-20}$ | $1.2407 \cdot 10^{-16}$ | $1.5384 \cdot 10^{-12}$ |
| 12400                 | $4.5540 \cdot 10^{-29}$ | $5.6924 \cdot 10^{-25}$ | $7.1155 \cdot 10^{-21}$ | $8.8944 \cdot 10^{-17}$ | $1.1118 \cdot 10^{-12}$ |
| 12500                 | $3.1924 \cdot 10^{-29}$ | $4.0224 \cdot 10^{-25}$ | $5.0682 \cdot 10^{-21}$ | $6.3860 \cdot 10^{-17}$ | $8.0463 \cdot 10^{-13}$ |
| 12600                 | $2.2307 \cdot 10^{-29}$ | $2.8330 \cdot 10^{-25}$ | $3.5979 \cdot 10^{-21}$ | $4.5694 \cdot 10^{-17}$ | $5.8031 \cdot 10^{-13}$ |
| 12700                 | $1.5600 \cdot 10^{-29}$ | $1.9967 \cdot 10^{-25}$ | $2.5558 \cdot 10^{-21}$ | $3.2714 \cdot 10^{-17}$ | $4.1874 \cdot 10^{-13}$ |
| 12800                 | $1.0940 \cdot 10^{-29}$ | $1.4112 \cdot 10^{-25}$ | $1.8205 \cdot 10^{-21}$ | $2.3484 \cdot 10^{-17}$ | $3.0294 \cdot 10^{-13}$ |
| 12900                 | $7.6900 \cdot 10^{-30}$ | $9.9970 \cdot 10^{-26}$ | $1.2996 \cdot 10^{-21}$ | $1.6895 \cdot 10^{-17}$ | $2.1964 \cdot 10^{-13}$ |
| 13000                 | $5.5830 \cdot 10^{-30}$ | $7.5371 \cdot 10^{-26}$ | $1.0175 \cdot 10^{-21}$ | $1.3737 \cdot 10^{-17}$ | $1.8544 \cdot 10^{-13}$ |
| 13500                 | $9.9578 \cdot 10^{-31}$ | $1.3743 \cdot 10^{-26}$ | $1.8966 \cdot 10^{-22}$ | $2.6174 \cdot 10^{-18}$ | $3.6123 \cdot 10^{-14}$ |
| 13800                 | $3.5593 \cdot 10^{-31}$ | $4.9830 \cdot 10^{-27}$ | $6.9761 \cdot 10^{-23}$ | $9.7665 \cdot 10^{-19}$ | $1.3674 \cdot 10^{-14}$ |
| 14000                 | $1.8399 \cdot 10^{-31}$ | $2.7598 \cdot 10^{-27}$ | $4.1396 \cdot 10^{-23}$ | $6.2094 \cdot 10^{-19}$ | $9.3141 \cdot 10^{-15}$ |
| 15000                 | $6.5712 \cdot 10^{-33}$ | $1.0514 \cdot 10^{-28}$ | $1.6823 \cdot 10^{-24}$ | $2.6916 \cdot 10^{-20}$ | $4.3065 \cdot 10^{-16}$ |
| 16000                 | $2.5739 \cdot 10^{-34}$ | $4.3756 \cdot 10^{-30}$ | $7.4384 \cdot 10^{-26}$ | $1.2646 \cdot 10^{-21}$ | $2.1497 \cdot 10^{-17}$ |
| 17000                 | $1.1168 \cdot 10^{-35}$ | $2.0101 \cdot 10^{-31}$ | $3.6182 \cdot 10^{-27}$ | $6.5127 \cdot 10^{-23}$ | $1.1723 \cdot 10^{-18}$ |
| 18000                 | $5.3739 \cdot 10^{-37}$ | $1.0211 \cdot 10^{-32}$ | $1.9400 \cdot 10^{-28}$ | $3.6860 \cdot 10^{-24}$ | $7.0033 \cdot 10^{-20}$ |
| 19000                 | $2.7357 \cdot 10^{-38}$ | $5.4714 \cdot 10^{-34}$ | $1.0943 \cdot 10^{-29}$ | $2.1886 \cdot 10^{-25}$ | $4.3772 \cdot 10^{-21}$ |
| 20000                 | $1.5041 \cdot 10^{-39}$ | $3.1585 \cdot 10^{-35}$ | $6.6329 \cdot 10^{-31}$ | $1.3929 \cdot 10^{-26}$ | $2.9251 \cdot 10^{-22}$ |
| 21000                 | $9.0606 \cdot 10^{-41}$ | $1.9934 \cdot 10^{-36}$ | $4.3853 \cdot 10^{-32}$ | $9.6477 \cdot 10^{-28}$ | $2.1225 \cdot 10^{-23}$ |
| 22000                 | $5.6101 \cdot 10^{-42}$ | $1.2904 \cdot 10^{-37}$ | $2.9678 \cdot 10^{-33}$ | $6.8258 \cdot 10^{-29}$ | $1.5700 \cdot 10^{-24}$ |
| 23000                 | $3.7554 \cdot 10^{-43}$ | $9.0129 \cdot 10^{-39}$ | $2.1631 \cdot 10^{-34}$ | $5.1915 \cdot 10^{-30}$ | $1.2460 \cdot 10^{-25}$ |
| 24000                 | $2.6756 \cdot 10^{-44}$ | $6.6889 \cdot 10^{-40}$ | $1.6723 \cdot 10^{-35}$ | $4.1806 \cdot 10^{-31}$ | $1.0452 \cdot 10^{-26}$ |
| 25000                 | $7.5635 \cdot 10^{-45}$ | $1.8909 \cdot 10^{-40}$ | $4.7272 \cdot 10^{-36}$ | $1.1818 \cdot 10^{-31}$ | $2.9545 \cdot 10^{-27}$ |

*Acknowledgements.* This research was supported by NSERC Discovery grants of Habiba Kadiri and Nathan Ng and the University of Lethbridge startup grant of Andrew Fiori. These grants also supported Joshua Swidinsky’s research assistantship. Samuel Broadbent and Kirsten Wilk were supported by NSERC USRA grants in Summer 2017 and 2018 and Allysa Lumley was supported by a York University graduate fellowship. Thank-you to the PIMS postdoctoral fellows Alia Hamieh (2015-2017) and Peng-Jie Wong (2017-2019) for helping with the supervision of Samuel Broadbent and Kirsten Wilk during part of this project.

## REFERENCES

- [1] S. BROADBENT, H. KADIRI, A. LUMLEY, N. NG, K. WILK, *Sharper bounds for the Chebyshev function  $\theta(x)$* , submitted.
- [2] J. BÜTHE, *Estimating  $\pi(x)$  and related functions under partial RH assumptions*, Math. Comp. 85 (2016), no. 301, 2483–2498.
- [3] J. BÜTHE, *An analytic method for bounding  $\psi(x)$* , Math. Comp. 87 (2018), no. 312, 1991–2009.
- [4] P. DUSART, *Estimates of some functions over primes without R.H.*, arXiv:1002.0442 (February 2, 2010).
- [5] P. DUSART, *Estimates of  $\psi, \theta$  for large values of  $x$  without the Riemann Hypothesis*, Math. Comp. 85 (2016), no. 298, 875–888.
- [6] L. FABER AND H. KADIRI, *New bounds for  $\psi(x)$* , Math. Comp. 84 (2015), no. 293, 1339–1357.
- [7] D. Platt and T. Trudgian, *The error term in the prime number theorem*, Math. Comp. 90 (2021), 871–881.



- [8] J.B. ROSSER, *Explicit bounds for some functions of prime numbers*, Amer. J. Math. 63 (1941), 211–232.
- [9] J.B. ROSSER AND L. SCHOENFELD, *Approximate formulas for some functions of prime numbers*, Illinois. J. Math. 6 (1962), 64–94.
- [10] J.B. ROSSER AND L. SCHOENFELD, *Sharper bounds for Chebyshev functions  $\theta(x)$  and  $\psi(x)$*  I, Math. Comp. 29 (1975), 243–269.
- [11] S. WEDENIWSKI - ZETAGRID, *Computational verification of the Riemann hypothesis*, Conference in Number Theory in Honour of Professor H.C. Williams, Alberta, Canada, May 2003.  
<https://github.com/Wedeniowski/ZetaGrid>

UNIVERSITY OF LETHBRIDGE, DEPARTMENT OF MATHEMATICS AND COMPUTER SCIENCE, 4401 UNIVERSITY DRIVE, LETHBRIDGE, AB T1K 3M4, CANADA

*E-mail address:* `sam.broadbent@uleth.ca`

*E-mail address:* `andrew.fiori@uleth.ca`

*E-mail address:* `habiba.kadiri@uleth.ca`

*E-mail address:* `lumley@crm.umontreal.ca`

*E-mail address:* `nathan.ng@uleth.ca`

*E-mail address:* `joshua.swidinsky@uleth.ca`

*E-mail address:* `kirsten.wilk@uleth.ca`
